# Supplementary material for: Electron-Phonon Coupling in Many-Body Perturbation Theory: Developments within the Quasiparticle Self-Consistent GW approximation and LMTO Formalism
Source: arXiv:2404.02902 source file (2025-03-13)
Supplement: Supplementary file 1 [file qsgw-eph__supplement.pdf]

# Supplementary materials: Electron–Phonon Coupling in Many-Body Perturbation Theory: Developments within the Quasiparticle Self-Consistent GW approximation and LMTO Formalism

Savio Laricchia,[1,2] Casey Eichstaedt,[3] Dimitar Pashov,[2] and Mark van Schilfgaarde[3]

[1] *Centro S3, CNR–Istituto Nanoscienze, 41125 Modena, Italy**

[2] *Department of Physics, King's College London, Strand, London WC2R 2LS, United Kingdom*

[3] *National Renewable Energy Laboratory, Golden, CO 80401,USA*

## CONTENTS

S.1. Technical details for computing the reduced *e-ph* matrix element 1
- A. Reduced *e-ph* matrix element integral evaluated in the interstitial region 1
  - 1. Case $\boldsymbol{\tau}_i - \boldsymbol{\tau}_r - \mathbf{R}_p \neq 0$ 2
  - 2. Case $\boldsymbol{\tau}_i - \boldsymbol{\tau}_r - \mathbf{R}_p = 0$ 4
- B. Reduced *e-ph* matrix element integral evaluated in the augmentation region 5
  - 1. Case $\boldsymbol{\tau}_i - \boldsymbol{\tau}_r - \mathbf{R}_p \neq 0$ 5
  - 2. Case $\boldsymbol{\tau}_i - \boldsymbol{\tau}_r - \mathbf{R}_p = 0$ 6
- C. Integral (S.1) evaluated in the interstitial region 6
- D. Integral (S.1) evaluated in the augmentation region 7

S.2. Rotation of the electron-phonon coupling matrix on the full BZ for the electron and phonon wave vectors 7

S.3. Transformation rules for the coefficients $G^{\mathbf{q}}_{I\nu}$ under rotation of the phonon wave vectors 10
  - 1. Transformation rules in the interstitial region 12
  - 2. Transformation rules in the augmentation region 12

S.4. Spherical functions 12
- A. Spherical Bessel and Hankel functions: definitions and conventions 12
  - 1. Derivatives and some recursion relations 14
  - 2. Integrals of Lommel's type for spherical functions 14
- B. Gaunt and Clebsch-Gordan coefficients 16
- C. Analytical evaluation of the gradient of a spherical function by means of real vector spherical harmonics 18
  - 1. Analytical expression for $\mathbf{Y}_{lm_l} = \widehat{\mathbf{r}} Y_{lm_l}$ 19
  - 2. Analytical expression for $\boldsymbol{\Psi}_{lm_l} = r\nabla_{\mathbf{r}} Y_{lm_l}$ 20
  - 3. Final expression for $\nabla_{\mathbf{r}} f_l(r) Y_{lm_l}(\widehat{\mathbf{r}})$ 22

S.5. Acoustic sum rule on density derivatives and Pulay-like corrections 24

S.6. *e-ph* matrix elements for acoustic phonon modes in the long wavelength limit 27
- A. Diagonal components of the *e-ph* matrix 29
- B. Off-diagonal components of the *e-ph* matrix 30
- C. Results within the field-theoretic approach: application to diamond 31

S.7. On the derivation of the nuclear contribution to the adiabatic phonon self-energy $\Pi^{\mathrm{A},i}_{r\alpha l,s\beta l'}$ 31

References 33

* Current affiliation: Istituto di Struttura della Materia-CNR (ISM-CNR), Area della Ricerca di Roma 1, Monterotondo Scalo, Italy; corresponding author: savio.laricchia@mlib.ism.cnr.it

## S.1. TECHNICAL DETAILS FOR COMPUTING THE REDUCED *E-PH* MATRIX ELEMENT

The most challenging aspect of implementing the reduced *e-ph* matrix elements (Eq. 158) involves calculating the integral

$$\int_{\Omega_0} d\mathbf{r} M^{\mathbf{q}\,*}_I(\mathbf{r}) \frac{\partial \widetilde{V}^{(0)\,\mathbf{q}}_r(\mathbf{r})}{\partial r_\alpha} = \int_{\Omega_0} d\mathbf{r} M^{\mathbf{q}\,*}_I(\mathbf{r}) \frac{\partial V^{(0)\,\mathbf{q}}_r(\mathbf{r})}{\partial r_\alpha} + \\ + \int_{\Omega_0} d\mathbf{r} M^{\mathbf{q}\,*}_I(\mathbf{r}) \frac{\partial V^{c\,\mathbf{q}}_r(\mathbf{r})}{\partial r_\alpha}\,. \tag{S.1}$$

In sections S.1 A and S.1 B, we provide a comprehensive approach to solving the integral

$$\int_{\Omega_0} d\mathbf{r} M^{\mathbf{q}\,*}_I(\mathbf{r}) \frac{\partial V^{(0)\,\mathbf{q}}_r(\mathbf{r})}{\partial r_\alpha} \tag{S.2}$$

within both the interstitial and augmentation regions for arbitrary wave vectors. The integral involving the Bloch-summed screening core potential $V^{c\,\mathbf{q}}_r(\mathbf{r})$,

$$\int_{\Omega_0} d\mathbf{r} M^{\mathbf{q}\,*}_I(\mathbf{r}) \frac{\partial V^{c\,\mathbf{q}}_r(\mathbf{r})}{\partial r_\alpha}\,, \tag{S.3}$$

is discussed in sections S.1 C and S.1 D.

### A. Reduced *e-ph* matrix element integral evaluated in the interstitial region

Combining Eq. (S.2) with the definitions from Eqs. (89)-(90) for the plane waves inside the interstitial region,

we compute this quantity over all space and subtract out its projection inside the atomic spheres, so the interstitial contribution is

$$\int_{\Omega_0} d\mathbf{r} P^{\mathbf{q}\,*}_{\mathbf{G}}(\mathbf{r}) \frac{\partial V_r^{(0)\,\mathbf{q}}(\mathbf{r})}{\partial r_\alpha} = \frac{1}{\sqrt{\Omega_0}} \int_{\Omega_0} d\mathbf{r}\, e^{-i(\mathbf{q}+\mathbf{G})\cdot\mathbf{x}} \frac{\partial V_r^{(0)\mathbf{q}}(\mathbf{r})}{\partial r_\alpha} - \\ - \frac{1}{\sqrt{\Omega_0}} \sum_i \sum_p \sum_{lm} \int_{\Omega_0} d\mathbf{r}\, \frac{\partial V_r^{(0)\mathbf{q}}(\mathbf{r})}{\partial r_\alpha} \left[ P^{\mathbf{q}+\mathbf{G}}_{\boldsymbol{\tau}_i+\mathbf{R}_p lm}(\mathbf{r}) \theta(s_i - |\mathbf{r}-\boldsymbol{\tau}_i-\mathbf{R}_p|) \right]^* . \tag{S.4}$$

The first integral in Eq. (S.4) is straightforward and can be solved by using the inverse Bloch sum of $V_r^{(0)\mathbf{q}}(\mathbf{r})$—obtained by inverting Eq. (107)—with a subsequent inverse Fourier transform of a Yukawa nuclear potential

$$V_{rl}^{(0)}(\mathbf{r}) = \lim_{\kappa\to 0} -\frac{4\pi Z_r}{N_\mathbf{k}\Omega_0} \sum_{\mathbf{k}\in\mathrm{BZ}} \sum_{\mathbf{G}'} \frac{e^{-i(\mathbf{k}+\mathbf{G}')\cdot(\boldsymbol{\tau}_r-\mathbf{r})} e^{-i\mathbf{k}\cdot\mathbf{R}_l}}{|\mathbf{k}+\mathbf{G}'|^2+\kappa^2}, \tag{S.5}$$

to help with divergences in the long-wavelength limit. Here, $\kappa$ is positive and defined as $(i\kappa)^2 = -\kappa^2 \equiv \varepsilon$, with $\varepsilon$ an energy parameter. Combining the inverse Bloch sum of Eq. (107) with the first integral in Eq. (S.4) and Eq. (S.5) yields

$$\frac{1}{\sqrt{\Omega_0}} \int_{\Omega_0} d\mathbf{r}\, e^{-i(\mathbf{q}+\mathbf{G})\cdot\mathbf{r}} \frac{\partial V_r^{(0)\mathbf{q}}(\mathbf{r})}{\partial r_\alpha} = \\ = -\frac{i}{\sqrt{\Omega_0}} \lim_{\kappa\to 0} \frac{4\pi Z_r (\mathbf{q}+\mathbf{G})_\alpha}{|\mathbf{k}+\mathbf{G}'|^2+\kappa^2} e^{i(\mathbf{q}+\mathbf{G})\cdot\boldsymbol{\tau}_r} \tag{S.6}$$

In contrast, computing the second integral in Eq. (S.4) is more complicated and requires a more detailed analysis. The spherical expansion $\sum_{lm} P^{\mathbf{q}+\mathbf{G}}_{\boldsymbol{\tau}_i lm}$ of the plane wave $\exp[i(\mathbf{q}+\mathbf{G})\cdot\mathbf{r}]$ inside the $i$-th augmentation sphere, with plane wave components defined by Eq. (90) is exact in the limit $l\to\infty$. Consequently, the second integral in Eq. (S.4) can be performed by integrating solely within the $i$-th augmentation sphere since $\sum_{lm} P^{\mathbf{q}+\mathbf{G}}_{\boldsymbol{\tau}_i lm}$ vanishes outside it, as dictated by the Heaviside step function $\theta(s_i - |\mathbf{r}-\boldsymbol{\tau}_i-\mathbf{R}_p|)$. This integral thus simplifes to

$$-\frac{Z_r}{N_\mathbf{k}\sqrt{\Omega_0}} \sum_{ijp} \sum_{lm} e^{i\mathbf{q}\cdot\mathbf{R}_j} \times \\ \times \int_{\Omega_i} d\mathbf{r}' \left[ \frac{\partial}{\partial r'_\alpha} v(\mathbf{r}'-\mathbf{R}_j+\mathbf{R}_p+\boldsymbol{\tau}_i-\boldsymbol{\tau}_r) \right] P^{\mathbf{q}+\mathbf{G}\,*}_{\boldsymbol{\tau}_i+\mathbf{R}_p lm}(\mathbf{r}'), \tag{S.7}$$

where we applied the change of variable $\mathbf{r}' = \mathbf{r}+\boldsymbol{\tau}_i+\mathbf{R}_p$. Using the relationship $P^{\mathbf{q}+\mathbf{G}}_{\boldsymbol{\tau}_i+\mathbf{R}_p lm}(\mathbf{r}) = e^{i\mathbf{q}\cdot\mathbf{R}_p} P^{\mathbf{q}+\mathbf{G}}_{\boldsymbol{\tau}_i lm}(\mathbf{r})$ and introducing the combined lattice vectors $\mathbf{R}_{p'} = \mathbf{R}_j - \mathbf{R}_p$, this integral becomes

$$-\frac{Z_r}{\sqrt{\Omega_0}} \sum_{ip'} \sum_{lm} e^{i\mathbf{q}\cdot\mathbf{R}_{p'}} \times \\ \times \int_{\Omega_i} d\mathbf{r} \left[ \frac{\partial}{\partial r_\alpha} v(\mathbf{r}-\mathbf{R}_{p'}+\boldsymbol{\tau}_i-\boldsymbol{\tau}_r) \right] P^{\mathbf{q}+\mathbf{G}\,*}_{\boldsymbol{\tau}_i lm}(\mathbf{r}). \tag{S.8}$$

To facilitate the analysis, we introduce a second vector position localized within the $i$-th augmentation sphere by means of a Dirac delta function

$$-\lim_{\kappa\to 0} \frac{Z_r}{\sqrt{\Omega_0}} \sum_{ip} \sum_{lm} e^{i\mathbf{q}\cdot\mathbf{R}_p} \int_{\Omega_i}\int_{\Omega_i} d\mathbf{r} d\mathbf{r}' P^{\mathbf{q}+\mathbf{G}\,*}_{\boldsymbol{\tau}_i lm}(\mathbf{r}) \delta(\mathbf{r}') \\ \times \left( \nabla_\mathbf{r} \frac{e^{-\kappa|\mathbf{r}-\mathbf{r}'+\boldsymbol{\tau}_i-\boldsymbol{\tau}_r-\mathbf{R}_p|}}{|\mathbf{r}-\mathbf{r}'+\boldsymbol{\tau}_i-\boldsymbol{\tau}_r-\mathbf{R}_p|} \right)_\alpha . \tag{S.9}$$

Similar to the fully plane wave contribution, in Eq. (S.9), the electron-nuclear interaction kernel has been replaced with a generalized Yukawa-like potential, taking the $\kappa\to 0$ limit as described in Eq. (S.5). The inclusion of a non-zero energy parameter allows us to rewrite the generalized Coulomb kernel in terms of spherical Bessel $j_l^m(\kappa r)$ and Hankel $h_l^m(\kappa r)$ functions within the Methfessel convention [1] through the expansion

$$\frac{e^{-\kappa|\mathbf{r}-\mathbf{r}'|}}{|\mathbf{r}-\mathbf{r}'|} = 4\pi \sum_{lm} j_l^m(\kappa r_<) h_l^m(\kappa r_>) Y_{lm}(\widehat{\mathbf{r}}) Y_{lm}(\widehat{\mathbf{r}}'). \tag{S.10}$$

Further details about these special functions and the convention used throughout the text are provided in Sec. S.4 A. In Eq. (S.10), $Y_{lm}(\widehat{\mathbf{r}})$ denotes real spherical harmonics, which are discussed in greater detail in Sec. S.4 C. When summing over the index $i$, two cases arise:

1. $\boldsymbol{\tau}_i - \boldsymbol{\tau}_r - \mathbf{R}_p \neq 0$: this represents either two distinct atomic positions within the same primitive unit cell ($\mathbf{R}_p = 0$) or atoms in different unit cells ($\mathbf{R}_p \neq 0$);

2. $\boldsymbol{\tau}_i - \boldsymbol{\tau}_r - \mathbf{R}_p = 0$: this corresponds to the same atomic position in a given primitive unit cell (i.e., $\mathbf{R}_p = 0$).

### 1. Case $\boldsymbol{\tau}_i - \boldsymbol{\tau}_r - \mathbf{R}_p \neq 0$

The case $\boldsymbol{\tau}_i - \boldsymbol{\tau}_r - \mathbf{R}_p \neq 0$ is possible if either $\boldsymbol{\tau}_i = \boldsymbol{\tau}_r$; $\mathbf{R}_p \neq 0$ or $\boldsymbol{\tau}_i \neq \boldsymbol{\tau}_r$; $\forall \mathbf{R}_p$. If this condition holds, it can be shown that $r < |\mathbf{r}' + \boldsymbol{\tau}_r - \boldsymbol{\tau}_i + \mathbf{R}_p|$. To demonstrate this relation, consider that both the position vectors $\mathbf{r}$ and $\mathbf{r}'$ are defined in the sphere centered at $\boldsymbol{\tau}_i$ and $\Delta\boldsymbol{\tau} = \boldsymbol{\tau}_r - \boldsymbol{\tau}_i$ is the vector between the spheres centered at $\boldsymbol{\tau}_r$ (which generates the bare nuclear potential $V_r^{(0)}$) and $\boldsymbol{\tau}_i$ (where the potential $V_r^{(0)}$ is felt). In the case of $\mathbf{R}_p = \mathbf{0}$, it is evident that the vector $\mathbf{r}' + \Delta\boldsymbol{\tau}$ has a modulus greater than the radius of the $i$-th augmentation sphere and, consequently, greater than $|\mathbf{r}|$. Thus, utilizing the spherical expansion (Eq. S.10) of the generalized Coulomb kernel, we obtain

$$\left(\nabla_{\mathbf{r}} \frac{e^{-\kappa|\mathbf{r}-\mathbf{r}'+\boldsymbol{\tau}_i-\boldsymbol{\tau}_r-\mathbf{R}_p|}}{|\mathbf{r}-\mathbf{r}'+\boldsymbol{\tau}_i-\boldsymbol{\tau}_r-\mathbf{R}_p|}\right)_\alpha = 4\pi \sum_{l_1m_1} h_{l_1}^m(\kappa|\mathbf{r}'+\boldsymbol{\tau}_r-\boldsymbol{\tau}_i+\mathbf{R}_p|) Y_{l_1m_1}\left[\frac{\mathbf{r}'+\boldsymbol{\tau}_r-\boldsymbol{\tau}_i+\mathbf{R}_p}{|\mathbf{r}'+\boldsymbol{\tau}_r-\boldsymbol{\tau}_i+\mathbf{R}_p|}\right]\left[\nabla_{\mathbf{r}} j_{l_1}^m(\kappa r) Y_{l_1m_1}(\hat{\mathbf{r}})\right]_\alpha, \tag{S.11}$$

where the $\alpha$-th component of the gradient of the generalized Coulomb kernel is related to the gradient of the spherical Bessel function $j_l^m(\kappa\mathbf{r})$. This expression can be reformulated using the one-center expansion of the spherical Hankel functions [2, 3]

$$h_{l_1}^m(\kappa|\mathbf{r}'+\boldsymbol{\tau}_r-\boldsymbol{\tau}_i+\mathbf{R}_p|) Y_{l_1m_1}\left[\frac{\mathbf{r}'+\boldsymbol{\tau}_r-\boldsymbol{\tau}_i+\mathbf{R}_p}{|\mathbf{r}'+\boldsymbol{\tau}_r-\boldsymbol{\tau}_i+\mathbf{R}_p|}\right] = \sum_{l_2m_2} j_{l_2}^m(\kappa r') Y_{l_2m_2}(\hat{\mathbf{r}}') S^{\boldsymbol{\tau}_i l_1 m_1}_{(\boldsymbol{\tau}_r+\mathbf{R}_p) l_2 m_2}(\kappa; \boldsymbol{\tau}_r - \boldsymbol{\tau}_i), \tag{S.12}$$

where $S^{\boldsymbol{\tau}_i l_1 m_1}_{(\boldsymbol{\tau}_r+\mathbf{R}_p) l_2 m_2}(\kappa; \boldsymbol{\tau}_r - \boldsymbol{\tau}_i)$ is the bare structure constant which only depends on the energy parameter $\varepsilon$ and on the atomic positions via the difference $\boldsymbol{\tau}_r - \boldsymbol{\tau}_i$. More information is provided in Sec. S.4 A. Combining Eqs. (S.9), (S.11), and (S.12) for the cases $\boldsymbol{\tau}_i = \boldsymbol{\tau}_r; \mathbf{R}_p \neq 0$ and $\boldsymbol{\tau}_i \neq \boldsymbol{\tau}_r; \forall \mathbf{R}_p$, we obtain [4]

$$-\lim_{\kappa\to 0} \frac{Z_r}{\sqrt{\Omega_0}} \sum_i \sum_{lm} \sum_{l_1m_1} \sum_{l_2m_2} S^{\boldsymbol{\tau}_i\boldsymbol{\tau}_r}_{l_1m_1,l_2m_2}(\kappa;\mathbf{q}) \int_{\Omega_i} d\mathbf{r}' \delta(\mathbf{r}') j_{l_2}^m(\kappa r') Y_{l_2m_2}(\hat{\mathbf{r}}') \int_{\Omega_i} d\mathbf{r} \left[\nabla_{\mathbf{r}} j_{l_1}^m(\kappa r) Y_{l_1m_1}(\hat{\mathbf{r}})\right]_\alpha P^{\mathbf{q}+\mathbf{G}\,*}_{\boldsymbol{\tau}_i l m_l}(\mathbf{r}) \tag{S.13}$$

where the following notation for the Bloch sum of the structure constant has been introduced to have a more compact form

$$S^{\boldsymbol{\tau}_i\boldsymbol{\tau}_r}_{l_1m_1,l_2m_2}(\kappa;\mathbf{q}) = \begin{cases} \bar{S}_{\boldsymbol{\tau}_i l_1 m_1, \boldsymbol{\tau}_r l_2 m_2}(\kappa;\mathbf{q}) & \text{if } \boldsymbol{\tau}_i \neq \boldsymbol{\tau}_r \\ \bar{S}^{p\neq 0}_{\boldsymbol{\tau}_r l_1 m_1, \boldsymbol{\tau}_r l_2 m_2}(\kappa;\mathbf{q}) & \text{if } \boldsymbol{\tau}_i = \boldsymbol{\tau}_r \end{cases} \tag{S.14}$$

with

$$S_{\tau_i l_1 m_1, \tau_r l_2 m_2}(\kappa, \mathbf{q}) = \sum_p e^{i\mathbf{q}\cdot\mathbf{R}_p} \times \times 4\pi S^{\boldsymbol{\tau}_i l_1 m_1}_{(\boldsymbol{\tau}_r+\mathbf{R}_p) l_2 m_2}(\kappa; \boldsymbol{\tau}_r - \boldsymbol{\tau}_i). \tag{S.15}$$

and

$$\bar{S}^{p\neq 0}_{\boldsymbol{\tau}_i l_1 m_1, \boldsymbol{\tau}_r l_2 m_2}(\kappa;\mathbf{q}) = \sum_{p\neq 0} e^{i\mathbf{q}\cdot\mathbf{R}_p} \times \times 4\pi S^{\boldsymbol{\tau}_i l_1 m_1}_{(\boldsymbol{\tau}_r+\mathbf{R}_p) l_2 m_2}(\kappa; \boldsymbol{\tau}_r - \boldsymbol{\tau}_i). \tag{S.16}$$

The incomplete Bloch sum in Eq. (S.16) is related to the condition $\boldsymbol{\tau}_i = \boldsymbol{\tau}_r$ and $\mathbf{R}_p \neq 0$. The structure constant would be divergent if the condition ($\boldsymbol{\tau}_i = \boldsymbol{\tau}_r; \mathbf{R}_p = 0$) was satisfied due to the divergence of the spherical Hankel function at the origin, as shown in Sec. S.4 A. This latter contribution is absent in Eq. (S.13) and will be explicitly addressed in Sec. S.1 A 2.

To solve the integral on the integration space $\mathbf{r}'$ in Eq. (S.13), we need to utilize the Dirac-delta function in spherical coordinates $\delta(\mathbf{r}') = \delta(r')\delta(\theta)\delta(\phi)/r'^2 \sin\theta$, yielding

$$\int_{\Omega_i} d\mathbf{r}' \delta(\mathbf{r}') j_{l_2}^m(\kappa r') Y_{l_2m_2}(\hat{\mathbf{r}}') = = \lim_{r'\to 0} \delta_{m_2 0} \frac{\sqrt{2l_2+1}}{2\sqrt{\pi}} j_{l_2}^m(\kappa r') = \lim_{r'\to 0} \delta_{m_2 0} \frac{\sqrt{2l_2+1}}{2\sqrt{\pi}} \frac{r'^{l_2}}{(2l_2+1)!!}, \tag{S.17}$$

where the asymptotic limit (Eq. S.107) of the Bessel function has been used with the Dirac delta $\delta(r')$ along the integration domain $[0, s_i]$. Here, $r'^{l_2}$ is non-zero in the limit $r' \to 0$ if and only if $l_2 = 0$, so the above integral becomes

$$\int_{\Omega_i} d\mathbf{r}' \delta(\mathbf{r}') j_{l_2}^m(\kappa r') Y_{l_2m_2}(\hat{\mathbf{r}}') = \tfrac{1}{\sqrt{4\pi}} \delta_{m_2 0} \delta_{l_2 0}. \tag{S.18}$$

Using this result, Eq. (S.13) can then be rewritten as

$$\lim_{\kappa\to 0} -\frac{Z_r}{\sqrt{4\pi\Omega_0}} \sum_{lm_l} \sum_{l_1m_1} \sum_i S^{\boldsymbol{\tau}_i\boldsymbol{\tau}_r}_{l_1m_1,00}(\kappa;\mathbf{q}) \times \times \int_{\Omega_i} d\mathbf{r} \left[\nabla_{\mathbf{r}} j_{l_1}^m(\kappa r) Y_{l_1m_1}(\hat{\mathbf{r}})\right]_\alpha P^{\mathbf{q}+\mathbf{G}\,*}_{\boldsymbol{\tau}_i l m_l}(\mathbf{r}). \tag{S.19}$$

The functions $P^{\mathbf{q}+\mathbf{G}}_{\boldsymbol{\tau}_i l m_l}$ defined by Eq. (90) can also be restated in terms of the Methfessel convention for the spherical Bessel functions $j_l^m(|\mathbf{q}+\mathbf{G}|r) = j_l(|\mathbf{q}+\mathbf{G}|r)/|\mathbf{q}+\mathbf{G}|^l$ as

$$P^{\mathbf{q}+\mathbf{G}}_{\boldsymbol{\tau}_i lm}(\mathbf{r}) = \eta^{\mathbf{q}+\mathbf{G}}_{\boldsymbol{\tau}_i,lm} j_l^m(|\mathbf{q}+\mathbf{G}|r)\, Y_{lm}(\widehat{\mathbf{r}})\,, \tag{S.20}$$

where

$$\eta^{\mathbf{q}+\mathbf{G}}_{\boldsymbol{\tau}_i,lm} = 4\pi i^l |\mathbf{q}+\mathbf{G}|^l e^{i(\mathbf{q}+\mathbf{G})\cdot\boldsymbol{\tau}_i} Y_{lm}(\widehat{\mathbf{q}+\mathbf{G}}) \tag{S.21}$$

Finally, by combining Eqs. (S.19)-(S.21) and utilizing the definition for the gradient $\nabla_{\mathbf{r}} j^m_{l_1}(\kappa r) Y_{l_1 m_1}(\widehat{\mathbf{r}})$ provided in Sec. S.4 C 3, we obtain

$$-\lim_{\kappa\to 0}\frac{Z_r}{\sqrt{4\pi\Omega_0}}\sum_{lm}\sum_i S^{\boldsymbol{\tau}_i\boldsymbol{\tau}_r}_{lm,00}(\kappa;\mathbf{q})\Bigg\{\sqrt{\frac{l}{2l+1}}\int_0^{s_i} dr r^2 j^m_{l-1}(\kappa r) j^m_{l-1}(|\mathbf{q}+\mathbf{G}|r)\sum_{\nu=-l+1}^{l-1}\eta^{\mathbf{q}+\mathbf{G}\,*}_{\boldsymbol{\tau}_i,l-1\nu}\,\gamma^{lm}_{l-1,\nu,\alpha} + \\ +\varepsilon\sqrt{\frac{l+1}{2l+1}}\int_0^{s_i} dr r^2 j^m_{l+1}(\kappa r) j^m_{l+1}(|\mathbf{q}+\mathbf{G}|r)\sum_{\nu=-l-1}^{l+1}\eta^{\mathbf{q}+\mathbf{G}\,*}_{\boldsymbol{\tau}_i,l+1\nu}\,\gamma^{lm}_{l+1,\nu,\alpha}\Bigg\} \tag{S.22}$$

where $\{\gamma^{lm}_{l\pm1,\nu,\alpha}\}$ is a set of coefficients introduced in Sec. S.4 C 3 and required for rewriting the $\alpha$-th component of the real tensor spherical harmonics in terms of real spherical harmonics

$$\widehat{\boldsymbol{e}}_\alpha\cdot\sum_{\mu=-l}^{l}\mathbf{Y}^{m\mu\nu}_{l,l\pm1}(\widehat{\mathbf{r}}) = \gamma^{lm}_{l\pm1,\nu\,\alpha} Y_{l\pm1,\nu}(\widehat{\mathbf{r}})\,. \tag{S.23}$$

The Lommel's type integrals

$$\mathcal{L}^{\boldsymbol{\tau}_i}_l(\kappa,|\mathbf{q}+\mathbf{G}|) = \int_0^{s_i} dr r^2 j^m_l(\kappa r) j^m_l(|\mathbf{q}+\mathbf{G}|r) \tag{S.24}$$

involving the products of two spherical Bessel functions can be solved analytically as shown in Sec. S.4 A.

### 2. *Case* $\boldsymbol{\tau}_i - \boldsymbol{\tau}_r - \mathbf{R}_p = 0$

In this section, we address the remaining term in Eq. (S.22), with null lattice vector $\mathbf{R}_p = \mathbf{0}$ and $\boldsymbol{\tau}_r = \boldsymbol{\tau}_i$, so fixing $i = r$ when iterating over the nuclear positions in Eq. (S.8). Leveraging the knowledge that the smooth Hankel function with $l = 0$—within Methfessel's convention defined as $h^m_0(\kappa r) = \exp(-\kappa r)/r$—coincides with the bare Coulomb kernel, the gradient of the Yukawa kernel can then be reformulated as

$$\left(\nabla_{\mathbf{r}}\frac{e^{-\kappa r}}{r}\right)_\alpha = \left[\nabla_{\mathbf{r}} h^m_0(\kappa r)\right]_\alpha \\ = -\sqrt{\tfrac{4\pi}{3}}\, h^m_1(\kappa r) Y_{1\nu(\alpha)}(\widehat{\mathbf{r}})\,. \tag{S.25}$$

Here, we utilized the derivative definition (S.121) for the smooth Hankel functions introduced in Sec. S.4 A and the index $\nu(\alpha)$ maps between Cartesian coordinates and the real spherical harmonics index $m$, i.e., $\nu(x) = 1, \nu(y) = -1, \nu(z) = 0$. Upon inserting Eqs. (S.20) and (S.25) into Eq. (S.8) for the only term with $\boldsymbol{\tau}_i = \boldsymbol{\tau}_r$ and $\mathbf{R}_p = \mathbf{0}$, we derive

$$\lim_{\kappa\to 0}\sqrt{\frac{4\pi}{3\Omega_0}}\, Z_r \eta^{\mathbf{q}+\mathbf{G}\,*}_{\boldsymbol{\tau}_r,1\nu(\alpha)}\mathcal{H}^{\boldsymbol{\tau}_r}_1(\kappa,|\mathbf{q}+\mathbf{G}|)\,, \tag{S.26}$$

where

$$\mathcal{H}^{\boldsymbol{\tau}_r}_1(\kappa,|\mathbf{q}+\mathbf{G}|) = \int_0^{s_r} dr r^2 h^m_1(\kappa r) j^m_1(|\mathbf{q}+\mathbf{G}|r) \tag{S.27}$$

is a Lommel's type integral involving the product of spherical Hankel and Bessel functions. Through a derivation akin to that employed in Sec. S.1 A 1, we establish the relation $\eta^{\mathbf{q}+\mathbf{G}}_{\boldsymbol{\tau}_r,1\nu(\alpha)} = -\sqrt{3}\sum_{\mu=-1}^{1}\eta^{\mathbf{q}+\mathbf{G}}_{\boldsymbol{\tau}_r,1\mu}\gamma^{00}_{1,\mu,\alpha}$, resulting in the reconfiguration of expression (S.26) as

$$-\lim_{\kappa\to 0}\frac{\sqrt{4\pi}Z_r}{\sqrt{\Omega_0}}\sum_{\mu=-1}^{1}\eta^{\mathbf{q}+\mathbf{G}\,*}_{\boldsymbol{\tau}_r,1\mu}\gamma^{00}_{1,\mu,\alpha}\mathcal{H}^r_1(\kappa,|\mathbf{q}+\mathbf{G}|) \tag{S.28}$$

Finally, by combining Eqs. (S.4), (S.6), (S.22), and (S.28) we arrive at

$$\int_{\Omega_0} d\mathbf{r} P_{\mathbf{G}}^{\mathbf{q}\,*}(\mathbf{r}) \frac{\partial V_r^{(0)\,\mathbf{q}}(\mathbf{r})}{\partial r_\alpha} =$$

$$= -\frac{i}{\sqrt{\Omega_0}} \frac{4\pi Z_r (\mathbf{q}+\mathbf{G})_\alpha}{|\mathbf{k}+\mathbf{G}'|^2+\kappa^2} e^{i(\mathbf{q}+\mathbf{G})\cdot\boldsymbol{\tau}_r} - \frac{\sqrt{4\pi} Z_r}{\sqrt{\Omega_0}} \sum_{\mu=-1}^{1} \eta_{\boldsymbol{\tau}_r,1\mu}^{\mathbf{q}+\mathbf{G}\,*} \gamma_{1,\mu,\alpha}^{00} \mathcal{H}_1^{\boldsymbol{\tau}_r}(\kappa, |\mathbf{q}+\mathbf{G}|) - \frac{Z_r}{\sqrt{4\pi\Omega_0}} \sum_{lm} \sum_{i} S_{lm,00}^{\boldsymbol{\tau}_i\boldsymbol{\tau}_r}(\kappa;\mathbf{q}) \times$$

$$\times \left\{ \sqrt{\frac{l}{2l+1}} \mathcal{L}_{l-1}^{\boldsymbol{\tau}_i}(\kappa, |\mathbf{q}+\mathbf{G}|) \sum_{\nu=-l+1}^{l-1} \eta_{\boldsymbol{\tau}_i,l-1\nu}^{\mathbf{q}+\mathbf{G}\,*} \gamma_{l-1,\nu,\alpha}^{lm} + \varepsilon \sqrt{\frac{l+1}{2l+1}} \mathcal{L}_{l+1}^{\boldsymbol{\tau}_i}(\kappa, |\mathbf{q}+\mathbf{G}|) \sum_{\nu=-l-1}^{l+1} \eta_{\boldsymbol{\tau}_i,l+1\nu}^{\mathbf{q}+\mathbf{G}\,*} \gamma_{l+1,\nu,\alpha}^{lm} \right\} \quad \text{(S.29)}$$

in the $\kappa \to 0$ limit.

### B. Reduced *e-ph* matrix element integral evaluated in the augmentation region

Combining Eq. (S.2) with the radial product basis Bloch functions, Eq. (91), we obtain

$$\int_{\Omega_0} d\mathbf{r} \, \frac{\partial V_r^{(0)\mathbf{q}}(\mathbf{r})}{\partial r_\alpha} B_{\boldsymbol{\tau}_i a l_a m_a}^{\mathbf{q}\,*}(\mathbf{r}) = \frac{1}{\sqrt{\Omega_0}} \int_{\Omega_0} d\mathbf{r} \, \frac{\partial V_r^{(0)\mathbf{q}}(\mathbf{r})}{\partial r_\alpha} \left[ \sum_p e^{i\mathbf{q}\cdot\mathbf{R}_p} B_{\boldsymbol{\tau}_i+\mathbf{R}_p a l_a m_a}(\mathbf{r}) \theta(s_i - |\mathbf{r}-\boldsymbol{\tau}_i-\mathbf{R}_p|) \right]^* \;\; \forall \; \boldsymbol{\tau}_i, a, l_a m_a. \quad \text{(S.30)}$$

The radial product basis functions $B_{\boldsymbol{\tau}_i a l_a m_a}$ are non-zero solely within the $i$-th augmentation sphere. Hence, integration in Eq. (S.30) is restricted to the volume $\Omega_i$, resulting in

$$\int_{\Omega_0} d\mathbf{r} \, \frac{\partial V_r^{(0)\mathbf{q}}(\mathbf{r})}{\partial r_\alpha} B_{\boldsymbol{\tau}_i a l_a m_a}^{\mathbf{q}\,*}(\mathbf{r}) = -\lim_{\kappa\to 0} \frac{Z_r}{\sqrt{\Omega_0}} \sum_p e^{i\mathbf{q}\cdot\mathbf{R}_p} \int_{\Omega_i} \int_{\Omega_i} d\mathbf{r} d\mathbf{r}' \left( \nabla_{\mathbf{r}} \frac{e^{-\kappa|\mathbf{r}-\mathbf{r}'+\boldsymbol{\tau}_i-\boldsymbol{\tau}_r-\mathbf{R}_p|}}{|\mathbf{r}-\mathbf{r}'+\boldsymbol{\tau}_i-\boldsymbol{\tau}_r-\mathbf{R}_p|} \right)_\alpha B_{\boldsymbol{\tau}_i a l_a m_a}(\mathbf{r}) \delta(\mathbf{r}') \,. \quad \text{(S.31)}$$

To get to this result, we used the Bloch sum for the electron-nuclear potential, the generalized Coulomb potential expansion (S.10), the variable transformation described in Eqs. (S.7) and (S.8), and the Dirac delta manipulation. Similar to Sec. S.1 A 1, two scenarios emerge when utilizing the spherical expansion of the generalized Coulomb potential, i.e. (i) the case $\boldsymbol{\tau}_i - \boldsymbol{\tau}_r \neq \mathbf{R}_p$ and (ii) the case $\boldsymbol{\tau}_i - \boldsymbol{\tau}_r - \mathbf{R}_p = \mathbf{0}$.

#### 1. *Case* $\boldsymbol{\tau}_i - \boldsymbol{\tau}_r - \mathbf{R}_p \neq 0$

As demonstrated in Sec. S.1 A 1, when $\boldsymbol{\tau}_i - \boldsymbol{\tau}_r \neq \mathbf{R}_p$ the relation $r < |\mathbf{r}' + \boldsymbol{\tau}_r - \boldsymbol{\tau}_i + \mathbf{R}_p|$ holds, allowing us to utilize the spherical expansions (S.11) and (S.12) for evaluating the gradient of the generalized Coulomb potential, resulting in

$$\sum_{l_1 m_{l_1}} \frac{Z_r S_{lm,00}^{\boldsymbol{\tau}_i\boldsymbol{\tau}_r}(\kappa;\mathbf{q})}{(-)\sqrt{4\pi\Omega_0}} \int_{\Omega_i} d\mathbf{r} \big[\nabla_{\mathbf{r}} j_l^m(\kappa r) Y_{lm}(\widehat{\mathbf{r}})\big]_\alpha B_{\boldsymbol{\tau}_i a l_a m_a}(\mathbf{r}) \quad \text{(S.32)}$$

in the $\kappa \to 0$ limit. To achieve this result, we employed Eq. (S.18) and defined $S_{lm,00}^{\boldsymbol{\tau}_i\boldsymbol{\tau}_r}(\kappa;\mathbf{q})$ as described in Eqs. (S.14)-(S.16). Once again, we omit consideration of the case $\boldsymbol{\tau}_i = \boldsymbol{\tau}_r$ and $\mathbf{R}_p = \mathbf{0}$, where the Bloch-summed structure constant could potentially diverge at nuclear positions. Referring to the definition of the gradient $\nabla_{\mathbf{r}} j_l^m(\kappa r) Y_{lm}(\widehat{\mathbf{r}})$ provided in S.4 C 3, the above equation can be reformulated as

$$-\frac{Z_r}{\sqrt{4\pi\Omega_0}} \sum_{lm} S_{lm,00}^{\boldsymbol{\tau}_i\boldsymbol{\tau}_r}(\kappa;\mathbf{q}) \left\{ \sqrt{\frac{l}{2l+1}} \sum_{\nu=-l+1}^{l-1} \gamma_{l-1,\nu,\alpha}^{lm} \varrho_{\boldsymbol{\tau}_i a}^{(l-1)}(\kappa) \delta_{l-1.l_a} \delta_{\nu m_a} + \varepsilon \sqrt{\frac{l+1}{2l+1}} \sum_{\nu=-l-1}^{l+1} \gamma_{l+1,\nu,\alpha}^{lm} \varrho_{\boldsymbol{\tau}_i a}^{(l+1)}(\kappa) \delta_{l+1,l_a} \delta_{\nu m_a} \right\} \quad \text{(S.33)}$$

in the $\kappa \to 0$ limit, where the radial integral

$$\varrho_{\boldsymbol{\tau}_i a}^{(l)}(\kappa) = \int_0^{s_i} dr r^2 j_l^m(\kappa r) B_{\boldsymbol{\tau}_i a l}(r) \quad \text{(S.34)}$$

involves the product of smooth Bessel functions and radial product basis functions and is computed numerically.

### 2. Case $\boldsymbol{\tau}_i - \boldsymbol{\tau}_r - \mathbf{R}_p = 0$

In this section, we focus on Eq. (S.31) in the case $\boldsymbol{\tau}_r = \boldsymbol{\tau}_i$ and with a null lattice vector $\mathbf{R}_p = \mathbf{0}$. Utilizing the gradient (S.25) for the bare Yukawa kernel and combining it with Eq. (S.31) for this specific case, yields

$$\lim_{\kappa\to 0} Z_r \sqrt{\frac{4\pi}{3\Omega_0}} \int_0^{s_r} dr r^2 h_1^m(\kappa r) B_{\boldsymbol{\tau}_r a 1}(r) \delta_{l_a 1} \delta_{m_a \nu(\alpha)} \, . \tag{S.35}$$

Following the approach outlined in Sec. S.1 A 2, we can reformulate the above expression using the set of coefficients $\{\gamma^{00}_{1,\mu,\alpha}\}$, which are used to express the $\alpha$-th component of the real tensor spherical harmonics in terms of real spherical harmonics. This yields

$$\frac{1}{\sqrt{\Omega_0}} \int_{\Omega_0} d\mathbf{r} \, \frac{\partial V_r^{(0)\mathbf{q}}(\mathbf{r})}{\partial r_\alpha} \left[ B_{\boldsymbol{\tau}_r a l_a m_a}(\mathbf{r}) \theta(s_r - |\mathbf{r} - \boldsymbol{\tau}_r|) \right] = = -\frac{Z_r \sqrt{4\pi} \delta_{l_a 1}}{\sqrt{\Omega_0}} \sum_{\mu=-1}^{-1} \gamma^{00}_{1,\mu,\alpha} \delta_{m_a \mu} \varsigma^{(1)}_{\boldsymbol{\tau}_r a}(\kappa) \tag{S.36}$$

in the $\kappa \to 0$ limit, where the radial integral

$$\varsigma^{(1)}_{\boldsymbol{\tau}_r a}(\kappa) = \int_0^{s_r} dr r^2 h_1^m(\kappa r) B_{\boldsymbol{\tau}_r a 1}(r) \tag{S.37}$$

involves the product of the Hankel function $h_1^m(\kappa r)$ and radial product basis functions and is computed numerically.

## C. Integral (S.1) evaluated in the interstitial region

The derivation of the integral (S.3), related to the electron core contribution to the screening of the bare Coulomb interaction, is straightforward in the fully plane wave case and for the plane wave expansion inside the augmentation region when $\boldsymbol{\tau}_i - \boldsymbol{\tau}_r - \mathbf{R}_p \neq 0$. However, for the case $\boldsymbol{\tau}_i = \boldsymbol{\tau}_r$ and $\mathbf{R}_p = 0$, the derivation is more complex, and the simplification provided by Eq. (S.25) cannot be utilized. In this section, we focus on the derivation for the latter case and provide the complete expression for the integral (S.3) at its conclusion. Within the augmentation region, the plane wave contribution to Eq. (S.3) can be expressed as

$$\frac{1}{\sqrt{\Omega_0}} \lim_{\kappa\to 0} \sum_{ip} \sum_{lm} e^{i\mathbf{q}\cdot\mathbf{R}_p} \int_{\Omega_i} \int_{\Omega_i} d\mathbf{r} d\mathbf{r}' P^{\mathbf{q}+\mathbf{G}\,*}_{\boldsymbol{\tau}_i lm}(\mathbf{r}) n^c_{e,i}(\mathbf{r}') \times \times \left( \nabla_{\mathbf{r}} \frac{e^{-\kappa|\mathbf{r}-\mathbf{r}'+\boldsymbol{\tau}_i-\boldsymbol{\tau}_r-\mathbf{R}_p|}}{|\mathbf{r}-\mathbf{r}'+\boldsymbol{\tau}_i-\boldsymbol{\tau}_r-\mathbf{R}_p|} \right)_\alpha , \tag{S.38}$$

Note that Eq. (S.9) can be regarded as a generalization of the above expression (S.38) where $n^c_{e,i}(\mathbf{r}')$ is replaced by $-Z_i \delta(\mathbf{r}')$. In the specific case of interest, characterized by the conditions $\boldsymbol{\tau}_i = \boldsymbol{\tau}_r$ and $\mathbf{R}_p = 0$, Eq. (S.38) becomes

$$\lim_{\kappa\to 0} \frac{1}{\sqrt{\Omega_0}} \sum_{lm} \int_{\Omega_r} \int_{\Omega_r} d\mathbf{r} d\mathbf{r}' P^{\mathbf{q}+\mathbf{G}\,*}_{\boldsymbol{\tau}_r lm}(\mathbf{r}) n^c_{e,r}(\mathbf{r}') \times \times \left( \nabla_{\mathbf{r}} \frac{e^{-\kappa|\mathbf{r}-\mathbf{r}'|}}{|\mathbf{r}-\mathbf{r}'|} \right)_\alpha \tag{S.39}$$

where the gradient of the generalized Coulomb kernel is expanded in terms of spherical harmonics as

$$\left( \nabla_{\mathbf{r}} \frac{e^{-\kappa|\mathbf{r}-\mathbf{r}'|}}{|\mathbf{r}-\mathbf{r}'|} \right)_\alpha = 4\pi \sum_{l'm'} Y_{l'm'}(\hat{\mathbf{r}}') \left[ \nabla_{\mathbf{r}} f_{l'}(r, r'; \kappa) Y_{l'm'}(\hat{\mathbf{r}}) \right]_\alpha \tag{S.40}$$

with the non-local function $f_{l'}(r, r'; \kappa)$ defined as

$$f_{l'}(r, r'; i\kappa) = \begin{cases} j^m_{l'}(\kappa r) h^m_{l'}(\kappa r') & \text{if } r < r' \\ h^m_{l'}(\kappa r) j^m_{l'}(\kappa r') & \text{if } r > r' \, . \end{cases} \tag{S.41}$$

To utilize the identities provided in Eq. (S.41), we divide the radial integral over $r'$ into two regions, i.e. $\int_0^{s_r} dr' = \int_0^r dr' + \int_r^{s_r} dr'$. Hence, making use of the gradients in Sec. S.4 C 3 for $l = 0$,

$$\begin{aligned} \left[ \nabla_{\mathbf{r}} j_0^m(\kappa r) Y_{00}(\hat{\mathbf{r}}) \right]_\alpha &= \varepsilon \sum_{\nu=-1}^{1} \gamma^{00}_{l+1,\nu,\alpha} j_1^m(\kappa r) Y_{1\nu}(\hat{\mathbf{r}}) \\ \left[ \nabla_{\mathbf{r}} h_0^m(\kappa r) Y_{00}(\hat{\mathbf{r}}) \right]_\alpha &= \sum_{\nu=-1}^{1} \gamma^{00}_{l+1,\nu,\alpha} h_1^m(\kappa r) Y_{1\nu}(\hat{\mathbf{r}}) \, , \end{aligned} \tag{S.42}$$

condition selected by the spherical symmetry of the core density $n^c_{e,i}(\mathbf{r}') = n^c_{e,i}(r') Y_{00}(\hat{\mathbf{r}}')$, and summing Eq. (S.39) with the $V^{(0)}_{rl}$-dependent term, Eq. (S.28), yields,

$$-\lim_{\kappa\to 0} \sqrt{\frac{4\pi}{\Omega_0}} \sum_{\mu=-1}^{1} \eta^{\mathbf{q}+\mathbf{G}\,*}_{\boldsymbol{\tau}_r,1\mu} \gamma^{00}_{1,\mu,\alpha} \times \times \int_0^{s_r} dr r^2 h_1^m(\kappa r) j_1^m(|\mathbf{q}+\mathbf{G}| r) Z_r^{(2)}(\kappa, r) \tag{S.43}$$

Here, the function $Z_r^{(2)}(\kappa, r)$ indicates an effective charge and is defined as

$$Z_r^{(2)}(\kappa, r) = Z_r^{(1)}(\kappa, r) - \frac{\sqrt{4\pi} \varepsilon j_1^m(\kappa r)}{h_1^m(\kappa r)} \times \times \left[ \int_0^{s_r} dr' r'^2 n^c_{e,r}(r') h_1^m(\kappa r') - \int_0^r dr' r'^2 n^c_{e,r}(r') h_1^m(\kappa r') \right] \tag{S.44}$$

with

$$Z_r^{(1)}(\kappa, r) = Z_r - \sqrt{4\pi} \int_0^r dr' r'^2 n^c_{e,r}(r') j_0^m(\kappa r') \, . \tag{S.45}$$

It can be demonstrated that in the limiting case of an electronic core charge $Z_r^c$ localized at the nuclear

position—i.e. without any spatial distribution, $n^c_{e,r}(\mathbf{r}) = Z^c_r\delta(\mathbf{r})$—Eq. (S.18) provides $Z^{(2)}_r(\kappa,r) = Z^{(1)}_r(\kappa) = Z_r - Z^c_r$, indicating the effective screened nuclear charge for the nucleus at the equilibrium position $\boldsymbol{\tau}^0_r$.

Finally, combining the result (S.43) with the fully plane wave case and the plane wave expansion inside the augmentation sphere for $\boldsymbol{\tau}_i - \boldsymbol{\tau}_r - \mathbf{R}_p \neq 0$ yields the following expression

$$\int_{\Omega_0} d\mathbf{r} P^{\mathbf{q}\,*}_{\mathbf{G}}(\mathbf{r}) \frac{\partial \widetilde{V}^{(0)\,\mathbf{q}}_r(\mathbf{r})}{\partial r_\alpha} = -\frac{i}{\sqrt{\Omega_0}} \frac{4\pi Z^{(1)}_r(|\mathbf{q}+\mathbf{G}|, s_r)(\mathbf{q}+\mathbf{G})_\alpha}{|\mathbf{k}+\mathbf{G}'|^2+\kappa^2} e^{i(\mathbf{q}+\mathbf{G})\cdot\boldsymbol{\tau}_r} - $$
$$-\sqrt{\frac{4\pi}{\Omega_0}} \sum_{\mu=-1}^{1} \eta^{\mathbf{q}+\mathbf{G}\,*}_{\boldsymbol{\tau}_r,1\mu} \gamma^{00}_{1,\mu,\alpha} \int_0^{s_r} dr r^2 h^m_1(\kappa r) j^m_1(|\mathbf{q}+\mathbf{G}|r) Z^{(2)}_r(\kappa,r) - \frac{Z^{(1)}_r(\kappa,s_r)}{\sqrt{4\pi\Omega_0}} \sum_{lm}\sum_{i} S^{\boldsymbol{\tau}_i\boldsymbol{\tau}_r}_{lm,00}(\kappa;\mathbf{q}) \times$$
$$\times \left\{ \sqrt{\frac{l}{2l+1}} \mathcal{L}^{\boldsymbol{\tau}_i}_{l-1}(\kappa,|\mathbf{q}+\mathbf{G}|) \sum_{\nu=-l+1}^{l-1} \eta^{\mathbf{q}+\mathbf{G}\,*}_{\boldsymbol{\tau}_i,l-1\nu}\, \gamma^{lm}_{l-1,\nu,\alpha} + \varepsilon \sqrt{\frac{l+1}{2l+1}} \mathcal{L}^{\boldsymbol{\tau}_i}_{l+1}(\kappa,|\mathbf{q}+\mathbf{G}|) \sum_{\nu=-l-1}^{l+1} \eta^{\mathbf{q}+\mathbf{G}\,*}_{\boldsymbol{\tau}_i,l+1\nu}\, \gamma^{lm}_{l+1,\nu,\alpha} \right\} \quad \text{(S.46)}$$

in the $\kappa \to 0$ limit. Here, $Z^{(1)}_r(|\mathbf{q}+\mathbf{G}|, s_r)$ corresponds to Eq. (S.45) with the modulus $|\mathbf{q}+\mathbf{G}|$ replacing $\kappa$. Note that Eq. (S.46) has a structure equivalent to Eq. (S.29) but with bare nuclear charges replaced by the effective nuclear charges $Z^{(1)}_r$ and $Z^{(2)}_r$.

### D. Integral (S.1) evaluated in the augmentation region

In this section we present the expressions for the integral (S.1) solved while using radial product basis functions. Then, when the condition $\boldsymbol{\tau}_i - \boldsymbol{\tau}_r - \mathbf{R}_p \neq 0$ is satisfied, the integral becomes

$$\int_{\Omega_0} d\mathbf{r}\, \frac{\partial \widetilde{V}^{(0)\mathbf{q}}_r(\mathbf{r})}{\partial r_\alpha} B^{\mathbf{q}\,*}_{\boldsymbol{\tau}_i a l_a m_a}(\mathbf{r}) = -\lim_{\kappa\to 0} \frac{Z^{(1)}_r(\kappa,s_r)}{\sqrt{4\pi\Omega_0}} \sum_{lm} S^{\boldsymbol{\tau}_i\boldsymbol{\tau}_r}_{lm,00}(\kappa;\mathbf{q}) \Bigg\{ \sqrt{\frac{l}{2l+1}} \sum_{\nu=-l+1}^{l-1} \gamma^{lm}_{l-1,\nu,\alpha} \rho^{(l-1)}_{\boldsymbol{\tau}_i a} \delta_{l-1.l_a} \delta_{\nu m_a} +$$
$$+ \varepsilon \sqrt{\frac{l+1}{2l+1}} \sum_{\nu=-l-1}^{l+1} \gamma^{lm}_{l+1,\nu,\alpha} \rho^{(l+1)}_{\boldsymbol{\tau}_i a} \delta_{l+1,l_a} \delta_{\nu m_a} \Bigg\}. \quad \text{(S.47)}$$

while for the remaining condition $\boldsymbol{\tau}_i = \boldsymbol{\tau}_r$ and $\mathbf{R}_p = 0$ we obtain

$$\int_{\Omega_0} d\mathbf{r}\, \frac{\partial \widetilde{V}^{(0)\mathbf{q}}_r(\mathbf{r})}{\partial r_\alpha} \Big[ B_{\boldsymbol{\tau}_r a l_a m_a}(\mathbf{r}) \theta(s_r - |\mathbf{r}-\boldsymbol{\tau}_r|) \Big] = \delta_{l_a 1} \sqrt{\frac{4\pi}{\Omega_0}} \sum_{\mu=-1}^{-1} \gamma^{00}_{1,\mu,\alpha} \delta_{m_a \nu(\alpha)} \int_0^{s_r} dr r^2 h^m_1(\kappa r) B_{\boldsymbol{\tau}_r a 1}(r) Z^{(2)}_r(\kappa,r) \quad \text{(S.48)}$$

## S.2. ROTATION OF THE ELECTRON-PHONON COUPLING MATRIX ON THE FULL BZ FOR THE ELECTRON AND PHONON WAVE VECTORS

In many applications, such as computing the Fan-Migdal *e-ph* self-energy $\Sigma^{\mathrm{FM}}_{nn,\mathbf{k}}(\varepsilon_{n\mathbf{k}})$, integrating over the phonon wave vectors $\mathbf{q}$ throughout the entire Brillouin zone (BZ) is essential. Nevertheless, the most computationally intensive step in evaluating the short-range *e-ph* matrix elements involves calculating the electronic inverse dielectric matrix $\varepsilon^{-1}_{e,v}(\mathbf{q})$ for each phonon wave vector $\mathbf{q}$. Consequently, it is necessary to find a method for rotating the *e-ph* matrix from the irreducible BZ (IBZ), so that $g_{in,\nu}(\mathbf{k},\mathbf{q}')$, with $\mathbf{q}' = \mathbf{S}\mathbf{q}$ and $\mathbf{q} \in$ IBZ, can be obtained through a symmetry operation. Note that, for the sake of simplicity, in this and the following sections, we will not use the *e-ph* matrix elements obtained via the downfolding approach described in Sec. VA (see Eq. 176). Instead, unless explicitly stated otherwise, we will rely on Eq. (175).

Here, the crystal point group symmetry operation $\mathcal{S}$ is

defined in the Seitz notation [5] as

$$\begin{aligned}\boldsymbol{\tau}_r = \mathcal{S}\boldsymbol{\tau}_s &= \{\mathbf{S}|\boldsymbol{v}\}\boldsymbol{\tau}_s + \bar{\boldsymbol{v}}_{\boldsymbol{\tau}_s}(\mathcal{S}) \\ &= \mathbf{S}\boldsymbol{\tau}_s + \boldsymbol{v}(\mathcal{S}) + \bar{\boldsymbol{v}}_{\boldsymbol{\tau}_s}(\mathcal{S}) \end{aligned} \tag{S.49}$$

where $\{\mathbf{S}|\boldsymbol{v}\}$ is a space group symmetry operator comprising a proper or improper rotation $\mathbf{S}$ and a possible fractional translation $v(\mathcal{S})$. The term $\bar{\boldsymbol{v}}_{\boldsymbol{\tau}_s}(\mathcal{S})$ represents a lattice translation required to map the rotated vector position $\{\mathbf{S}|\boldsymbol{v}\}\boldsymbol{\tau}_s$ onto an equivalent position $\boldsymbol{\tau}_r$ within the same sublattice.

By combining Eqs. (75)-(76) in the for a phonon momentum transfer $\mathbf{Sq}$, we arrive at the following expression of the *e-ph* matrix elements in terms of the reduced *e-ph* coupling function

$$\begin{aligned} g_{in,\nu}(\mathbf{k},\mathbf{Sq}) = \sum_{r\alpha}\sqrt{\frac{\hbar}{2m_r\omega_{\mathbf{q}\nu}}}e_{r\alpha,\nu}(\mathbf{Sq})\times \\ \times \langle\psi_{i,\mathbf{k}+\mathbf{Sq}}|\,\xi^{r\alpha}_{\mathbf{Sq}}\,|\psi_{n,\mathbf{k}}\rangle_{\Omega_0}\,, \end{aligned} \tag{S.50}$$

where the rotational invariance of the phonon frequencies, $\omega_{\mathbf{Sq}\nu} = \omega_{\mathbf{q}\nu}$, has been applied. The transformation law for the eigenmodes is given by

$$e_{r\alpha,\nu}(\mathbf{Sq}) = \sum_{s\beta}\left[\Gamma_{\{\mathbf{S}|\boldsymbol{v}\}}(\mathbf{q})\right]^{rs}_{\alpha\beta} e_{s\beta,\nu}(\mathbf{q}) \tag{S.51}$$

with

$$\left[\Gamma_{\{\mathbf{S}|\boldsymbol{v}\}}(\mathbf{q})\right]^{rs}_{\alpha\beta} = S_{\alpha\beta}\delta_{r,F_{\mathcal{S}}(s)}e^{i\mathbf{Sq}\cdot[\boldsymbol{\tau}_r-\{\mathbf{S}|\boldsymbol{v}\}\boldsymbol{\tau}_s]}\,. \tag{S.52}$$

Here, $\delta_{r,F_{\mathcal{S}}(s)}$ represents the interchange of sublattices, if any, and vanishes unless $\boldsymbol{\tau}_r$ corresponds to the sublattice $F_{\mathcal{S}}(s)$, which is reached from $\boldsymbol{\tau}_s$ by the crystal point group symmetry $\mathcal{S}$. When $\delta_{r,F_{\mathcal{S}}(s)} = 1$, the phase factor in Eq. (S.52) simplifies to

$$\begin{aligned}\boldsymbol{\tau}_r - \{\mathbf{S}|\boldsymbol{v}\}\boldsymbol{\tau}_s &= \mathcal{S}\boldsymbol{\tau}_s - \{\mathbf{S}|\boldsymbol{v}\}\boldsymbol{\tau}_s \\ &= \bar{\boldsymbol{v}}_{\boldsymbol{\tau}_s}(\mathcal{S})\,, \end{aligned} \tag{S.53}$$

using the definition in Eq. (S.49). Equation (S.51) implicitly assumes that the eigenmodes at $\mathbf{q}$ and $\mathbf{Sq}$ do not carry any additional phase difference beyond that due to possible lattice translation vectors $\bar{\boldsymbol{v}}_{\boldsymbol{\tau}_s}(\mathcal{S})$ between $\boldsymbol{\tau}_r$ and $\{\mathbf{S}|\boldsymbol{v}\}\boldsymbol{\tau}_s$ as expressed in Eq. (S.53). Additionally, it assumes that no gauge mixing occurs in the case of degeneracy among eigenmodes. Using the definition (S.51), we can rewrite Eq. (S.50) as

$$g_{in,\nu}(\mathbf{k},\mathbf{Sq}) = \sum_{s\beta}\sqrt{\frac{\hbar}{2\omega_{\mathbf{q}\nu}}}e_{s\beta,\nu}(\mathbf{q})\;\langle\psi_{i,\mathbf{k}+\mathbf{Sq}}|\sum_{r\alpha}\sqrt{\tfrac{1}{m_r}}\left[\Gamma_{\{\mathbf{S}|\boldsymbol{v}\}}(\mathbf{q})\right]^{rs}_{\alpha\beta}\xi^{r\alpha}_{\mathbf{Sq}}\,|\psi_{n,\mathbf{k}}\rangle_{\Omega_0}\,, \tag{S.54}$$

where, using Eq. (77), we obtain

$$\begin{aligned}\sum_{r\alpha}\sqrt{\tfrac{1}{m_r}}\left[\Gamma_{\{\mathbf{S}|\boldsymbol{v}\}}(\mathbf{q})\right]^{rs}_{\alpha\beta}\xi^{r\alpha}_{\mathbf{Sq}}(\mathbf{r}) &= \sum_{r\alpha}\sqrt{\tfrac{1}{m_r}}\left[\Gamma_{\{\mathbf{S}|\boldsymbol{v}\}}(\mathbf{q})\right]^{rs}_{\alpha\beta}\int_{\Omega}d\mathbf{r}'\,\varepsilon_e^{-1}(\mathbf{r},\mathbf{r}')\frac{\partial V_r^{(0)\,\mathbf{Sq}}(\mathbf{r}')}{\partial r'_\alpha} \\ &= \sum_{mr\alpha}\sqrt{\tfrac{1}{m_r}}\left[\Gamma_{\{\mathbf{S}|\boldsymbol{v}\}}(\mathbf{q})\right]^{rs}_{\alpha\beta}e^{i\mathbf{Sq}\cdot\mathbf{R}_m}\int_{\Omega}d\mathbf{r}'\,\varepsilon_e^{-1}(\mathbf{r},\mathbf{r}')\frac{\partial V_{rm}^{(0)}(\mathbf{r}'-\boldsymbol{\tau}_r-\mathbf{R}_m)}{\partial r'_\alpha} \\ &= \sum_{mr}\frac{\delta_{r,F_{\mathbf{S}}(s)}}{\sqrt{m_r}}e^{i\mathbf{Sq}\cdot[\mathbf{R}_m+\boldsymbol{\tau}_r-\{\mathbf{S}|\boldsymbol{v}\}\boldsymbol{\tau}_s]}\int_{\Omega}d\mathbf{r}'\,\varepsilon_e^{-1}(\mathbf{r},\mathbf{r}')\sum_{\alpha}S_{\alpha\beta}\left[\nabla_{\mathbf{r}'}V_{rm}^{(0)}(\mathbf{r}'-\boldsymbol{\tau}_r-\mathbf{R}_m)\right]_\alpha\,, \end{aligned} \tag{S.55}$$

where $\varepsilon_e^{-1}(\mathbf{r},\mathbf{r}') = \varepsilon_e^{-1}(\mathbf{r},\mathbf{r}';0)$ in the static electronic inverse dielectric function. In the second line, we use the inverse Bloch sum definition for the electron-nuclear potential, $V_r^{(0)\,\mathbf{q}}(\mathbf{r}) = \sum_m V_{rm}^{(0)}(\mathbf{r}-\boldsymbol{\tau}_r-\mathbf{R}_m)\exp(i\mathbf{q}\cdot\mathbf{R}_m)$, and in the third line, we recall the definition (S.52) for the transformation matrix $\boldsymbol{\Gamma}_{\{\mathbf{S}|\boldsymbol{v}\}}(\mathbf{q})$. Using the orthogonality property of the rotation matrix, we apply the identity $\mathbf{SqR}_m = \mathbf{qS}^{-1}\mathbf{R}_m$, which, combined with the change in the lattice vector reference frame $\mathbf{R}_m = \mathbf{SR}_l$, yields

$$\sum_{r\alpha}\sqrt{\tfrac{1}{m_r}}\left[\Gamma_{\{\mathbf{S}|\boldsymbol{v}\}}(\mathbf{q})\right]^{rs}_{\alpha\beta}\xi^{r\alpha}_{\mathbf{Sq}}(\mathbf{r}) = \sum_{lr}\frac{\delta_{r,F_{\mathbf{S}}(s)}}{\sqrt{m_r}}e^{i\mathbf{q}\cdot\mathbf{R}_l}e^{i\mathbf{Sq}\cdot[\boldsymbol{\tau}_r-\{\mathbf{S}|\boldsymbol{v}\}\boldsymbol{\tau}_s]}\int_{\Omega}d\mathbf{r}'\,\varepsilon_e^{-1}(\mathbf{r},\mathbf{r}')\sum_{\alpha}S_{\alpha\beta}\left[\nabla_{\mathbf{r}'}V_{rl}^{(0)}(\mathbf{r}'-\boldsymbol{\tau}_r-\mathbf{SR}_l)\right]_\alpha\,. \tag{S.56}$$

With $V_{rl}^{(0)}(\mathbf{r}'-\boldsymbol{\tau}_r-\mathbf{SR}_l) = -e^2Z_r|\mathbf{r}'-\boldsymbol{\tau}_r-\mathbf{SR}_l|^{-1}$ and knowing that the magnitude of a vector is rotationally invariant, we can write

$$|\mathbf{r}'-\boldsymbol{\tau}_r-\mathbf{SR}_l| = |\mathbf{S}(\mathbf{S}^{-1}\mathbf{r}'-\mathbf{S}^{-1}\boldsymbol{\tau}_r-\mathbf{R}_l)| = |\mathbf{S}^{-1}\mathbf{r}'-\mathbf{S}^{-1}\boldsymbol{\tau}_r-\mathbf{R}_l|\,, \tag{S.57}$$

By adding and subtracting the fractional translation $\boldsymbol{v}(\mathcal{S}^{-1})$, corresponding to the inverse rotation operator, along with the variable change $\mathbf{r}'' = \{\mathbf{S}|\boldsymbol{v}\}^{-1}\mathbf{r}'$ and the Jacobian $J_{\alpha\beta} = \left|\frac{\partial r'_\alpha}{\partial r''_\beta}\right| = |S_{\alpha\beta}| = 1$, we arrive from Eq. (S.56) to the

expression

$$\sum_{r\alpha}\sqrt{\tfrac{1}{m_r}}\big[\Gamma_{\{\mathbf{S}|\boldsymbol{v}\}}(\mathbf{q})\big]^{rs}_{\alpha\beta}\,\xi^{r\alpha}_{\mathbf{S}\mathbf{q}}(\mathbf{r}) = \sum_{lr}\frac{\delta_{r,F_{\mathbf{S}}(s)}}{\sqrt{m_r}}e^{i\mathbf{q}\cdot\mathbf{R}_l}e^{i\mathbf{S}\mathbf{q}\cdot[\boldsymbol{\tau}_r-\{\mathbf{S}|\boldsymbol{v}\}\boldsymbol{\tau}_s]}\times$$
$$\times\int_\Omega d\mathbf{r}''\,\varepsilon_e^{-1}(\mathbf{r},\{\mathbf{S}|\boldsymbol{v}\}\mathbf{r}'')\sum_{\alpha\gamma}S_{\alpha\beta}\left(\frac{\partial r''_\gamma}{\partial r'_\beta}\right)\big[\nabla_{\mathbf{r}'}V^{(0)}_{rl}(\mathbf{r}''-\{\mathbf{S}|\boldsymbol{v}\}^{-1}\boldsymbol{\tau}_r-\mathbf{R}_l)\big]_\gamma\,. \tag{S.58}$$

Using the inverse relation $\mathbf{r}''=\{\mathbf{S}|\boldsymbol{v}\}^{-1}\mathbf{r}'$, it is straightforward to compute the derivative $\frac{\partial r''_\gamma}{\partial r'_\beta}=S^{-1}_{\gamma\beta}$, resulting in

$$\begin{aligned}\sum_{\alpha\gamma}S_{\alpha\beta}\left(\frac{\partial r''_\gamma}{\partial r'_\beta}\right)\big[\nabla_{\mathbf{r}''}V^{(0)}_{rl}(\mathbf{r}''-\{\mathbf{S}|\boldsymbol{v}\}^{-1}\boldsymbol{\tau}_r-\mathbf{R}_l)\big]_\gamma &= \sum_\gamma\big[\nabla_{\mathbf{r}''}V^{(0)}_{rl}(\mathbf{r}''-\{\mathbf{S}|\boldsymbol{v}\}^{-1}\boldsymbol{\tau}_r-\mathbf{R}_l)\big]_\gamma\big(\mathbf{S}^{-1}\mathbf{S}\big)_{\gamma\beta}\\ &= \sum_\gamma\big[\nabla_{\mathbf{r}''}V^{(0)}_{rl}(\mathbf{r}''-\{\mathbf{S}|\boldsymbol{v}\}^{-1}\boldsymbol{\tau}_r-\mathbf{R}_l)\big]_\gamma\delta_{\gamma\beta}\\ &= \big[\nabla_{\mathbf{r}''}V^{(0)}_{rl}(\mathbf{r}''-\{\mathbf{S}|\boldsymbol{v}\}^{-1}\boldsymbol{\tau}_r-\mathbf{R}_l)\big]_\beta\,.\end{aligned} \tag{S.59}$$

The expression (S.58) can be further simplified by inverting Eq. (S.49)

$$\{\mathbf{S}|\boldsymbol{v}\}^{-1}\boldsymbol{\tau}_r=\mathcal{S}^{-1}\boldsymbol{\tau}_r-\bar{\boldsymbol{v}}_{\boldsymbol{\tau}_r}(\mathcal{S}^{-1})\,. \tag{S.60}$$

In this specific context, the electron-nuclear Coulomb interaction can be re-expressed as $V^{(0)}_{rl}(\mathbf{r}'-\{\mathbf{S}|\boldsymbol{v}\}^{-1}\boldsymbol{\tau}_r-\mathbf{R}_l)=V^{(0)}_{rl}[\mathbf{r}'-\mathcal{S}^{-1}\boldsymbol{\tau}_r-(\mathbf{R}_l-\bar{\boldsymbol{v}}_{\boldsymbol{\tau}_r}(\mathcal{S}^{-1}))]$. Since $\bar{\boldsymbol{v}}_{\boldsymbol{\tau}_r}(\mathcal{S}^{-1})$ is any possible lattice translation, we can define a new lattice reference frame via $\mathbf{R}_l-\bar{\boldsymbol{v}}_{\boldsymbol{\tau}_r}(\mathcal{S}^{-1})\equiv\mathbf{R}_n$. This results in

$$\sum_{r\alpha}\sqrt{\tfrac{1}{m_r}}\big[\Gamma_{\{\mathbf{S}|\boldsymbol{v}\}}(\mathbf{q})\big]^{rs}_{\alpha\beta}\,\xi^{r\alpha}_{\mathbf{S}\mathbf{q}}(\mathbf{r}) = \sum_{r\,n}\frac{\delta_{r,F_{\mathbf{S}}(s)}}{\sqrt{m_r}}e^{i\mathbf{q}\cdot\mathbf{R}_n}e^{i\mathbf{q}\cdot\bar{\boldsymbol{v}}_{\boldsymbol{\tau}_r}(\mathcal{S}^{-1})}e^{i\mathbf{S}\mathbf{q}\cdot[\boldsymbol{\tau}_r-\{\mathbf{S}|\boldsymbol{v}\}\boldsymbol{\tau}_s]}\times$$
$$\times\int_\Omega d\mathbf{r}'\,\varepsilon_e^{-1}(\mathbf{r},\{\mathbf{S}|\boldsymbol{v}\}\mathbf{r}')\frac{\partial V^{(0)}_{rn}(\mathbf{r}'-\mathcal{S}^{-1}\boldsymbol{\tau}_r-\mathbf{R}_n)}{\partial r'_\beta}\,, \tag{S.61}$$

where the equality (S.59) has been used. The phase factors in this expression can be simplified by using the identity [6]

$$\bar{\boldsymbol{v}}_{\boldsymbol{\tau}_r}(\mathcal{S}^{-1})=-\mathbf{S}^{-1}\bar{\boldsymbol{v}}_{\mathcal{S}^{-1}\boldsymbol{\tau}_r}(\mathcal{S})\,, \tag{S.62}$$

which yields

$$e^{i\mathbf{q}\cdot\bar{\boldsymbol{v}}_{\boldsymbol{\tau}_r}(\mathcal{S}^{-1})}e^{i\mathbf{S}\mathbf{q}\cdot[\boldsymbol{\tau}_r-\{\mathbf{S}|\boldsymbol{v}\}\boldsymbol{\tau}_s]}=e^{i\mathbf{S}\mathbf{q}\cdot[-\bar{\boldsymbol{v}}_{\mathcal{S}^{-1}\boldsymbol{\tau}_r}(\mathcal{S})+\boldsymbol{\tau}_r-\{\mathbf{S}|\boldsymbol{v}\}\boldsymbol{\tau}_s]}\,. \tag{S.63}$$

By applying the definition (S.49) under the condition $\boldsymbol{\tau}_s=\mathcal{S}^{-1}\boldsymbol{\tau}_r$,

$$\bar{\boldsymbol{v}}_{\mathcal{S}^{-1}\boldsymbol{\tau}_r}(\mathcal{S})=\boldsymbol{\tau}_r-\{\mathbf{S}|\boldsymbol{v}\}\mathcal{S}^{-1}\boldsymbol{\tau}_r\,, \tag{S.64}$$

Eq. (S.61) becomes

$$\sum_{r\alpha}\sqrt{\tfrac{1}{m_r}}\big[\Gamma_{\{\mathbf{S}|\boldsymbol{v}\}}(\mathbf{q})\big]^{rs}_{\alpha\beta}\,\xi^{r\alpha}_{\mathbf{S}\mathbf{q}}(\mathbf{r}) = \sum_{r\,n}\frac{\delta_{r,F_{\mathbf{S}}(s)}}{\sqrt{m_r}}e^{i\mathbf{q}\cdot\mathbf{R}_n}e^{i\mathbf{S}\mathbf{q}\cdot\{\mathbf{S}|\boldsymbol{v}\}[\mathcal{S}^{-1}\boldsymbol{\tau}_r-\boldsymbol{\tau}_s]}\times$$
$$\times\int_\Omega d\mathbf{r}'\,\varepsilon_e^{-1}(\mathbf{r},\{\mathbf{S}|\boldsymbol{v}\}\mathbf{r}')\frac{\partial V^{(0)}_{rn}(\mathbf{r}'-\mathcal{S}^{-1}\boldsymbol{\tau}_r-\mathbf{R}_n)}{\partial r'_\beta}\,. \tag{S.65}$$

Finally, using $\mathcal{S}^{-1}\boldsymbol{\tau}_r=\boldsymbol{\tau}_s$ when $\delta_{r,F_{\mathbf{S}}(s)}=1$, the expression simplifies further to

$$\begin{aligned}\sum_{r\alpha}\sqrt{\tfrac{1}{m_r}}\big[\Gamma_{\{\mathbf{S}|\boldsymbol{v}\}}(\mathbf{q})\big]^{rs}_{\alpha\beta}\,\xi^{r\alpha}_{\mathbf{S}\mathbf{q}}(\mathbf{r}) &= \sqrt{\tfrac{1}{m_s}}\sum_n e^{i\mathbf{q}\cdot\mathbf{R}_n}\int_\Omega d\mathbf{r}'\,\varepsilon_e^{-1}(\mathbf{r},\{\mathbf{S}|v\}\mathbf{r}')\frac{\partial V^{(0)}_{sn}(\mathbf{r}'-\boldsymbol{\tau}_s-\mathbf{R}_n)}{\partial r'_\beta}\\ &= \sqrt{\tfrac{1}{m_s}}\int_\Omega d\mathbf{r}'\,\varepsilon_e^{-1}(\mathbf{r},\{\mathbf{S}|v\}\mathbf{r}')\frac{\partial V^{(0)\,\mathbf{q}}_s(\mathbf{r}')}{\partial r'_\beta}\,.\end{aligned} \tag{S.66}$$

With the invariance of the inverse dielectric function under rotation, expressed as $\varepsilon_e^{-1}(\{\mathbf{S}|\boldsymbol{v}\}\mathbf{r},\{\mathbf{S}|\boldsymbol{v}\}\mathbf{r}')=\varepsilon_e^{-1}(\mathbf{r},\mathbf{r}')$, we deduce

$$\begin{aligned}\varepsilon_e^{-1}(\{\mathbf{S}|\boldsymbol{v}\}\{\mathbf{S}|\boldsymbol{v}\}^{-1}\mathbf{r},\{\mathbf{S}|\boldsymbol{v}\}\mathbf{r}') &= \varepsilon_e^{-1}(\{\mathbf{S}|\boldsymbol{v}\}^{-1}\mathbf{r},\mathbf{r}')\\ &= \varepsilon_e^{-1}(\mathbf{r},\{\mathbf{S}|\boldsymbol{v}\}\mathbf{r}')\,.\end{aligned} \tag{S.67}$$

Using this, we can rewrite Eq. (S.66) as

$$\begin{aligned}\sum_{r\alpha}\sqrt{\tfrac{1}{m_r}}\left[\Gamma_{\{\mathbf{S}|\boldsymbol{v}\}}(\mathbf{q})\right]^{rs}_{\alpha\beta}\xi^{r\alpha}_{\mathbf{Sq}}(\mathbf{r}) &= \sqrt{\tfrac{1}{m_s}}\int_\Omega d\mathbf{r}''\,\varepsilon_e^{-1}(\{\mathbf{S}|\boldsymbol{v}\}^{-1}\mathbf{r},\mathbf{r}')\frac{\partial V_s^{(0)\,\mathbf{q}}(\mathbf{r}')}{\partial r'_\beta}\\ &= \sqrt{\tfrac{1}{m_s}}\,\xi^{s\beta}_{\mathbf{q}}(\{\mathbf{S}|\boldsymbol{v}\}^{-1}\mathbf{r})\,.\end{aligned} \tag{S.68}$$

Next, applying this result allows us to rewrite Eq. (S.54) as

$$\begin{aligned}g_{in,\nu}(\mathbf{k},\mathbf{Sq}) &= \sum_{s\beta}\sqrt{\frac{\hbar}{2m_s\omega_{\mathbf{q}\nu}}}e_{s\beta,\nu}(\mathbf{q})\int_{\Omega_0}d\mathbf{r}\,\psi^*_{i,\mathbf{k}+\mathbf{Sq}}(\mathbf{r})\,\xi^{s\beta}_{\mathbf{q}}(\{\mathbf{S}|\boldsymbol{v}\}^{-1}\mathbf{r})\psi_{n,\mathbf{k}}(\mathbf{r})\\ &= \sum_{s\beta}\sqrt{\frac{\hbar}{2m_s\omega_{\mathbf{q}\nu}}}e_{s\beta,\nu}(\mathbf{q})\int_{\Omega_0}d\mathbf{r}'\,\psi^*_{i,\mathbf{k}+\mathbf{Sq}}(\{\mathbf{S}|\boldsymbol{v}\}\mathbf{r}')\,\xi^{s\beta}_{\mathbf{q}}(\mathbf{r}')\psi_{n,\mathbf{k}}(\{\mathbf{S}|\boldsymbol{v}\}\mathbf{r}')\,,\end{aligned} \tag{S.69}$$

where we considered the change of variable $\{\mathbf{S}|\boldsymbol{v}\}^{-1}\mathbf{r}=\mathbf{r}'$. Finally, employing the identity

$$\psi_{n,\mathbf{k}}(\{\mathbf{S}|\boldsymbol{v}\}\mathbf{r}')=\psi_{n,\mathbf{S}^{-1}\mathbf{k}}(\mathbf{r}')\,, \tag{S.70}$$

the rotated *e-ph* coupling matrix element can be evaluated using

$$\begin{aligned}g_{in,\nu}(\mathbf{k},\mathbf{Sq}) &= \sum_{r\alpha}\sqrt{\frac{\hbar}{2m_r\omega_{\mathbf{q}\nu}}}e_{r\alpha,\nu}(\mathbf{q})\,\langle\psi_{i,\mathbf{S}^{-1}\mathbf{k}+\mathbf{q}}|\,\xi^{r\alpha}_{\mathbf{q}}\,|\psi_{n,\mathbf{S}^{-1}\mathbf{k}}\rangle_{\Omega_0}\\ &= \langle\psi_{i,\mathbf{S}^{-1}\mathbf{k}+\mathbf{q}}|\,g_{\mathbf{q}\nu}\,|\psi_{n,\mathbf{S}^{-1}\mathbf{k}}\rangle_{\Omega_0}\end{aligned} \tag{S.71}$$

Here, we recognize an expression for the rotation of the *e-ph* coupling matrix element over the full electronic BZ **k**-mesh, in a form analogous to Eq. (S.71)

$$g_{in,\nu}(\mathbf{Sk},\mathbf{q})=\langle\psi_{i,\mathbf{Sk}+\mathbf{q}}|\,g_{\mathbf{q}\nu}\,|\psi_{n,\mathbf{Sk}}\rangle_{\Omega_0}\,, \tag{S.72}$$

from which we obtain a formula for rotating the *e-ph* matrix elements from the irreducible set of phonon wave vectors to the full BZ set

$$\boxed{g_{in,\nu}(\mathbf{k},\mathbf{Sq})=g_{in,\nu}(\mathbf{S}^{-1}\mathbf{k},\mathbf{q})}\,. \tag{S.73}$$

## S.3. TRANSFORMATION RULES FOR THE COEFFICIENTS $G^{\mathbf{q}}_{I\nu}$ UNDER ROTATION OF THE PHONON WAVE VECTORS

In the main text, we demonstrated that the *e-ph* matrix elements can alternately be reformulated using an expansion with projection coefficients expressed in terms of the biorthogonal MPB functions, $\{M^{\mathbf{q}}_I\}$,

$$g_{in,\nu}(\mathbf{k},\mathbf{q})=\sum_I G^{\mathbf{q}}_{I\nu}\,\langle\psi_{i,\mathbf{k}+\mathbf{q}}|\,\psi_{n,\mathbf{k}}M^{\mathbf{q}}_I\rangle_{\Omega_0}\,, \tag{S.74}$$

where the coefficients $G^{\mathbf{q}}_{I\nu}$ are defined as

$$G^{\mathbf{q}}_{I\nu}=\sum_J\bar{\varepsilon}^{-1}_{e,IJ}(\mathbf{q})\Pi^{\mathbf{q}}_{J\nu}\,. \tag{S.75}$$

with

$$\begin{aligned}\Pi^{\mathbf{q}}_{J\nu} &= \sum_{r\alpha}\sqrt{\frac{\hbar}{2m_r\omega_{\mathbf{q}\nu}}}e_{r\alpha,\nu}(\mathbf{q})\times\\ &\qquad\times\int_{\Omega_0}d\mathbf{r}\,M^{\mathbf{q}\,*}_J(\mathbf{r})\frac{\partial V_r^{(0)\,\mathbf{q}}(\mathbf{r})}{\partial r_\alpha},\end{aligned} \tag{S.76}$$

and

$$\bar{\varepsilon}^{-1}_{e,IJ}(\mathbf{q}) = \left(\mathbf{O}^{\mathbf{q}\,-1}\boldsymbol{\varepsilon}^{-1}_{e,\mathrm{M}}\right)_{IJ}$$
$$= \frac{1}{N_{\mathbf{k}}\Omega_0}\int_\Omega\int_\Omega d\mathbf{r}\,d\mathbf{r}'\widetilde{M}^{\mathbf{q}\,*}_I(\mathbf{r})\varepsilon^{-1}_e(\mathbf{r},\mathbf{r}';0)\widetilde{M}^{\mathbf{q}}_J(\mathbf{r}') \quad (S.77)$$

In this section, we aim to derive an expression for the coefficients $\Pi^{\mathbf{q}}_{J\nu}$ under a rotation applied to phonon wave vectors $\mathbf{Sq}$

$$\Pi^{\mathbf{Sq}}_{J\nu} = \sum_{r\alpha}\sqrt{\frac{\hbar}{2m_r\omega_{\mathbf{q}\nu}}}e_{r\alpha,\nu}(\mathbf{Sq})\times$$
$$\times\int_{\Omega_0} d\mathbf{r}\,M^{\mathbf{Sq}\,*}_J(\mathbf{r})\frac{\partial V^{(0)\,\mathbf{Sq}}_r(\mathbf{r})}{\partial r_\alpha}, \quad (S.78)$$

where we incorporate the rotational invariance of the phonon frequencies, i.e., $\omega_{\mathbf{Sq}\nu} = \omega_{\mathbf{q}\nu}$. The transformation law for the eigenmodes is governed by Eqs. (S.51) and (S.52). Following the procedure outlined in Sec. S.2, we proceed with an analytical derivation to obtain an explicit expression for evaluating Eq. (S.78). Combining Eqs. (S.78) and (S.52) yields

$$\Pi^{\mathbf{Sq}}_{J\nu} = \sum_{sl\beta}\sqrt{\frac{\hbar}{2\omega_{\mathbf{q}\nu}}}e_{s\beta,\nu}(\mathbf{q})\sum_r\frac{\delta_{r,F_{\mathbf{S}}(s)}}{\sqrt{m_r}}e^{i\mathbf{Sq}\cdot\mathbf{R}_l}\times$$
$$\times e^{i\mathbf{Sq}\cdot[\boldsymbol{\tau}_r-\{\mathbf{S}|\boldsymbol{v}\}\boldsymbol{\tau}_s]}\int_\Omega d\mathbf{r}\,M^{\mathbf{Sq}\,*}_J(\mathbf{r})\sum_\alpha S_{\alpha\beta}\left[\nabla_{\mathbf{r}}V^{(0)}_{rl}(\mathbf{r})\right]_\alpha \quad (S.79)$$

We isolate the quantity

$$\sum_l e^{i\mathbf{Sq}\cdot\mathbf{R}_l}\int_\Omega d\mathbf{r}\,M^{\mathbf{Sq}\,*}_J(\mathbf{r})\sum_\alpha S_{\alpha\beta}\left[\nabla_{\mathbf{r}}V^{(0)}_{rl}(\mathbf{r})\right]_\alpha,$$

where the gradient of the rotationally invariant potential $V^{(0)}_{rl}$ will be rotated from direction $\alpha$ to direction $\beta$ due to the rotation operator $\mathbf{S}$. Furthermore, by rewriting the argument of the phase factor as $\mathbf{SqR}_l = \mathbf{qS}^{-1}\mathbf{R}_l = \mathbf{qR}_m$ and $\mathbf{R}_l = \mathbf{SR}_m$ we can express the above term as

$$\sum_m e^{i\mathbf{q}\cdot\mathbf{R}_m}\int_\Omega d\mathbf{r}\,M^{\mathbf{Sq}\,*}_J(\mathbf{r})\frac{\partial V^{(0)}_{rm}(\mathbf{r}-\boldsymbol{\tau}_r-\mathbf{SR}_m)}{\partial r_\beta}. \quad (S.80)$$

Using the fact that the modulus of a vector is rotationally invariant, we can rewrite the inverse of the Coulomb kernel as

$$|\mathbf{r}-\boldsymbol{\tau}_r-\mathbf{SR}_m| = |\mathbf{S}(\{\mathbf{S}|\boldsymbol{v}\}^{-1}\mathbf{r}-\{\mathbf{S}|\boldsymbol{v}\}^{-1}\boldsymbol{\tau}_r-\mathbf{R}_m)|$$
$$= |\{\mathbf{S}|\boldsymbol{v}\}^{-1}\mathbf{r}-\{\mathbf{S}|\boldsymbol{v}\}^{-1}\boldsymbol{\tau}_r-\mathbf{R}_m|$$
$$= |\{\mathbf{S}|\boldsymbol{v}\}^{-1}\mathbf{r}-\mathcal{S}^{-1}\boldsymbol{\tau}_r-[\mathbf{R}_m-\bar{\boldsymbol{v}}_{\boldsymbol{\tau}_r}(\mathcal{S}^{-1})]|. \quad (S.81)$$

In the first line we added and subtracted the fractional translation $\boldsymbol{v}(\mathcal{S})$, and in the third line, we obtained the result by using the definition (S.49) for the translation vectors $\bar{\boldsymbol{v}}_{\boldsymbol{\tau}_r}(\mathcal{S}^{-1})$. Inserting this result into Eq. (S.80) and setting $\mathbf{R}_n = \mathbf{R}_m - \bar{\boldsymbol{v}}_{\boldsymbol{\tau}_r}(\mathcal{S}^{-1})$, where $\bar{\boldsymbol{v}}_{\boldsymbol{\tau}_r}$ is generally a lattice vector, we obtain

$$\sum_n e^{i\mathbf{q}\cdot\mathbf{R}_n}e^{-i\mathbf{Sq}\cdot\bar{\boldsymbol{v}}_{\mathcal{S}^{-1}\boldsymbol{\tau}_r}(\mathcal{S})}\times$$
$$\times\int_\Omega d\mathbf{r}\,M^{\mathbf{Sq}\,*}_J(\mathbf{r})\frac{\partial V^{(0)}_{rn}(\{\mathbf{S}|\boldsymbol{v}\}^{-1}\mathbf{r}-\mathcal{S}^{-1}\boldsymbol{\tau}_r-\mathbf{R}_n)}{\partial r_\beta}. \quad (S.82)$$

Here, we used the relation $\bar{\boldsymbol{v}}_{\boldsymbol{\tau}_r}(\mathcal{S}^{-1}) = -\mathbf{S}^{-1}\bar{\boldsymbol{v}}_{\mathcal{S}^{-1}\boldsymbol{\tau}_r}(\mathcal{S})$. The condition $\delta_{r,F_{\mathcal{S}}(s)} = 1$ is fulfilled only when $\mathcal{S}\boldsymbol{\tau}_s = \boldsymbol{\tau}_r$. Using this relation along with the definition (S.53) for the translation vector $\bar{\boldsymbol{v}}_{\mathcal{S}^{-1}\boldsymbol{\tau}_r}(\mathcal{S})$, Eq. (S.79) can be simplified as

$$\Pi^{\mathbf{Sq}}_{J\nu} = \sum_{s\beta}\sqrt{\frac{\hbar}{2m_s\omega_{\mathbf{q}\nu}}}e_{s\beta,\nu}(\mathbf{q})\times$$
$$\times\int_{\Omega_0} d\mathbf{r}\,M^{\mathbf{Sq}\,*}_J(\mathbf{r})\frac{\partial V^{(0)\,\mathbf{q}}_s(\{\mathbf{S}|\boldsymbol{v}\}^{-1}\mathbf{r})}{\partial r_\beta} \quad (S.83)$$

In both Eqs. (S.75) and (S.74), we are summing over interstitial $\{P^{\mathbf{q}}_{\mathbf{G}}\}$ and atomic sphere $\{B^{\mathbf{q}}_{\boldsymbol{\tau}alm}\}$ MPB functions. Therefore, it is meaningful to separate the analysis of the expansion coefficients (S.75) and of the *e-ph* matrix elements into their interstitial (*ipw*) and augmentation (*aug*) contributions, respectively. Specifically, we can express the *e-ph* matrix elements as

$$g_{in,\nu}(\mathbf{k},\mathbf{Sq}) = g^{ipw}_{in,\nu}(\mathbf{k},\mathbf{Sq}) + g^{aug}_{in,\nu}(\mathbf{k},\mathbf{Sq}) \quad (S.84)$$

The transformation rules for the biorthogonal MPB functions $M^{\mathbf{Sq}}_J$ differ for the interstitial and augmentation regions. Under the rotation of the wave vectors they transform as [7]

$$P^{\mathbf{Sq}}_{\mathbf{G}}(\mathbf{r}) = e^{i(\mathbf{Sq}+\mathbf{G})\cdot\boldsymbol{v}(\mathcal{S})}P^{\mathbf{q}}_{\mathbf{S}^{-1}\mathbf{G}}(\{\mathbf{S}|\boldsymbol{v}\}^{-1}\mathbf{r}) \quad (S.85)$$

and

$$B^{\mathbf{Sq}}_{\boldsymbol{\tau}alm}(\mathbf{r}) = e^{-i\mathbf{Sq}\cdot\bar{\boldsymbol{v}}_{\mathcal{S}^{-1}\boldsymbol{\tau}}(\mathcal{S})}\times$$
$$\times\sum_\mu\widetilde{D}^l_{\mu m}(\mathcal{S})B^{\mathbf{q}}_{\mathcal{S}^{-1}\boldsymbol{\tau}al\mu}(\{\mathbf{S}|\boldsymbol{v}\}^{-1}\mathbf{r}), \quad (S.86)$$

where $\widetilde{D}^l_{\mu m}(\mathcal{S})$ denotes the matrix element of the Wigner $\widetilde{D}$-matrix $\widetilde{\mathbf{D}}^l(\mathcal{S})$, which governs the rotation of real spherical harmonics according to

$$Y_{lm}(\widehat{\mathbf{Sr}}) = \sum_{\mu=-l}^{l}\widetilde{D}^l_{\mu m}(\mathcal{S})Y_{l\mu}(\widehat{\mathbf{r}}). \quad (S.87)$$

These matrices satisfy the orthonormality condition $\widetilde{\mathbf{D}}^l(\mathcal{S})\widetilde{\mathbf{D}}^{l\,T}(\mathcal{S}) = \mathbf{1}$. Note that the transformation rules (S.85) and (S.86) also apply to the set of MPB functions $\{\widetilde{M}^{\mathbf{Sq}}_J\}$.

### 1. Transformation rules in the interstitial region

In this section we examine the transformation rules for the coefficients $\Pi^{\mathbf{Sq}}_{\mathbf{G}\nu}$, $G^{\mathbf{Sq}}_{\mathbf{G}\nu}$, and of $g^{ipw}_{in,\nu}(\mathbf{k},\mathbf{Sq})$ within the interstitial region. Making use of the property (S.85) in Eq. (S.83) and using a change of variable $\mathbf{r}' = \{\mathbf{S}|\boldsymbol{v}\}^{-1}\mathbf{r}$ in the integral, we obtain

$$\Pi^{\mathbf{Sq}}_{\mathbf{G}',\nu} = e^{-i(\mathbf{Sq}+\mathbf{G}')\cdot\boldsymbol{v}(\mathcal{S})}\Pi^{\mathbf{q}}_{\mathbf{S}^{-1}\mathbf{G}',\nu}\,. \tag{S.88}$$

Regarding the Fourier component $\bar{\varepsilon}^{-1}_{e,\mathbf{GG}'}$ of the inverse dielectric function, the transformation rule under rotated phonon momentum transfer $\mathbf{Sq}$ can be straightforwardly derived again by using Eq. (S.85),

$$\bar{\varepsilon}^{-1}_{e,\mathbf{GG}'}(\mathbf{Sq}) = e^{-i(\mathbf{G}-\mathbf{G}')\boldsymbol{v}(\mathcal{S})}\bar{\varepsilon}^{-1}_{e,\mathbf{S}^{-1}\mathbf{G}\,\mathbf{S}^{-1}\mathbf{G}'}(\mathbf{q})\,. \tag{S.89}$$

By combining Eqs. (S.75), (S.88), and (S.89) we arrive at

$$G^{\mathbf{Sq}}_{\mathbf{G},\nu} = e^{-i(\mathbf{Sq}+\mathbf{G})\boldsymbol{v}(\mathcal{S})}G^{\mathbf{q}}_{\mathbf{S}^{-1}\mathbf{G},\nu}\,. \tag{S.90}$$

Finally, upon inserting this result into Eq. (S.74), the *e-ph* matrix elements will transform as

$$g^{ipw}_{in,\nu}(\mathbf{k},\mathbf{Sq}) = \sum_{\mathbf{G}} G^{\mathbf{q}}_{\mathbf{S}^{-1}\mathbf{G},\nu}\times \times\left(e^{-i(\mathbf{Sq}+\mathbf{G})\cdot\boldsymbol{v}(\mathcal{S})}\,\langle\psi_{i,\mathbf{k}+\mathbf{Sq}}|\,\psi_{n,\mathbf{k}}P^{\mathbf{Sq}}_{\mathbf{G}}\rangle_{\Omega_0}\right), \tag{S.91}$$

where the quantity within brackets represents the transformation rule for the projection coefficients as implemented in the `Questaal` code

$$e^{-i(\mathbf{Sq}+\mathbf{G})\cdot\boldsymbol{v}(\mathcal{S})}\,\langle\psi_{i,\mathbf{k}+\mathbf{Sq}}|\,\psi_{n,\mathbf{k}}P^{\mathbf{Sq}}_{\mathbf{G}}\rangle_{\Omega_0} = = \langle\psi_{i,\mathbf{S}^{-1}\mathbf{k}+\mathbf{q}}|\,\psi_{n,\mathbf{S}^{-1}\mathbf{k}}P^{\mathbf{q}}_{\mathbf{S}^{-1}\mathbf{G}}\rangle_{\Omega_0}. \tag{S.92}$$

*Our algorithm does not require evaluating the projection coefficients for rotated electronic wave vectors* $\mathbf{S}^{-1}\mathbf{k}$—the left hand side of Eq. (S.92) is instead calculated—*and can be easily extended to electronic wave vectors that do not belong to the BZ mesh.* Carrying out the replacement $\mathbf{S}^{-1}\mathbf{G}\to\mathbf{G}$, which keeps the summation over reciprocal lattice vectors invariant, we obtain

$$g^{ipw}_{in,\nu}(\mathbf{k},\mathbf{Sq}) = \sum_{\mathbf{G}} G^{\mathbf{q}}_{\mathbf{G},\nu}\,\langle\psi_{i,\mathbf{S}^{-1}\mathbf{k}+\mathbf{q}}|\,\psi_{n,\mathbf{S}^{-1}\mathbf{k}}P^{\mathbf{q}}_{\mathbf{G}}\rangle_{\Omega_0}\,. \tag{S.93}$$

This expression can be rewritten as $g^{ipw}_{in,\nu}(\mathbf{k},\mathbf{Sq}) = g^{ipw}_{in,\nu}(\mathbf{S}^{-1}\mathbf{k},\mathbf{q})$, reminiscent of the identity (S.73).

### 2. Transformation rules in the augmentation region

In this section we examine the transformation rules for the coefficients $\Pi^{\mathbf{Sq}}_{\boldsymbol{\tau}alm,\nu}$, $G^{\mathbf{Sq}}_{\boldsymbol{\tau}alm,\nu}$, and of $g^{aug}_{in,\nu}(\mathbf{k},\mathbf{Sq})$ within the augmentation region. Making use of rule (S.86) in Eq. (S.83) we obtain

$$\Pi^{\mathbf{Sq}}_{\boldsymbol{\tau}'a'l'm',\nu} = e^{i\mathbf{Sq}\cdot\bar{\boldsymbol{v}}_{\mathcal{S}^{-1}\boldsymbol{\tau}'}(\mathcal{S})}\sum_{\mu}\widetilde{D}^{l'}_{\mu m'}(\mathcal{S})\,\Pi^{\mathbf{q}}_{\mathcal{S}^{-1}\boldsymbol{\tau}'a'l'\mu,\nu}\,. \tag{S.94}$$

The matrix elements $\bar{\varepsilon}^{-1}_{e,\boldsymbol{\tau}alm,\boldsymbol{\tau}'a'l'm'}$ will then transform as

$$\bar{\varepsilon}^{-1}_{e,\boldsymbol{\tau}alm,\boldsymbol{\tau}'a'l'm'}(\mathbf{Sq}) = e^{i\mathbf{Sq}(\bar{\boldsymbol{v}}_{\mathcal{S}^{-1}\boldsymbol{\tau}}(\mathcal{S})-\bar{\boldsymbol{v}}_{\mathcal{S}^{-1}\boldsymbol{\tau}'}(\mathcal{S}))}\times \times\widetilde{D}^{l}_{\eta m}(\mathcal{S})\widetilde{D}^{l'}_{\eta' m'}(\mathcal{S})\,\bar{\varepsilon}^{-1}_{e,\mathcal{S}^{-1}\boldsymbol{\tau}al\eta,\mathcal{S}^{-1}\boldsymbol{\tau}'a'l'\eta'}(\mathbf{q}). \tag{S.95}$$

By combining Eqs. (S.75), (S.94), and (S.95) we arrive at

$$G^{\mathbf{Sq}}_{\boldsymbol{\tau}alm,\nu} = e^{i\mathbf{Sq}\cdot\bar{\boldsymbol{v}}_{\mathcal{S}^{-1}\boldsymbol{\tau}}(\mathcal{S})}\sum_{\eta}\widetilde{D}^{l}_{\eta m}(\mathcal{S})\,G^{\mathbf{q}}_{\mathcal{S}^{-1}\boldsymbol{\tau}al\eta,\nu}\,. \tag{S.96}$$

Finally, upon inserting Eq. (S.96) into Eq. (S.74), the *e-ph* matrix elements in the augmentation region will transform as

$$g^{aug}_{in,\nu}(\mathbf{k},\mathbf{Sq}) = \sum_{\boldsymbol{\tau}al\eta} G^{\mathbf{q}}_{\boldsymbol{\tau}al\eta,\nu}\times \times\left(e^{i\mathbf{Sq}\cdot\bar{\boldsymbol{v}}_{\boldsymbol{\tau}}(\mathcal{S})}\sum_{m}\widetilde{D}^{l}_{\eta m}(\mathcal{S})\,\langle\psi_{i,\mathbf{k}+\mathbf{Sq}}|\,\psi_{n,\mathbf{k}}B^{\mathbf{Sq}}_{\mathcal{S}\boldsymbol{\tau}alm}\rangle_{\Omega_0}\right). \tag{S.97}$$

with the quantity in brackets representing the transformation rule for the projection coefficients as implemented in the `Questaal` code

$$e^{i\mathbf{Sq}\cdot\bar{\boldsymbol{v}}_{\boldsymbol{\tau}}(\mathcal{S})}\sum_{m}\widetilde{D}^{l}_{\eta m}(\mathcal{S})\,\langle\psi_{i,\mathbf{k}+\mathbf{Sq}}|\,\psi_{n,\mathbf{k}}B^{\mathbf{Sq}}_{\mathcal{S}\boldsymbol{\tau}alm}\rangle_{\Omega_0} = = \langle\psi_{i,\mathbf{S}^{-1}\mathbf{k}+\mathbf{q}}|\,\psi_{n,\mathbf{S}^{-1}\mathbf{k}}B^{\mathbf{q}}_{\boldsymbol{\tau}al\eta}\rangle_{\Omega_0}. \tag{S.98}$$

Again, by replacing this result into Eq. (S.97), we find an expression reminiscent of the identity (S.73)

$$g^{aug}_{in,\nu}(\mathbf{k},\mathbf{Sq}) = g^{aug}_{in,\nu}(\mathbf{S}^{-1}\mathbf{k},\mathbf{q}) = \sum_{\boldsymbol{\tau}al\eta} G^{\mathbf{q}}_{\boldsymbol{\tau}al\eta,\nu}\,\langle\psi_{i,\mathbf{S}^{-1}\mathbf{k}+\mathbf{q}}|\,\psi_{n,\mathbf{S}^{-1}\mathbf{k}}B^{\mathbf{q}}_{\boldsymbol{\tau}al\eta}\rangle_{\Omega_0}. \tag{S.99}$$

## S.4. SPHERICAL FUNCTIONS

### A. Spherical Bessel and Hankel functions: definitions and conventions

In polar coordinates, the Helmholtz equation for a free particle leads, for each integer value $l \geq 0$ of the orbital angular momentum, to the radial equation

$$\left[-\frac{d^2}{dr^2}-\frac{2}{r}\frac{d}{dr}+\frac{l(l+1)}{r^2}\right]f_l(r) = a^2 f_l(r) \tag{S.100}$$

known as *Bessel's differential equation*, with $a$ potentially a complex parameter. The spherical Bessel functions are

special solutions of this equation. We denote this solution as $j_l(ar)$, which is regular (behaving as $r^l$) at the origin and is referred to as the proper spherical Bessel function. Other solutions include the irregular solutions $n_l(ar)$ (the Neumann functions), $h_l^{(+)}(ar) = h_l(ar)$ (the Hankel function of the first kind), and $h_l^{(-)}(ar)$ (the Hankel function of the second kind). We focus on a detailed analysis of the proper spherical Bessel functions and Hankel functions of the first kind, as they are extensively used throughout this study. Proper spherical Bessel functions (from here on referred to as Bessel functions) are real solutions of Eq. (S.100), while the Hankel functions of the first kind (hereafter referred to simply as Hankel functions) are complex functions ($h_l^* = h_l^{(-)}$) and can be expressed in terms of the Bessel and Neumann functions as $h_l(ar) = j_l(ar) + i n_l(ar)$.

A power series expansion for the Bessel function is given by

$$j_l(ar) = a^l r^l \sum_{n=0}^{\infty} \frac{(-)^n a^{2n} r^{2n}}{2^n n!(2l+2n+1)!!} \,. \tag{S.101}$$

Similarly, the Hankel function can be expressed as

$$h_l(ar) = \frac{e^{iar}}{ar} \sum_{n=0}^{l} \frac{i^{n-l}(l+n)!}{2^n n!(l-n)!(ar)^n} \,. \tag{S.102}$$

Expressions (S.101) and (S.102) follow standard conventions. However, it is advantageous to adopt an alternative convention, introduced by Methfessel[1], to streamline the mathematical formalism of asymptotic expressions of both the Bessel and Hankel functions near the origin, especially in the expansion of the generalized Yukawa kernel $\exp(-ar)/r$ in spherical harmonics (as shown below) and in the *one-centre expansion* of the Hankel functions. Under the *Methfessel convention*, the Bessel and Hankel functions are defined as

$$j_l^m(ar) = \frac{j_l(ar)}{a^l} = r^l \sum_{n=0}^{\infty} \frac{(-)^n a^{2n} r^{2n}}{2^n n!(2l+2n+1)!!} \,, \tag{S.103}$$

$$h_l^m(ar) = a^{l+1} h_l(ar) = \frac{e^{iar}}{r} \sum_{n=0}^{l} \frac{i^{n-l}(l+n)! a^{l-n}}{2^n n!(l-n)! r^n} \,. \tag{S.104}$$

The parameter $a$ may be a complex number, and in this case, the spherical Bessel and Hankel functions are complex-valued functions. However, in case of purely imaginary parameters $a = i|\kappa|$, the Methfessel convention yields real spherical Bessel and Hankel functions

$$\begin{aligned} j_l^m(i|\kappa|r) &= r^l \sum_{n=0}^{\infty} \frac{(-)^n i^{2n} |\kappa|^{2n} r^{2n}}{2^n n!(2l+2n+1)!!} \\ &= r^l \sum_{n=0}^{\infty} \frac{|\kappa|^{2n} r^{2n}}{2^n n!(2l+2n+1)!!} \,, \end{aligned} \tag{S.105}$$

$$\begin{aligned} h_l^m(i|\kappa|r) &= \frac{e^{-|\kappa|r}}{r} \sum_{n=0}^{l} \frac{i^{n-l}(l+n)!(i|\kappa|)^{l-n}}{2^n n!(l-n)! r^n} \\ &= \frac{e^{-|\kappa|r}}{r} \sum_{n=0}^{l} \frac{(l+n)! |\kappa|^{l-n}}{2^n n!(l-n)! r^n} \,, \end{aligned} \tag{S.106}$$

where $(-)^n i^{2n} = (-)^{2n} = 1$. Thus, if $a = i|\kappa|$ both $j_l^m$ and $h_l^m$ are real-valued and positive defined functions. For real parameters $a$, the asymptotic $r \to 0$ limit of the Bessel and Hankel functions in the Methfessel convention are

$$\begin{aligned} j_l^m(ar) &= r^l \left[ \frac{1}{(2l+1)!!} + \sum_{n=1}^{\infty} \frac{(-)^n a^{2n} r^{2n}}{2^n n!(2l+2n+1)!!} \right] \\ &\xrightarrow[r \to 0]{} \frac{r^l}{(2l+1)!!} = \delta_{l0} \,, \end{aligned} \tag{S.107}$$

which is equal to 1 for $l = 0$ and vanishes for $l \geq 1$, and

$$\begin{aligned} h_l^m(ar) &= \frac{e^{iar}}{r} \left[ i^{-l} a^l + \cdots + \frac{(2l)!}{2^l l! r^l} \right] \\ &= e^{iar} \left[ \frac{i^{-l} a^l}{r} + \cdots + \frac{(2l-1)!!}{r^{l+1}} \right] \xrightarrow[r \to 0]{} \frac{(2l-1)!!}{r^{l+1}} \,, \end{aligned} \tag{S.108}$$

since the final term in the summation ($n = l$) is the leading diverging term, which diverges more rapidly than contributions with $n < l$. At the second line of Eq. (S.108) we used the identity $(2n)! = 2^n n!(2n-1)!!$.

As mentioned before, the Methfessel convention can be used to derive an expression for the spherical harmonics expansion of the generalized Yukawa kernel within a spherical symmetry

$$\frac{e^{-a|\mathbf{r}-\mathbf{r}'|}}{|\mathbf{r}-\mathbf{r}'|} \tag{S.109}$$

in the $a \to 0$ limit. The spherical harmonics expansion of the Coulomb kernel is given by

$$\frac{1}{|\mathbf{r}-\mathbf{r}'|} = \sum_{lm_l} \frac{4\pi}{2l+1} \frac{r_<^l}{r_>^{l+1}} Y_{lm_l}(\widehat{\mathbf{r}}) Y_{lm_l}(\widehat{\mathbf{r}}') \,, \tag{S.110}$$

with $Y_{lm_l}(\widehat{\mathbf{r}})$ a real spherical harmonic (see Sec. S.4 C). In this context, the generalized Yukawa kernel (S.109) can be expressed in terms of the Bessel and Hankel functions in the Methfessel convention

$$\frac{e^{-a|\mathbf{r}-\mathbf{r}'|}}{|\mathbf{r}-\mathbf{r}'|} = 4\pi \sum_{lm_l} j_l^m(ar_<) h_l^m(ar_>) Y_{lm_l}(\widehat{\mathbf{r}}) Y_{lm_l}(\widehat{\mathbf{r}}') \,, \tag{S.111}$$

as the asymptotic forms (S.107) and (S.108) allow us to recover the spherical harmonics expansion (S.110) in the $a \to 0$ limit

$$\begin{aligned} \frac{e^{-a|\mathbf{r}-\mathbf{r}'|}}{|\mathbf{r}-\mathbf{r}'|} &\xrightarrow[a \to 0]{} 4\pi \sum_{lm_l} \frac{(2l-1)!!}{(2l+1)!!} \frac{r_<^l}{r_>^{l+1}} Y_{lm_l}(\widehat{\mathbf{r}}) Y_{lm_l}(\widehat{\mathbf{r}}') \\ &= \sum_{lm_l} \frac{4\pi}{2l+1} \frac{r_<^l}{r_>^{l+1}} Y_{lm_l}(\widehat{\mathbf{r}}) Y_{lm_l}(\widehat{\mathbf{r}}'). \end{aligned} \tag{S.112}$$

Returning to the standard convention, the following expression is needed to expand the generalized Yukawa kernel

$$\frac{e^{-a|\mathbf{r}-\mathbf{r}'|}}{|\mathbf{r}-\mathbf{r}'|} = 4\pi a \sum_{lm_l} j_l(ar_<) h_l(ar_>) Y_{lm_l}(\widehat{\mathbf{r}}) Y_{lm_l}(\widehat{\mathbf{r}}') \,, \tag{S.113}$$

with numerical difficulties in the limit $a \to 0$ due to the divergence of the Hankel functions in this limit.

A key mathematical relation is the *one-centre expansion of the Hankel functions* $h_l(a|\mathbf{r}' + \boldsymbol{\tau}_s - \boldsymbol{\tau}_t|)$ with $s \neq t$, rewritten in the Methfessel convention as

$$h_l^m(a|\mathbf{r}' + \boldsymbol{\tau}_s - \boldsymbol{\tau}_t|) Y_{lm_l}\left(\frac{\mathbf{r}' + \boldsymbol{\tau}_s - \boldsymbol{\tau}_t}{|\mathbf{r}' + \boldsymbol{\tau}_s - \boldsymbol{\tau}_t|}\right) = \\ = \sum_{l'm_{l'}} j_{l'}^m(ar') Y_{l'm_{l'}}(\widehat{\mathbf{r}}') S_{\boldsymbol{\tau}_s l' m_{l'}}^{\boldsymbol{\tau}_t l m_l}(a; \boldsymbol{\tau}_s - \boldsymbol{\tau}_t), \tag{S.114}$$

where $S_{\boldsymbol{\tau}_s l' m_{l'}}^{\boldsymbol{\tau}_t l m_l}(a; \boldsymbol{\tau}_s - \boldsymbol{\tau}_t)$ is the *bare structure constant* (depending only on atomic positions, without contributions from atomic sphere potentials and radii) defined as

$$S_{\boldsymbol{\tau}_s l' m_{l'}}^{\boldsymbol{\tau}_t l m_l}(a; \boldsymbol{\tau}_s - \boldsymbol{\tau}_t) = 4\pi \sum_{l''m_{l''}} G_{l''m_{l''},l'm_{l'}}^{lm_l} \times \\ \times (-)^{l'} a^{l+l'-l''} h_{l''m_{l''}}^m(\boldsymbol{\tau}_s - \boldsymbol{\tau}_t) \tag{S.115}$$

with $G_{l''m_{l''},l'm_{l'}}^{lm_l}$ representing the Gaunt coefficients (introduced in Sec. S.4 B), $h_{l''m_{l''}}^m(\boldsymbol{\tau}_s - \boldsymbol{\tau}_t) = h_{l''}^m(a|\boldsymbol{\tau}_s - \boldsymbol{\tau}_t|) Y_{l''m_{l''}}(\widehat{\boldsymbol{\tau}_s - \boldsymbol{\tau}_t})$ the solid Hankel function, and the condition $|\boldsymbol{\tau}_s - \boldsymbol{\tau}_t| \gg r'$ assumed to validate the *addition theorem* for spherical functions.

### 1. Derivatives and some recursion relations

The derivative of the Bessel function with respect to the radial position in its standard convention is defined by the recursion relation

$$\frac{\partial}{\partial r} j_l(ar) = \frac{l}{r} j_l(ar) - a j_{l+1}(ar) \,, \tag{S.116}$$

while in the Methfessel convention

$$\begin{aligned} \frac{\partial}{\partial r} j_l^m(ar) &= \frac{l}{r} j_l^m(ar) + r^l \sum_{n=0}^{\infty} \frac{2n(-)^n a^{2n} r^{2n-1}}{2^n n!(2l+2n+1)!!} \\ &= \frac{l}{r} j_l^m(ar) + r^l \sum_{n=1}^{\infty} \frac{(-)^n a^{2n} r^{2n-1}}{2^{n-1}(n-1)!(2l+2n+1)!!} \\ &= \frac{l}{r} j_l^m(ar) + r^l \sum_{m=0}^{\infty} \frac{(-)^{m+1} a^{2m+2} r^{2m+1}}{2^m m![2(l+1)+2m+1]!!} \\ &= \frac{l}{r} j_l^m(ar) - a^2 j_{l+1}^m(ar) \,, \end{aligned} \tag{S.117}$$

where, at the third line, we set $m = n - 1$. Equation (S.117) also can be simply derived starting from Eq. (S.116) and passing to the Methfessel convention as follows

$$\begin{aligned} \frac{1}{a^l}\frac{\partial}{\partial r} j_l(ar) = \frac{\partial}{\partial r} j_l^m(ar) &= \frac{1}{a^l}\frac{l}{r} j_l(ar) - \frac{a}{a^l} j_{l+1}(ar) \\ &= \frac{l}{r} j_l^m(ar) - a^2 j_{l+1}^m(ar) \end{aligned} \tag{S.118}$$

Given that the spherical Hankel function of the first kind in the Methfessel convention is related to the *unsmoothed Hankel function* as

$$\begin{aligned} \check{H}_L(a\mathbf{r}) &= \mathscr{Y}_L(-\nabla)\check{h}(ar) \\ &= h_l^m(ar) Y_L(\widehat{\mathbf{r}}) = h_l^m(a\mathbf{r}) \,, \end{aligned} \tag{S.119}$$

with $\mathscr{Y}_L(-\nabla)$ denoting the spherical harmonics polynomial in the gradient components and $\check{h}(ar) = h_0^m(ar) = \exp(iar)/r$ the *unsmoothed Hankel root function*, the derivative of the Hankel function can be derived by the recurrence relation[1]

$$h_l^m(ar) = \left[-\frac{\partial}{\partial r} + \frac{l-1}{r}\right] h_{l-1}^m(ar) \quad \text{for} \quad l \geq 1 \,. \tag{S.120}$$

Thus, its derivate can be formulated as

$$\frac{\partial}{\partial r} h_l^m(ar) = \frac{l}{r} h_l^m(ar) - h_{l+1}^m(ar) \,. \tag{S.121}$$

Equations (S.117) and (S.121) are examples of recursion relations for Bessel and Hankel functions, respectively. Other useful recursion relations are[8]

$$j_{l+1}^m(ar) = \frac{2l+1}{a^2 r} j_l^m(ar) - \frac{j_{l-1}^m(ar)}{a^2} \,, \tag{S.122}$$

$$h_{l+1}^m(ar) = \frac{2l+1}{r} h_l^m(ar) - h_{l-1}^m(ar) \,. \tag{S.123}$$

### 2. Integrals of Lommel's type for spherical functions

In the following, we derive an analytic solution for the radial Lommel's type integral[9, 10]

$$\int_0^s dr r^2 j_l(ar) j_{l'}(br) \,, \tag{S.124}$$

where the integration is performed within an augmentation sphere of radius $s$. At the end of the derivation we will focus on the special case where $l = l'$. The derivation is performed in the standard convention, though it remains valid in the Methfessel convention. To proceed, we multiply the integral by $(a^2 - b^2)$ and rewrite it as

$$(a^2-b^2)\int_0^s drr^2 j_l(ar)j_{l'}(br) = \int_0^s drr^2\big[a^2 j_l(ar)\big]j_{l'}(br) - \int_0^s drr^2 j_l(ar)\big[b^2 j_{l'}(br)\big]\,. \tag{S.125}$$

Since Bessel functions are solutions of the Helmholtz equation (S.100), we can substitute their definition into the integral (S.125) to replace the terms $a^2 j_l(ar)$ and $b^2 j_{l'}(br)$. This yields

$$(a^2-b^2)\int_0^s drr^2 j_l(ar)j_{l'}(br) = \big[l(l+1)-l'(l'+1)\big]\int_0^s dr j_l(ar)j_{l'}(br) + \\ +\int_0^s drr^2\left(\frac{\partial^2}{\partial r^2}j_{l'}(br)\right)j_l(ar) - \int_0^s drr^2\left(\frac{\partial^2}{\partial r^2}j_l(ar)\right)j_{l'}(br) + \int_0^s drr\left(\frac{\partial}{\partial r}j_{l'}(br)\right)j_l(ar) - 2\int_0^s drr\left(\frac{\partial}{\partial r}j_l(ar)\right)j_{l'}(br) \tag{S.126}$$

By integrating by parts, e.g.,

$$\begin{aligned}\int_0^s drr^2\left(\frac{\partial^2}{\partial r^2}j_l(ar)\right)j_{l'}(br) &= \int_0^s drr^2\frac{\partial}{\partial r}\left(\frac{\partial}{\partial r}j_l(ar)\right)j_{l'}(br) \\ &= s^2\left(\frac{\partial}{\partial r}j_l(ar)\right)_{r=s} j_{l'}(bs) - \int_0^s dr\frac{\partial}{\partial r}\left(r^2 j_{l'}(br)\right)\frac{\partial}{\partial r}j_l(ar) \\ &= s^2\left(\frac{\partial}{\partial r}j_l(ar)\right)_{r=s} j_{l'}(bs) - 2\int_0^s drr j_{l'}(br)\frac{\partial}{\partial r}j_l(ar) - \int_0^s drr^2\frac{\partial}{\partial r}j_{l'}(br)\frac{\partial}{\partial r}j_l(ar)\end{aligned} \tag{S.127}$$

and simplifying, we obtain

$$\int_0^s drr^2 j_l(ar)j_{l'}(br) = \frac{s^2}{a^2-b^2}\left[\left(\frac{\partial}{\partial r}j_{l'}(br)\right)_{r=s} j_l(as) - j_{l'}(bs)\left(\frac{\partial}{\partial r}j_l(ar)\right)_{r=s}\right] + \\ + \frac{1}{a^2-b^2}\big[l(l+1)-l'(l'+1)\big]\int_0^s dr j_l(ar)j_{l'}(br)\,. \tag{S.128}$$

The integral $\int_0^s dr j_l(ar)j_{l'}(br)$ can be analytically solved in terms of hypergeometric functions only in the limit $s\to\infty$ or by using the power expansion (S.101). However, since the formalism only requires the case $l=l'$, we have

$$\int_0^s drr^2 j_l(ar)j_l(br) = \frac{s^2}{a^2-b^2}\left[\left(\frac{\partial}{\partial r}j_l(br)\right)_{r=s} j_l(as) - j_l(bs)\left(\frac{\partial}{\partial r}j_l(ar)\right)_{r=s}\right]. \tag{S.129}$$

Similarly, we obtain

$$\int_0^s drr^2 j_l(ar)h_l(br) = \frac{s^2}{a^2-b^2}\left[\left(\frac{\partial}{\partial r}h_l(br)\right)_{r=s} j_l(as) - h_l(bs)\left(\frac{\partial}{\partial r}j_l(ar)\right)_{r=s}\right], \tag{S.130}$$

$$\int_0^s drr^2 h_l(ar)h_l(br) = \frac{s^2}{a^2-b^2}\left[\left(\frac{\partial}{\partial r}h_l(br)\right)_{r=s} h_l(as) - h_l(bs)\left(\frac{\partial}{\partial r}h_l(ar)\right)_{r=s}\right]. \tag{S.131}$$

It should be noted that these analytical solutions cannot be evaluated using the asymptotic forms (S.107) and (S.108) in the $s\to 0$ limit, as these forms do not satisfy the Helmholtz equation in that regime.

For the case $a=b\neq 0$, the right-hand sides of Eqs. (S.129)-(S.131) become indeterminate. Applying L'Hôpital's theorem, we differentiate with respect to the parameter $a^2$ and obtain

$$\int_0^s drr^2 j_l^m(ar)j_l^m(ar) = s^2\left[\left(\frac{\partial}{\partial r}j_l^m(ar)\right)_{r=s}\frac{\partial}{\partial a^2}j_l^m(as) - j_l^m(as)\frac{\partial}{\partial a^2}\left(\frac{\partial}{\partial r}j_l^m(ar)\right)_{r=s}\right], \tag{S.132}$$

where the Methfessel convention is used to evaluate the integral, and the derivatives with respect to $a^2$ for the Bessel functions are given by

$$\frac{\partial}{\partial a^2}j_l^m(as) = -\frac{s}{2}j_{l+1}^m(as)\,, \qquad \frac{\partial}{\partial a^2}\left(\frac{\partial}{\partial r}j_l^m(ar)\right)_{r=s} = \frac{sa^2}{2}j_{l+2}^m(as) - \frac{l+2}{2}j_{l+1}^m(as)\,. \tag{S.133}$$

Similarly, we find

$$\int_0^s drr^2 h_l^m(ar)h_l^m(ar) = s^2\left[\left(\frac{\partial}{\partial r}h_l^m(ar)\right)_{r=s}\frac{\partial}{\partial a^2}h_l^m(as) - h_l^m(as)\frac{\partial}{\partial a^2}\left(\frac{\partial}{\partial r}h_l^m(ar)\right)_{r=s}\right]. \tag{S.134}$$

### B. Gaunt and Clebsch-Gordan coefficients

Let $|j_3 m_3\rangle$ be a set of coupled states resulting from the uncoupled states $|j_1 m_1\rangle$ and $|j_2 m_2\rangle$. By employing the completeness relation in the coupled basis, we obtain an important expansion known as the *Clebsch-Gordan series*

$$|j_1 m_1; j_2 m_2\rangle = \sum_{j_3 m_3} \langle j_3 m_3 \, | j_1 m_1; j_2 m_2\rangle \, |j_3 m_3\rangle \ , \tag{S.135}$$

where $\langle j_3 m_3 \, | j_1 m_1; j_2 m_2\rangle$ denotes the *Gaunt coefficients*. From Eq. (S.135), it follows that the Gaunt coefficients correspond to integrals of the product of three complex spherical harmonics, defined as in Eq. (S.158),

$$\langle j_3 m_3 \, | j_1 m_1; j_2 m_2\rangle = \int d\Omega \, Y_{j_3}^{m_3 *}(\widehat{\mathbf{r}}) Y_{j_1}^{m_1}(\widehat{\mathbf{r}}) Y_{j_2}^{m_2}(\widehat{\mathbf{r}}) \, , \tag{S.136}$$

with $\int d\Omega = \int_0^{2\pi} \int_0^{\pi} d\phi \, d\theta \sin\theta$. An important property of the Gaunt coefficients is given by

$$\langle j_3 m_3 \, | j_1 m_1; j_2 m_2\rangle = \delta_{m_3, m_1+m_2} \langle j_3 m_1 + m_2 \, | j_1 m_1; j_2 m_2\rangle \tag{S.137}$$

which allows the summation over $m_3$ in Eq. (S.135) to be carried out, yielding

$$|j_1 m_1; j_2 m_2\rangle = \sum_{j_3} \langle j_3 m_1 + m_2 \, | j_1 m_1; j_2 m_2\rangle \, |j_3 m_1 + m_2\rangle \ . \tag{S.138}$$

Moreover, the condition $|j_1 - j_2| \leq j_3 \leq j_1 + j_2$ (where $j_1$, $j_2$, and $j_3$ are non-negative integers) must be satisfied, otherwise the corresponding coefficients vanish. These conditions follow directly from the rules governing angular momentum addition in quantum mechanics. Consequently, the sum over $j_3$ in Eq. (S.138) is taken over integer values satisfying $\max[|j_1 - j_2|, m_1 + m_2] \leq j_3 \leq j_1 + j_2$.

The explicit expression for the Gaunt coefficient is given by

$$\langle j_3 m_1 + m_2 \, | j_1 m_1; j_2 m_2\rangle = \sqrt{\frac{(2j_1+1)(2j_2+1)}{4\pi(2j_3+1)}} \times \\ \times \ \langle j_1 m_1; j_2 m_2 | \, j_3 m_1 + m_2\rangle \, \langle j_1 0; j_2 0 | \, j_3 0\rangle, \tag{S.139}$$

where $\langle j_1 m_1; j_2 m_2 | \, j_3 m_1 + m_2\rangle$ are the *Clebsch-Gordan coefficients*, which are defined as the expansion coefficients of the total angular momentum basis $|j_3 m_3\rangle$ in terms of the direct product basis $|j_1 m_1; j_2 m_2\rangle = |j_1 m_1\rangle \otimes |j_2 m_2\rangle$, using the completness relation in the uncoupled basis

$$|j_3 m_3\rangle = \sum_{j_1 m_1} \sum_{j_2 m_2} \langle j_1 m_1; j_2 m_2 \, | j_3 m_3\rangle \, |j_1 m_1\rangle \otimes |j_2 m_2\rangle \tag{S.140}$$

The Clebsch-Gordon coefficients are zero unless the following conditions hold

$$\begin{aligned} & m_i \in \{-j_i, -j_i + 1, \ldots, j_i - 1, j_i\} \\ & m_1 + m_2 = m_3 \\ & |j_1 - j_2| \leq j_3 \leq |j_1 + j_2| \\ & j_1 + j_2 + j_3 \text{ is an integer,} \end{aligned}$$

These coefficients are all real and possess the following symmetry properties:

$$\begin{aligned} \langle j_1 m_1; j_2 m_2 | \, j_3 m_3\rangle &= (-)^{j_1 + j_2 - j_3} \, \langle j_1(-m_1); j_2(-m_2) | \, j_3(-m_3)\rangle && \text{(S.141)} \\ &= (-)^{j_1 + j_2 - j_3} \, \langle j_2 m_2 : j_1 m_1 | \, j_3 m_3\rangle && \text{(S.142)} \\ &= (-)^{j_1 - m_1} \sqrt{\frac{2j_3+1}{2j_2+1}} \, \langle j_1 m_1; j_3(-m_3) | \, j_2(-m_2)\rangle && \text{(S.143)} \\ &= (-)^{j_2 + m_2} \sqrt{\frac{2j_3+1}{2j_1+1}} \, \langle j_3(-m_3); j_2 m_2 | \, j_1(-m_1)\rangle && \text{(S.144)} \\ &= (-)^{j_1 - m_1} \sqrt{\frac{2j_3+1}{2j_2+1}} \, \langle j_3 m_3; j_1(-m_1) | \, j_2 m_2\rangle && \text{(S.145)} \\ &= (-)^{j_2 + m_2} \sqrt{\frac{2j_3+1}{2j_1+1}} \, \langle j_2(-m_2); j_3 m_3 | \, j_1 m_1\rangle && \text{(S.146)} \end{aligned}$$

Clebsch-Gordan coefficients are related to *Wigner 3j-symbols* through

$$\langle j_1 m_1; j_2 m_2 \, | j_3 m_3\rangle = (-)^{j_1 - j_2 + m_3} \sqrt{2j_3+1} \begin{pmatrix} j_1 & j_2 & j_3 \\ m_1 & m_2 & -m_3 \end{pmatrix} \ , \tag{S.147}$$

leading to the Gaunt coefficient expression

$$\langle j_3 m_1+m_2 \,|j_1 m_1; j_2 m_2\rangle = (-)^{m_1+m_2}\sqrt{\frac{(2j_1+1)(2j_2+1)(2j_3+1)}{4\pi}}\begin{pmatrix} j_1 & j_2 & j_3 \\ m_1 & m_2 & -m_1-m_2\end{pmatrix}\begin{pmatrix} j_1 & j_2 & j_3 \\ 0 & 0 & 0\end{pmatrix}. \tag{S.148}$$

To compute the Wigner $3j$-symbol, we use the *Racah formula*

$$\begin{aligned}\begin{pmatrix} j_1 & j_2 & j_3 \\ m_1 & m_2 & -m_3\end{pmatrix} &= (-)^{j_1-j_2+m_3}\sqrt{\Delta(j_1,j_2,j_3)}\sqrt{(j_1+m_1)!(j_1-m_1)!(j_2+m_2)!(j_2-m_2)!(j_3+m_3)!(j_3-m_3)!}\times \\ &\times\sum_{t=0}^{\nu+1}\frac{(-)^t}{t!}\frac{1}{(j_3-j_2+t+m_1)!(j_3-j_1+t-m_2)!(j_1+j_2-j_3-t)!(j_1-t-m_1)!(j_2-t+m_2)!},\end{aligned} \tag{S.149}$$

where $m_1+m_2=m_3$, $|j_1-j_2|\le j_3\le j_1+j_2$, and

$$\Delta(j_1,j_2,j_3)=\frac{(j_1+j_2-j_3)!(j_2+j_3-j_1)!(j_3+j_1-j_2)!}{(j_1+j_2+j_3+1)!} \tag{S.150}$$

is the triangle coefficient. In Eq. (S.149) the sum runs over all integers $t$ for which the factorials remain non-negative. The number of terms in this sum is $\nu+1$, where $\nu$ is the smallest of the nine numbers

$$\begin{gathered} j_1\pm m_1 \quad j_2\pm m_2 \quad j_3\pm m_3 \\ j_1+j_2-j_3 \quad j_2+j_3-j_1 \quad j_3+j_1-j_2\,. \end{gathered} \tag{S.151}$$

In Sec. S.4 C, it is necessary to compute the Clebsch-Gordan coefficients $\langle l\pm 1 \mu+q; 1-q|\, l\mu\rangle$ for $q\in[-1,1]$. Using Eqs. (S.147), (S.149), and (S.150), we obtain

$$\langle l+1 \mu+q; 1-q|\, l\mu\rangle = (-)^{1-q}\sqrt{\frac{(l+1+\mu+q)!(l+1-\mu-q)!}{(2l+3)(l+1)(l+\mu)!(l-\mu)!(1-q)!(1+q)!}}\,, \tag{S.152}$$

$$\langle l-1 \mu+q; 1-q|\, l\mu\rangle = \sqrt{\frac{(l+\mu)!(l-\mu)!}{l(2l-1)(1-q)!(1+q)!(l-1-\mu-q)!(l-1+\mu+q)!}}\,. \tag{S.153}$$

Thus, for $-1\le q\le 1$, we find

$$\langle l+1 \mu+q; 1-q|\, l\mu\rangle = \begin{cases} \sqrt{\frac{(l+1-\mu)(l+2-\mu)}{2(l+1)(2l+3)}} & \text{if } q=-1 \\ -\sqrt{\frac{(l+1-\mu)(l+1+\mu)}{(l+1)(2l+3)}} & \text{if } q=0 \\ \sqrt{\frac{(l+1+\mu)(l+2+\mu)}{2(l+1)(2l+3)}} & \text{if } q=1 \end{cases} \tag{S.154}$$

$$\langle l-1 \mu+q; 1-q|\, l\mu\rangle = \begin{cases} \sqrt{\frac{(l-1+\mu)(l+\mu)}{2l(2l-1)}} & \text{if } q=-1 \\ \sqrt{\frac{(l+\mu)(l-\mu)}{l(2l-1)}} & \text{if } q=0 \\ \sqrt{\frac{(l-1-\mu)(l-\mu)}{2l(2l-1)}} & \text{if } q=1\,. \end{cases} \tag{S.155}$$

### C. Analytical evaluation of the gradient of a spherical function by means of real vector spherical harmonics

Let $f(\mathbf{r})$ be any function that can be expressed in spherical coordinates as $f_l(r)Y_{lm_l}(\widehat{\mathbf{r}})$, with $\widehat{\mathbf{r}} = \mathbf{r}/r = (\theta, \phi)$. Its gradient can be written as

$$\nabla_{\mathbf{r}} f_l(r) Y_{lm_l}(\widehat{\mathbf{r}}) = \mathbf{Y}_{lm_l} \frac{\partial f_l(r)}{\partial r} + \frac{f_l(r)}{r} \boldsymbol{\Psi}_{lm_l} \quad (S.156)$$

where $\mathbf{Y}_{lm_l} = \widehat{\mathbf{r}} Y_{lm_l}(\widehat{\mathbf{r}})$ and $\boldsymbol{\Psi}_{lm_l} = r\nabla_{\mathbf{r}} Y_{lm_l}(\widehat{\mathbf{r}})$ are extensions of the *scalar real spherical harmonics* to vector fields, i.e., the *real vector spherical harmonics*. The concept of vector spherical harmonics was first introduced by Blatt and Weisskopf [11] and Hill [12], and has been extensively used as an angular basis in quantum mechanics, in the study of electromagnetic and nuclear radiation [11, 13–15], and more recently in atomic and molecular physics [16, 17].

In this section we report a detailed derivation of the real vector spherical harmonics, as such derivations are not easily found in the literature. Our goal is to establish a general analytical expression constructed via a mapping relation between real and complex scalar spherical harmonics. We start by expressing the real spherical harmonics in terms of the complex ones as

$$\begin{aligned} Y_{l0}(\widehat{\mathbf{r}}) &= Y_l^0(\widehat{\mathbf{r}}) \\ Y_{lm_l}(\widehat{\mathbf{r}}) &= \tfrac{1}{\sqrt{2}}\left[(-)^{m_l} Y_l^{m_l}(\widehat{\mathbf{r}}) + Y_l^{-m_l}(\widehat{\mathbf{r}})\right] \\ Y_{l-m_l}(\widehat{\mathbf{r}}) &= \tfrac{i}{\sqrt{2}}\left[Y_l^{-m_l}(\widehat{\mathbf{r}}) - (-)^{m_l} Y_l^{m_l}(\widehat{\mathbf{r}})\right], \end{aligned} \quad (S.157)$$

where $Y_l^{m_l}(\widehat{\mathbf{r}})$ denotes the standard complex spherical harmonics in the Condon-Shortley convention, defined as

$$Y_l^{m_l}(\theta,\phi) = (-)^{m_l} \sqrt{\frac{2l+1}{4\pi} \frac{(l-m_l)!}{(l+m_l)!}} P_l^{m_l}(\cos\theta) e^{im_l\phi}, \quad (S.158)$$

with $P_l^{m_l}(\cos\theta)$ being the real associated Legendre polynomial. Using the property $Y_l^{-m_l}(\widehat{\mathbf{r}}) = (-)^{m_l} Y_l^{m_l *}(\widehat{\mathbf{r}})$, we rewrite Eqs. (S.157) as

$$\begin{aligned} Y_{l0}(\widehat{\mathbf{r}}) &= Y_l^0(\widehat{\mathbf{r}}) \\ Y_{lm_l}(\widehat{\mathbf{r}}) &= \tfrac{(-)^{m_l}}{\sqrt{2}}\left[Y_l^{m_l}(\widehat{\mathbf{r}}) + Y_l^{m_l *}(\widehat{\mathbf{r}})\right] \\ &= \sqrt{2}(-)^{m_l} \mathrm{Re}[Y_l^{m_l}(\widehat{\mathbf{r}})] \quad (S.159) \\ Y_{l-m_l}(\widehat{\mathbf{r}}) &= \tfrac{i(-)^{m_l}}{\sqrt{2}}\left[Y_l^{m_l *}(\widehat{\mathbf{r}}) - Y_l^{m_l}(\widehat{\mathbf{r}})\right] \\ &= \sqrt{2}(-)^{m_l} \mathrm{Im}[Y_l^{m_l}(\widehat{\mathbf{r}})]. \end{aligned}$$

These expressions can be further generalized through a linear combination of complex spherical harmonics[18]

$$Y_{lm_l}(\widehat{\mathbf{r}}) = \sum_{\mu=-l}^{l} U^l_{m_l\mu} Y_l^\mu(\widehat{\mathbf{r}}), \quad (S.160)$$

where $\mathbf{U}^l$ is a $(2l+1)\times(2l+1)$-dimensional unitary matrix satisfying the properties

$$\sum_{m_l} [U^l_{m_l\mu}]^* U^l_{m_l\mu'} = \delta_{\mu\mu'} \quad \sum_{\mu} [U^l_{m_l\mu}]^* U^l_{m\mu} = \delta_{m_l m}. \quad (S.161)$$

As a result, the real spherical harmonics define a set of orthonormal functions:

$$\begin{aligned} &\int_0^{2\pi}\int_0^{\pi} d\phi d\theta \sin\theta Y_{lm_l}(\widehat{\mathbf{r}}) Y_{l'm_{l'}}(\widehat{\mathbf{r}}) = \\ &= \sum_{\mu\mu'} [U^l_{m_l\mu}]^* U^l_{m_{l'}\mu'} \int_0^{2\pi}\int_0^{\pi} d\phi d\theta \sin\theta Y_l^\mu(\widehat{\mathbf{r}}) Y_{l'}^{\mu'}(\widehat{\mathbf{r}}) \\ &= \sum_{\mu\mu'} [U^l_{m_l\mu}]^* U^l_{m_{l'}\mu'} \delta_{ll'}\delta_{\mu\mu'} \\ &= \delta_{ll'} \sum_{\mu} [U^l_{m_l\mu}]^* U^l_{m_{l'}\mu} = \delta_{ll'}\delta_{m_l m_{l'}}. \end{aligned} \quad (S.162)$$

Notably, as a consequence of the completeness of the scalar complex harmonics, the scalar real spherical harmonics also form a complete set[18].

An important consequence of properties (S.161) is the expression

$$Y_l^\mu(\widehat{\mathbf{r}}) = \sum_{m_l=-l}^{l} [U^l_{m_l\mu}]^* Y_{lm_l}(\widehat{\mathbf{r}}), \quad (S.163)$$

which can be easily derived by multiplying both sides of Eq. (S.160) by $[U^l_{m_l\mu'}]^*$, summing over $m_l$, and using the unitarity condition (S.161) of the transformation matrix. Starting from the condition $Y^*_{lm_l} = Y_{lm_l}$, employing the expansion (S.160), and using the property $Y_l^{-m_l}(\widehat{\mathbf{r}}) = (-)^{m_l} Y_l^{m_l *}(\widehat{\mathbf{r}})$, we obtain the constraint

$$\sum_{\mu=-l}^{l} \{(-)^\mu [U^l_{m_l-\mu}]^* - U^l_{m_l\mu}\} Y_l^\mu(\widehat{\mathbf{r}}) = 0 \quad (S.164)$$

Since the complex spherical harmonics are linearly independent, the elements of the unitary matrix $\mathbf{U}^l$ must satisfy the additional condition

$$[U^l_{m_l\mu}]^* = (-)^\mu U^l_{m_l-\mu}. \quad (S.165)$$

For a given $l$, Eqs. (S.159) and (S.160) can be expressed in the following matrix formalism[18]

$$
\begin{pmatrix} Y_{ll} \\ Y_{ll-1} \\ \vdots \\ Y_{l1} \\ Y_{l0} \\ Y_{l-1} \\ \vdots \\ Y_{l-l+1} \\ Y_{l-l} \end{pmatrix} = \underbrace{\frac{1}{\sqrt{2}} \begin{pmatrix} (-)^l & & & & & & & & 1 \\ & (-)^{l-1} & & & & & & 1 & \\ & & \ddots & & & & & & \\ & & & -1 & & 1 & & & \\ & & & & \sqrt{2} & & & & \\ & & & i & & i & & & \\ & & & & & & \ddots & & \\ & -i(-)^{l-1} & & & & & & i & \\ -i(-)^l & & & & & & & & i \end{pmatrix}}_{=\mathbf{U}^l} \begin{pmatrix} Y_l^l \\ Y_l^{l-1} \\ \vdots \\ Y_l^1 \\ Y_l^0 \\ Y_l^{-1} \\ \vdots \\ Y_l^{-l+1} \\ Y_l^{-l} \end{pmatrix} \tag{S.166}
$$

from which the structure of the transformation matrix $\mathbf{U}^l$ is evident, and it follows that $U^l_{m_l\mu} = 0$ if $|m_l| \neq |\mu|$.

This initial characterization of the unitary matrix $\mathbf{U}^l$ is essential for deriving a simple analytical expression for the real vector spherical harmonics by leveraging theorems and properties that hold for the complex spherical harmonics but not for their real counterparts.

### 1. *Analytical expression for* $\mathbf{Y}_{lm_l} = \widehat{\mathbf{r}} Y_{lm_l}$

The radial unit vector $\widehat{\mathbf{r}}$ defined in cartesian coordinates

$$
\widehat{\mathbf{r}} = \widehat{\mathbf{e}}_x \sin\theta\cos\phi + \widehat{\mathbf{e}}_y \sin\theta\sin\phi + \widehat{\mathbf{e}}_z \cos\theta \,, \tag{S.167}
$$

complicates the derivation of an expression for the real vector spherical harmonics $\mathbf{Y}_{lm_l} = \widehat{\mathbf{r}} Y_{lm_l}(\widehat{\mathbf{r}})$. However, a *simple* analytical expression can be obtained by rewriting the unit vector $\widehat{\mathbf{r}}$ in terms of spherical unit vectors $\{\widehat{\mathbf{e}}_q\}$ and complex spherical harmonics as

$$
\widehat{\mathbf{r}} = \sqrt{\tfrac{4\pi}{3}} \sum_{q=-1}^{1} (-)^q Y_1^q(\widehat{\mathbf{r}})\, \widehat{\mathbf{e}}_{-q} \,, \tag{S.168}
$$

where

$$
\begin{aligned}
\widehat{\mathbf{e}}_0 &= \widehat{\mathbf{e}}_z \\
\widehat{\mathbf{e}}_{\pm 1} &= \mp \tfrac{1}{\sqrt{2}} (\widehat{\mathbf{e}}_x \pm i \widehat{\mathbf{e}}_y) \,.
\end{aligned} \tag{S.169}
$$

The spherical unit vectors satisfy the properties $\widehat{\mathbf{e}}^*_q = (-)^q \widehat{\mathbf{e}}_{-q}$ and $\widehat{\mathbf{e}}_\mu \cdot \widehat{\mathbf{e}}^*_\nu = \delta_{\mu\nu}$, which allow us to rewrite Eq. (S.168) as

$$
\widehat{\mathbf{r}} = \sqrt{\tfrac{4\pi}{3}} \sum_{q=-1}^{1} Y_1^q(\widehat{\mathbf{r}})\, \widehat{\mathbf{e}}^*_q \,. \tag{S.170}
$$

Thus, the vector spherical harmonics $\mathbf{Y}_{lm_l}$ can be rewritten as

$$
\begin{aligned}
\mathbf{Y}_{lm_l} &= \sqrt{\tfrac{4\pi}{3}} Y_{lm_l} \sum_{q=-1}^{1} Y_1^q(\widehat{\mathbf{r}})\, \widehat{\mathbf{e}}^*_q \\
&= \sqrt{\tfrac{4\pi}{3}} \sum_{\mu=-l}^{l} \sum_{q=-1}^{1} U^l_{m_l,\mu} Y_l^\mu(\widehat{\mathbf{r}}) Y_1^q(\widehat{\mathbf{r}})\, \widehat{\mathbf{e}}^*_q
\end{aligned} \tag{S.171}
$$

where Eq. (S.160) has been used to rewrite the real spherical harmonics $Y_{lm_l}(\widehat{\mathbf{r}})$ in terms of their complex counterparts. The product of the complex spherical harmonics, $Y_l^\mu Y_1^q$, can be expressed as a sum of complex spherical harmonics weighted by Gaunt coefficients

$$
\begin{aligned}
Y_l^\mu(\widehat{\mathbf{r}}) Y_1^q(\widehat{\mathbf{r}}) = \sum_{l'} \sqrt{\frac{3(2l+1)}{4\pi(2l'+1)}} \times \\
\times \langle l\mu; 1q |\, l'\mu+q \rangle \, \langle l0\,; 10 |\, l'0 \rangle Y_{l'}^{\mu+q}(\widehat{\mathbf{r}}),
\end{aligned} \tag{S.172}
$$

where $\langle j_1 m_1; j_2 m_2 |\, j_3 m_3 \rangle$ are the Clebsch-Gordan coefficients introduced in Eqs. (S.138) and (S.139) of Sec. S.4 B. Only two terms, corresponding to $l' = l \pm 1$, contribute to the sum over $l'$ in Eq. (S.171) since

$$
\langle l0\,; 10 |\, l'0 \rangle = \begin{cases} \sqrt{\frac{l+1}{2l+1}} & \text{for } l' = l+1 \\ 0 & \text{for } l' \neq l \pm 1 \\ -\sqrt{\frac{l}{2l+1}} & \text{for } l' = l-1 \end{cases} . \tag{S.173}
$$

Inserting Eq. (S.172) into the right-hand side of Eq. (S.171) and employing Eq. (S.173) yields

$$
\mathbf{Y}_{lm_l} = \sum_{\mu=-l}^{l} \sum_{q=-1}^{1} U^l_{m_l,\mu} \widehat{\mathbf{e}}^*_q \left[ \sqrt{\frac{l+1}{2l+3}} \, \langle l\mu; 1q |\, l+1 \mu+q \rangle Y_{l+1}^{\mu+q}(\widehat{\mathbf{r}}) - \sqrt{\frac{l}{2l-1}} \, \langle l\mu; 1q |\, l-1 \mu+q \rangle Y_{l-1}^{\mu+q}(\widehat{\mathbf{r}}) \right] . \tag{S.174}
$$

It is convenient to rewrite Eq. (S.174) using the symmetry properties of the Clebsch-Gordan coefficients provided in Sec. S.4 B. By applying Eqs. (S.144) and (S.141), the Clebsch-Gordan coefficient $\langle l\mu; 1q |\, l+1 \mu+q \rangle$ can be rewritten

as

$$\langle l\mu;1q|\,l+1\mu+q\rangle = (-)^{1+q}\sqrt{\frac{2l+3}{2l+1}}\,\langle l+1(-\mu-q);1q|\,l(-\mu)\rangle = -(-)^{q}\sqrt{\frac{2l+3}{2l+1}}\,\langle l+1\mu+q;1-q|\,l\mu\rangle \tag{S.175}$$

Similarly,

$$\langle l\mu;1q|\,l-1\mu+q\rangle = -(-)^{q}\sqrt{\frac{2l-1}{2l+1}}\,\langle l-1\mu+q;1-q|\,l\mu\rangle\,, \tag{S.176}$$

which allows us to rewrite Eq. (S.174) as

$$\mathbf{Y}_{lm_l} = -\sum_{\mu=-l}^{l}\sum_{q=-1}^{1}(-)^{q}U^{l}_{m_l,\mu}\widehat{\mathbf{e}}^{*}_{q}\left[\sqrt{\frac{l+1}{2l+1}}\,\langle l+1\mu+q;1-q|\,l\mu\rangle Y^{\mu+q}_{l+1}(\widehat{\mathbf{r}}) - \sqrt{\frac{l}{2l+1}}\,\langle l-1\mu+q;1-q|\,l\mu\rangle Y^{\mu+q}_{l-1}(\widehat{\mathbf{r}})\right]. \tag{S.177}$$

Using Eq. (S.163), we can express the complex spherical harmonics in Eq. (S.177) in terms of their real counterparts

$$\begin{aligned}\mathbf{Y}_{lm_l} = &-\sum_{\mu=-l}^{l}\sum_{\nu=-l-1}^{l+1}\sum_{q=-1}^{1}(-)^{q}U^{l}_{m_l,\mu}[U^{l+1}_{\nu,\mu+q}]^{*}\widehat{\mathbf{e}}^{*}_{q}\sqrt{\frac{l+1}{2l+1}}\,\langle l+1\mu+q;1-q|\,l\mu\rangle Y_{l+1,\nu}(\widehat{\mathbf{r}})+\\ &+\sum_{\mu=-l}^{l}\sum_{\nu=-l+1}^{l-1}\sum_{q=-1}^{1}(-)^{q}U^{l}_{m_l,\mu}[U^{l-1}_{\nu,\mu+q}]^{*}\widehat{\mathbf{e}}^{*}_{q}\sqrt{\frac{l}{2l+1}}\,\langle l-1\mu+q;1-q|\,l\mu\rangle Y_{l-1,\nu}(\widehat{\mathbf{r}})\,.\end{aligned} \tag{S.178}$$

Finally, introducing the *real tensor spherical harmonics*

$$\boxed{\mathbf{Y}^{m_l\mu\nu}_{l,l\pm1}(\widehat{\mathbf{r}}) = U^{l}_{m_l,\mu}Y_{l\pm1,\nu}(\widehat{\mathbf{r}})\sum_{q=-1}^{1}(-)^{q}[U^{l\pm1}_{\nu,\mu+q}]^{*}\widehat{\mathbf{e}}^{*}_{q}\,\langle l\pm1\mu+q;1-q|\,l\mu\rangle}\,, \tag{S.179}$$

Eq. (S.178) can then be rewritten as

$$\boxed{\mathbf{Y}_{lm_l} = -\sum_{\mu=-l}^{l}\sum_{\nu=-l-1}^{l+1}\sqrt{\frac{l+1}{2l+1}}\mathbf{Y}^{m_l\mu\nu}_{l,l+1}(\widehat{\mathbf{r}}) + \sum_{\mu=-l}^{l}\sum_{\nu=-l+1}^{l-1}\sqrt{\frac{l}{2l+1}}\mathbf{Y}^{m_l\mu\nu}_{l,l-1}(\widehat{\mathbf{r}})}\,. \tag{S.180}$$

### 2. *Analytical expression for* $\mathbf{\Psi}_{lm_l} = r\nabla_{\mathbf{r}}Y_{lm_l}$

In analogy with Eq. (S.168), the gradient operator in spherical coordinates, given by

$$\nabla_{\mathbf{r}} = \frac{\partial}{\partial r}\widehat{\mathbf{r}} + \frac{1}{r}\frac{\partial}{\partial\theta}\widehat{\theta} + \frac{1}{r\sin\theta}\frac{\partial}{\partial\phi}\widehat{\phi}\,, \tag{S.181}$$

can be expanded in terms of the spherical unit vectors (S.169) and the components of the gradient operator in the spherical basis

$$\nabla_{\mathbf{r}} = \sum_{q=-1}^{1}(-)^{q}\widehat{\mathbf{e}}_{-q}\nabla_{q} = \sum_{q=-1}^{1}\widehat{\mathbf{e}}^{*}_{q}\nabla_{q}, \tag{S.182}$$

where $\nabla_q$ is defined as

$$\begin{aligned}\nabla_{\pm1} &= \mp\tfrac{1}{\sqrt{2}}\left(\frac{\partial}{\partial x}\pm i\frac{\partial}{\partial y}\right)\\ &= \mp\frac{e^{\pm i\phi}}{\sqrt{2}}\left[\sin\theta\frac{\partial}{\partial r} + \frac{\cos\theta}{r}\frac{\partial}{\partial\theta} \pm \frac{i}{r\sin\theta}\frac{\partial}{\partial\phi}\right]\end{aligned} \tag{S.183}$$

for $q = \pm1$ and

$$\nabla_0 = \frac{\partial}{\partial z} = \cos\theta\frac{\partial}{\partial r} - \frac{\sin\theta}{r}\frac{\partial}{\partial\theta} \tag{S.184}$$

for $q = 0$. Using Eq. (S.182) into the definition $\mathbf{\Psi}_{lm_l} = r\nabla_{\mathbf{r}}Y_{lm_l}$, we obtain

$$\begin{aligned}\mathbf{\Psi}_{lm_l} &= r\sum_{q=-1}^{1}\widehat{\mathbf{e}}^{*}_{q}\nabla_{q}Y_{lm_l}(\widehat{\mathbf{r}})\\ &= r\sum_{\mu=-l}^{l}\sum_{q=-1}^{1}U^{l}_{m_l\mu}\widehat{\mathbf{e}}^{*}_{q}\nabla_{q}Y^{\mu}_{l}(\widehat{\mathbf{r}})\,,\end{aligned} \tag{S.185}$$

where the set of real spherical harmonics $\{Y_{lm_l}\}$ have been replaced by their complex counterparts. The completeness relation in the angular states $|lm_l\rangle$, expressed in terms of complex spherical harmonics, allows rewriting

the above equation as

$$\mathbf{\Psi}_{lm_l} = r \sum_{l'm_{l'}} \sum_{\mu=-l}^{l} \sum_{q=-1}^{1} U^l_{m_l\mu} \widehat{\mathbf{e}}^*_q Y^{m_{l'}}_{l'}(\widehat{\mathbf{r}}) \langle l'm_{l'}| \nabla_q |l\mu\rangle \,, \tag{S.186}$$

where the coordinate-space representation $\langle \widehat{\mathbf{r}}| \nabla_q |l\mu\rangle = \nabla_q Y^{\mu}_l(\widehat{\mathbf{r}})$ was used. The matrix elements of the spherical vector operator on the complex spherical harmonics can be computed using the *Wigner-Eckart theorem*[19], which states that

$$\langle l'm_{l'}| \nabla_q |l\mu\rangle = \langle l\mu; 1q| l'm_{l'}\rangle \langle l' \|\nabla\| l\rangle \,, \tag{S.187}$$

where the *reduced matrix elements* $\langle l' \|\nabla\| l\rangle$ are independent of $q$, $\mu$, and $m_{l'}$. This property facilitates its evaluation by considering Eq. (S.187) in the particular case $q = \mu = m_{l'} = 0$, yielding

$$\langle l' \|\nabla\| l\rangle = \frac{\langle l'0| \nabla_0 |l0\rangle}{\langle l0; 10| l'0\rangle} \,. \tag{S.188}$$

Thus, Eq. (S.187) can be reformulated as

$$\langle l'm_{l'}| \nabla_q |l\mu\rangle = \frac{\langle l\mu; 1q| l'm_{l'}\rangle}{\langle l0; 10| l'0\rangle} \langle l'0| \nabla_0 |l0\rangle \,, \tag{S.189}$$

in terms of quantities with a well-defined analytical form. The Clebsch-Gordan coefficients introduced in Sec. (S.4 C 1) allow for the explicit evaluation of the matrix element $\langle l'0| \nabla_0 |l0\rangle$ in the coordinate representation using Eqs. (S.184) and (S.158), with the latter stating that $Y^0_l(\widehat{\mathbf{r}}) = \sqrt{(2l+1)/4\pi} P^0_l(\cos\theta)$,

$$\begin{aligned}\langle l'0| \nabla_0 |l0\rangle &= \int_0^{2\pi}\int_0^{\pi} d\phi d\theta \sin\theta Y^0_{l'}(\widehat{\mathbf{r}}) \Big[-\frac{\sin\theta}{r}\frac{\partial}{\partial\theta}\Big] Y^0_l(\widehat{\mathbf{r}}) \\ &= \frac{\sqrt{(2l+1)(2l'+1)}}{2r}\int_{-1}^{1} d\cos\theta (1-\cos^2\theta) P^0_{l'}(\cos\theta) \frac{\partial}{\partial\cos\theta} P^0_l(\cos\theta) \,. \end{aligned}\tag{S.190}$$

With the substitution $x = \cos\theta$, and employing the recurrence relation for the first derivative of the Legendre polynomials

$$\frac{1-x^2}{l}\frac{\partial P^0_l(x)}{\partial x} = P^0_{l-1}(x) - x P^0_l(x) \tag{S.191}$$

and their orthogonality property, $\int_{-1}^{1} P^0_l(x) P^0_{l'}(x) dx = 2\delta_{ll'}/(2l+1)$, Eq. (S.190) simplifies to

$$\langle l'0| \nabla_0 |l0\rangle = \frac{\sqrt{(2l+1)(2l'+1)}}{2r}\Big[\frac{2l}{2l-1}\delta_{l-1,l'} - l\int_{-1}^{1} dx\, x P^0_l(x) P^0_{l'}(x)\Big] \,. \tag{S.192}$$

To compute the second integral, we use $cos\theta = P^0_1(\cos\theta) = \sqrt{4\pi/3} Y^0_1(\widehat{\mathbf{r}})$ and the Gaunt coefficient definition (S.139)

$$2\pi\int_{-1}^{1} d\cos\theta\, Y^0_{l'}(\widehat{\mathbf{r}}) Y^0_l(\widehat{\mathbf{r}}) Y^0_1(\widehat{\mathbf{r}}) = \sqrt{\frac{3(2l+1)}{4\pi(2l'+1)}} \langle l0; 10| l'0\rangle^2 \,, \tag{S.193}$$

which leads to

$$\int_{-1}^{1} dx\, x P^0_l(x) P^0_{l'}(x) = \frac{2}{2l'+1} \langle l0; 10| l'0\rangle^2 \,. \tag{S.194}$$

Substituting Eqs. (S.194) and (S.192) into (S.189), we obtain

$$\begin{aligned}\langle l'm_{l'}| \nabla_q |l\mu\rangle &= \frac{\sqrt{(2l+1)(2l'+1)}}{r} \langle l\mu; 1q| l'm_{l'}\rangle \Big[\frac{l}{2l-1}\frac{\delta_{l-1,l'}}{\langle l0; 10| l'0\rangle} - \frac{l}{2l'+1}\langle l0; 10| l'0\rangle\Big] \\ &= -\frac{\langle l\mu; 1q| l'm_{l'}\rangle}{r}\Big[(l+1)\sqrt{\frac{l}{2l-1}}\delta_{l-1,l'} + l\sqrt{\frac{l+1}{2l+3}}\delta_{l+1,l'}\Big] \,, \end{aligned}\tag{S.195}$$

where Eq. (S.173) was used to evaluate the Clebsch-Gordan coefficients $\langle l0; 10| l'0\rangle$

$$\langle l0; 10| l'0\rangle = \delta_{l+1,l'}\sqrt{\frac{l+1}{2l+1}} - \delta_{l-1,l'}\sqrt{\frac{l}{2l+1}} \,. \tag{S.196}$$

Inserting Eq. (S.195) into the expansion (S.186), we derive an analytical expression for the vector spherical harmonics $\mathbf{\Psi}_{lm_l} = r\nabla_{\mathbf{r}} Y_{lm_l}$

$$\begin{aligned}\mathbf{\Psi}_{lm_l} &= -\sum_{l'm_{l'}}\sum_{\mu=-l}^{l}\sum_{q=-1}^{1} U^l_{m_l\mu}\widehat{\mathbf{e}}^*_q Y^{m_{l'}}_{l'}(\widehat{\mathbf{r}})\,\langle l\mu;1q|\,l'm_{l'}\rangle\left[(l+1)\sqrt{\frac{l}{2l-1}}\delta_{l-1,l'}+l\sqrt{\frac{l+1}{2l+3}}\delta_{l+1,l'}\right]\\ &= -\sum_{\mu=-l}^{l}\sum_{q=-1}^{1} U^l_{m_l\mu}\widehat{\mathbf{e}}^*_q Y^{\mu+q}_{l+1}(\widehat{\mathbf{r}})\,\langle l\mu;1q|\,l+1\mu+q\rangle l\sqrt{\frac{l+1}{2l+3}}-\\ &\qquad -\sum_{\mu=-l}^{l}\sum_{q=-1}^{1} U^l_{m_l\mu}\widehat{\mathbf{e}}^*_q Y^{\mu+q}_{l-1}(\widehat{\mathbf{r}})\,\langle l\mu:1q|\,l-1\mu+q\rangle(l+1)\sqrt{\frac{l}{2l-1}}\,, \end{aligned}\tag{S.197}$$

where only Clebsch-Gordan coefficients with $m_{l'} = \mu + q$ survive in the above expansion. Finally, using Eqs. (S.163), (S.175), (S.176), and (S.179), we obtain

$$\boxed{\mathbf{\Psi}_{lm_l} = \sum_{\mu=-l}^{l}\sum_{\nu=-l-1}^{l+1} l\sqrt{\frac{l+1}{2l+1}}\mathbf{Y}^{m_l\mu\nu}_{l,l+1}(\widehat{\mathbf{r}}) + \sum_{\mu=-l}^{l}\sum_{\nu=-l+1}^{l-1}(l+1)\sqrt{\frac{l}{2l+1}}\mathbf{Y}^{m_l\mu\nu}_{l,l-1}(\widehat{\mathbf{r}})}\,,\tag{S.198}$$

which is known in the literature as the *gradient formula.*

### 3. Final expression for $\nabla_{\mathbf{r}} f_l(r) Y_{lm_l}(\widehat{\mathbf{r}})$

Combining Eqs. (S.156), (S.180), and (S.198), we compute the gradient of $f_l(r)Y_{lm_l}(\widehat{\mathbf{r}})$ through the expression

$$\nabla_{\mathbf{r}} f_l(r)Y_{lm_l}(\widehat{\mathbf{r}}) = \sum_{\mu=-l}^{l}\left\{\sqrt{\frac{l}{2l+1}}\left[\frac{\partial}{\partial r}+\frac{l+1}{r}\right]f_l(r)\sum_{\nu=-l+1}^{l-1}\mathbf{Y}^{m_l\mu\nu}_{l,l-1}(\widehat{\mathbf{r}}) - \sqrt{\frac{l+1}{2l+1}}\left[\frac{\partial}{\partial r}-\frac{l}{r}\right]f_l(r)\sum_{\nu=-l-1}^{l+1}\mathbf{Y}^{m_l\mu\nu}_{l,l+1}(\widehat{\mathbf{r}})\right\}.\tag{S.199}$$

However, we are interested in the cartesian components of the above gradient, which can be simply found through Eqs. (S.169). Then, the cartesian component $\left(\sum_\mu \mathbf{Y}^{m_l\mu\nu}_{l,l\pm1}\right)_x$ of the real tensor spherical harmonics is evaluated as its projection on the $\widehat{\mathbf{e}}_x$ unit vector

$$\begin{aligned}\widehat{\mathbf{e}}_x\cdot\sum_{\mu=-l}^{l}\mathbf{Y}^{m_l\mu\nu}_{l,l\pm1}(\widehat{\mathbf{r}}) &= Y_{l\pm1,\nu}(\widehat{\mathbf{r}})\sum_{\mu=-l}^{l}\sum_{q=-1}^{1}(-)^q U^l_{m_l,\mu}[U^{l\pm1}_{\nu,\mu+q}]^*\,\langle l\pm1\mu+q;1-q|\,l\mu\rangle\,\widehat{\mathbf{e}}_x\cdot\widehat{\mathbf{e}}^*_q\\ &= \tfrac{1}{\sqrt{2}}Y_{l\pm1,\nu}(\widehat{\mathbf{r}})\sum_{\mu=-l}^{l}U^l_{m_l,\mu}\left\{[U^{l\pm1}_{\nu,\mu+1}]^*\,\langle l\pm1\mu+1;1-1|\,l\mu\rangle-[U^{l\pm1}_{\nu,\mu-1}]^*\,\langle l\pm1\mu-1;1\,1|\,l\mu\rangle\right\}\\ &= \gamma^{lm_l}_{l\pm1,\nu,x}Y_{l\pm1,\nu}(\widehat{\mathbf{r}})\,, \end{aligned}\tag{S.200}$$

with the Clebsch-Gordan coefficients defined by Eqs. (S.154) and (S.155) and

$$\gamma^{lm_l}_{l\pm1,\nu,x} = \begin{cases}\sum_{\mu=-l}^{l}\frac{U^l_{m_l,\mu}}{\sqrt{4(l+1)(2l+3)}}\left\{[U^{l+1}_{\nu,\mu+1}]^*\sqrt{(l+1+\mu)(l+2+\mu)}-[U^{l+1}_{\nu,\mu-1}]^*\sqrt{(l+1-\mu)(l+2-\mu)}\right\} & l+1 \text{ case}\\ \sum_{\mu=-l}^{l}\frac{U^l_{m_l,\mu}}{\sqrt{4l(2l-1)}}\left\{[U^{l-1}_{\nu,\mu+1}]^*\sqrt{(l-1-\mu)(l-\mu)}-[U^{l-1}_{\nu,\mu-1}]^*\sqrt{(l-1+\mu)(l+\mu)}\right\} & l-1 \text{ case}\end{cases}\tag{S.201}$$

The cartesian component $\left(\sum_\mu \mathbf{Y}^{m_l\mu\nu}_{l,l\pm1}\right)_y$ is found to be

$$\begin{aligned}\widehat{\mathbf{e}}_y\cdot\sum_{\mu=-l}^{l}\mathbf{Y}^{m_l\mu\nu}_{l,l\pm1}(\widehat{\mathbf{r}}) &= Y_{l\pm1,\nu}(\widehat{\mathbf{r}})\sum_{\mu=-l}^{l}\sum_{q=-1}^{1}(-)^q U^l_{m_l,\mu}[U^{l\pm1}_{\nu,\mu+q}]^*\,\langle l\pm1\mu+q;1-q|\,l\mu\rangle\,\widehat{\mathbf{e}}_y\cdot\widehat{\mathbf{e}}^*_q\\ &= -\tfrac{i}{\sqrt{2}}Y_{l\pm1,\nu}(\widehat{\mathbf{r}})\sum_{\mu=-l}^{l}U^l_{m_l,\mu}\left\{[U^{l\pm1}_{\nu,\mu-1}]^*\,\langle l\pm1\mu-1;1\,1|\,l\mu\rangle+[U^{l\pm1}_{\nu,\mu+1}]^*\,\langle l\pm1\mu+1;1\ -1|\,l\mu\rangle\right\}\\ &= \gamma^{lm_l}_{l\pm1,\nu,y}Y_{l\pm1,\nu}(\widehat{\mathbf{r}})\,, \end{aligned}\tag{S.202}$$

with

$$\gamma^{lm_l}_{l\pm1,\nu,y} = \begin{cases} -i\sum_{\mu=-l}^{l} \frac{U^l_{m_l,\mu}}{\sqrt{4(l+1)(2l+3)}} \left\{ [U^{l+1}_{\nu,\mu-1}]^* \sqrt{(l+2-\mu)(l+1-\mu)} + [U^{l+1}_{\nu,\mu+1}]^* \sqrt{(l+1+\mu)(l+2+\mu)} \right\} & l+1 \text{ case} \\ -i\sum_{\mu=-l}^{l} \frac{U^l_{m_l,\mu}}{\sqrt{4l(2l-1)}} \left\{ [U^{l-1}_{\nu,\mu-1}]^* \sqrt{(l-1+\mu)(l+\mu)} + [U^{l-1}_{\nu,\mu+1}]^* \sqrt{(l-1-\mu)(l-\mu)} \right\} & l-1 \text{ case} \end{cases} \tag{S.203}$$

Finally, the cartesian component $\left(\sum_\mu \mathbf{Y}^{m_l\mu\nu}_{l,l\pm1}\right)_z$ is

$$\begin{aligned} \widehat{\mathbf{e}}_z \cdot \sum_{\mu=-l}^{l} \mathbf{Y}^{m_l\mu\nu}_{l,l\pm1}(\widehat{\mathbf{r}}) &= Y_{l\pm1,\nu}(\widehat{\mathbf{r}}) \sum_{\mu=-l}^{l}\sum_{q=-1}^{1} (-)^q U^l_{m_l,\mu}[U^{l\pm1}_{\nu,\mu+q}]^* \left\langle l\pm1\mu+q;1-q\right| l\mu\rangle\, \widehat{\mathbf{e}}_z\cdot\widehat{\mathbf{e}}^*_q \\ &= Y_{l\pm1,\nu}(\widehat{\mathbf{r}}) \sum_{\mu=-l}^{l} U^l_{m_l,\mu}[U^{l\pm1}_{\nu,\mu}]^* \left\langle l\pm1\mu;1\,0\right| l\mu\rangle \\ &= \gamma^{lm_l}_{l\pm1,\nu,z} Y_{l\pm1,\nu}(\widehat{\mathbf{r}}) \,, \end{aligned} \tag{S.204}$$

with

$$\gamma^{lm_l}_{l\pm1,\nu,z} = \begin{cases} -\sum_{\mu=-l}^{l} U^l_{m_l,\mu}[U^{l+1}_{\nu,\mu}]^* \sqrt{\frac{(l+1-\mu)(l+1+\mu)}{(l+1)(2l+3)}} & l+1 \text{ case} \\ \sum_{\mu=-l}^{l} U^l_{m_l,\mu}[U^{l-1}_{\nu,\mu}]^* \sqrt{\frac{(l+\mu)(l-\mu)}{l(2l-1)}} & l-1 \text{ case} \end{cases} \tag{S.205}$$

Therefore, the $\alpha$-th component of the gradient of $f_l(r)Y_{lm_l}(\widehat{\mathbf{r}})$ will be

$$\begin{aligned} \left[\nabla_{\mathbf{r}} f_l(r) Y_{lm_l}(\widehat{\mathbf{r}})\right]_\alpha &= \sqrt{\frac{l}{2l+1}} \left[\frac{\partial}{\partial r} + \frac{l+1}{r}\right] f_l(r) \sum_{\nu=-l+1}^{l-1} \gamma^{lm_l}_{l-1,\nu,\alpha} Y_{l-1,\nu}(\widehat{\mathbf{r}}) - \\ &\quad - \sqrt{\frac{l+1}{2l+1}} \left[\frac{\partial}{\partial r} - \frac{l}{r}\right] f_l(r) \sum_{\nu=-l-1}^{l+1} \gamma^{lm_l}_{l+1,\nu,\alpha} Y_{l+1,\nu}(\widehat{\mathbf{r}}) \,. \end{aligned} \tag{S.206}$$

Note that the final expression (S.206) can be simplified when using spherical Bessel and Hankel functions. When replacing the spherical function $f_l(r)$ with a spherical Bessel function in the Methfessel convention, $j^m_l(ar)$, using Eqs. (S.117) and (S.122) yields

$$\left[\frac{\partial}{\partial r} + \frac{l+1}{r}\right] j^m_l(ar) = \frac{2l+1}{r} j^m_l(ar) - a^2 j^m_{l+1}(ar) = j^m_{l-1}(ar) \,,$$

$$\left[\frac{\partial}{\partial r} - \frac{l}{r}\right] j^m_l(ar) = -a^2 j^m_{l+1}(ar) \,.$$

Similarly, using Eqs. (S.121) and (S.123) for Hankel functions in the Methfessel convention, $h^m_l(ar)$, we obtain

$$\left[\frac{\partial}{\partial r} + \frac{l+1}{r}\right] h^m_l(ar) = \frac{2l+1}{r} h^m_l(ar) - h^m_{l+1}(ar) = h^m_{l-1}(ar) \,,$$

$$\left[\frac{\partial}{\partial r} - \frac{l}{r}\right] h^m_l(ar) = -h^m_{l+1}(ar) \,.$$

Therefore, the final expression for Eq. (S.206) in the case of Bessel and Hankel functions in the Methfessel convention will be

$$\left[\nabla_{\mathbf{r}} j^m_l(ar) Y_{lm_l}(\widehat{\mathbf{r}})\right]_\alpha = j^m_{l-1}(ar)\sqrt{\frac{l}{2l+1}} \sum_{\nu=-l+1}^{l-1} \gamma^{lm_l}_{l-1,\nu,\alpha} Y_{l-1,\nu}(\widehat{\mathbf{r}}) + a^2 j^m_{l+1}(ar)\sqrt{\frac{l+1}{2l+1}} \sum_{\nu=-l-1}^{l+1} \gamma^{lm_l}_{l+1,\nu,\alpha} Y_{l+1,\nu}(\widehat{\mathbf{r}}) \,, \tag{S.207}$$

$$\left[\nabla_{\mathbf{r}} h_l^m(ar) Y_{lm_l}(\widehat{\mathbf{r}})\right]_\alpha = h_{l-1}^m(ar)\sqrt{\frac{l}{2l+1}}\sum_{\nu=-l+1}^{l-1}\gamma_{l-1,\nu,\alpha}^{lm_l} Y_{l-1,\nu}(\widehat{\mathbf{r}}) + h_{l+1}^m(ar)\sqrt{\frac{l+1}{2l+1}}\sum_{\nu=-l-1}^{l+1}\gamma_{l+1,\nu,\alpha}^{lm_l} Y_{l+1,\nu}(\widehat{\mathbf{r}}) \,. \tag{S.208}$$

## S.5. ACOUSTIC SUM RULE ON DENSITY DERIVATIVES AND PULAY-LIKE CORRECTIONS

Let us consider the electron density $n_e(\mathbf{r};\{\boldsymbol{\tau}_{rl}\})$ as a function of the position vector $\mathbf{r}$, parametrically dependent on the set of nuclear positions $\boldsymbol{\tau}_{rl} = \boldsymbol{\tau}_{rl}^0 + \Delta\boldsymbol{\tau}_{rl}$, where $\boldsymbol{\tau}_{rl}^0$ represents the equilibrium position of the $r$-th nucleus in the $l$-th unit cell, identified by the lattice vector $\mathbf{R}_l$ within the BvK macrocrystal, and $\Delta\boldsymbol{\tau}_{rl}$ denotes the displacement from equilibrium. Note that the electron density exhibits a parametric dependence on the nuclear positions if and only if $n_e(\mathbf{r};\{\boldsymbol{\tau}_{rl}\})$ corresponds to the ground-state density. This holds both in equilibrium and in the presence of residual forces, as long as the electronic state remains adiabatically connected to the ground state. In contrast, in an out-of-equilibrium regime, the electronic and nuclear dynamics are no longer parametrically coupled. Therefore, for a ground-state electron density we express its total differential form as

$$dn_e(\mathbf{r};\{\boldsymbol{\tau}_{rl}\}) = \sum_\alpha \Bigg( \frac{\partial n_e(\mathbf{r})}{\partial r_\alpha}\bigg|_{\{\boldsymbol{\tau}_{tn}\}} dr_\alpha + \\ + \sum_{rl} \frac{\partial n_e(\mathbf{r})}{\partial \tau_{rl\alpha}}\bigg|_{\mathbf{r},\{tn\}\neq rl} d\tau_{rl\alpha}\Bigg). \tag{S.209}$$

It is important to note that in this context, the out-of-equilibrium nuclear positions $\boldsymbol{\tau}_{rl}$ are parameters and are not dependent on the position vector, i.e. $\partial\tau_{rl\alpha}/\partial r_\beta = 0$.

For a uniform translation of the nuclei within the BvK macrocrystal, where $d\mathbf{r} = d\boldsymbol{\tau}_{rl} = \boldsymbol{\delta}$, the translational invariance of the electron density implies $dn_e(\mathbf{r};\{\boldsymbol{\tau}_{rl}\}) = 0$ or equivalently,

$$\sum_\alpha \Bigg( \frac{\partial n_e(\mathbf{r})}{\partial r_\alpha}\bigg|_{\{\boldsymbol{\tau}_{tn}\}} + \sum_{rl} \frac{\partial n_e(\mathbf{r})}{\partial \tau_{rl\alpha}}\bigg|_{\mathbf{r},\{tn\}\neq rl}\Bigg)\delta_\alpha = 0\,. \tag{S.210}$$

Given that this condition must hold for any arbitrary displacement $\delta_\alpha$, the equality is satisfied if and only if the following sum rule is valid

$$\frac{\partial n_e(\mathbf{r})}{\partial r_\alpha}\bigg|_{\{\boldsymbol{\tau}_{tn}\}} = -\sum_{rl} \frac{\partial n_e(\mathbf{r})}{\partial \tau_{rl\alpha}}\bigg|_{\mathbf{r},\{tn\}\neq rl} \quad \forall\,\alpha\,. \tag{S.211}$$

The right-hand side of Eq. (S.211) can be recast using linear response theory, resulting in

$$\frac{\partial n_e(\mathbf{r})}{\partial \tau_{rl\alpha}} = \int_\Omega d\mathbf{r}'\chi_e(\mathbf{r},\mathbf{r}')\,\frac{\partial V_{rl}(\mathbf{r}')}{\partial \tau_{rl\alpha}}\bigg|_{\boldsymbol{\tau}_{rl}^0} \\ = -\int_\Omega d\mathbf{r}'\chi_e(\mathbf{r},\mathbf{r}')\frac{\partial V_{rl}^{(0)}(\mathbf{r}')}{\partial r'_\alpha}\,, \tag{S.212}$$

where we used the identity $\partial v(\mathbf{r}-\boldsymbol{\tau}_{rl})/\partial\tau_{rl\alpha} = -\nabla_\alpha v(\mathbf{r}-\boldsymbol{\tau}_{rl})$, and $\chi_e$ denotes the static reducible electronic polarizability, defined in symbolic notation as $\varepsilon_e^{-1} = 1 + v\chi_e$. In Eq. (S.212), the derivative of the out-of-equilibrium potential $V_{rl}$ with respect to nuclear displacements must be evaluated at equilibrium nuclear positions $\{\boldsymbol{\tau}_{rl}^0\}$. Similarly, the nuclear gradient of the electron density should also be computed at equilibrium nuclear positions. However, for the sake of clarity and to avoid overly complex notation, this dependence is not explicitly indicated. By combining Eqs. (S.212) and (S.211) we then obtain

$$\frac{\partial n_e(\mathbf{r})}{\partial r_\alpha} = \sum_{rl}\int_\Omega d\mathbf{r}'\chi_e(\mathbf{r},\mathbf{r}')\frac{\partial V_{rl}^{(0)}(\mathbf{r}')}{\partial r'_\alpha}\,, \tag{S.213}$$

which corresponds to Eq. (61) in the main text.

The acoustic sum rule (S.213) can also be alternately derived following the approach of Gillis[20], who considers an infinitesimal translation of the electronic coordinates generated by the total momentum operator. Using the fluctuation theorem and the response function formalism, he establishes a sum rule that ensures the correct acoustic behavior of the system at long wavelengths.

The sum rules in Eqs. (S.211) and (S.213) form the foundation for further analysis. As discussed in Sec. IIIA of the main text, the wave functions $\psi_{n,\mathbf{k}}$ are linear combinations of the basis functions $\{\chi_{\boldsymbol{\tau}Lj}^{\mathbf{k}}\}$, which are Bloch-summed versions of smooth Hankel envelope functions. Specifically, $\psi_{n,\mathbf{k}}(\mathbf{r}) = \sum_{\boldsymbol{\tau}Lj} z_{\boldsymbol{\tau}Lj,n}^{\mathbf{k}}\chi_{\boldsymbol{\tau}Lj}^{\mathbf{k}}(\mathbf{r})$, where $\boldsymbol{\tau}$ identifies the nuclear site where the $j$-th envelope function is centered within the primitive unit cell with angular momentum $L = lm$. The electron density, $n_e = (1/N_{\mathbf{k}})\sum_n\sum_{\mathbf{k}\in\mathrm{BZ}} f_{n,\mathbf{k}}|\psi_{n,\mathbf{k}}|^2$, can thus be written as

$$n_e(\mathbf{r}) = \frac{1}{N_{\mathbf{k}}} \sum_{\mathbf{k}\in \mathrm{BZ}} \sum_{\substack{\boldsymbol{\tau} Lj \\ \boldsymbol{\tau}' L' j'}} \sum_{n} f_{n,\mathbf{k}} z^{\mathbf{k}}_{\boldsymbol{\tau} Lj,n} z^{\mathbf{k}*}_{\boldsymbol{\tau}' L' j',n} \chi^{\mathbf{k}}_{\boldsymbol{\tau} Lj}(\mathbf{r}) \chi^{\mathbf{k}*}_{\boldsymbol{\tau}' L' j'}(\mathbf{r}) \,. \tag{S.214}$$

Here, the occupation numbers $f_{n,\mathbf{k}}$ are assumed to be independent of the nuclear positions $\{\boldsymbol{\tau}\}$, and the summation over $\boldsymbol{\tau}$ is restricted to the nuclear sites within the primitive unit cell, since adding a lattice vector $\mathbf{R}$ satisfies the condition $\chi^{\mathbf{k}}_{\boldsymbol{\tau}+\mathbf{R}Lj}(\mathbf{r}) = e^{-i\mathbf{k}\cdot\mathbf{R}} \chi^{\mathbf{k}}_{\boldsymbol{\tau} Lj}(\mathbf{r})$, and the phase factor cancels exactly with the corresponding phase from $z^{\mathbf{k}}_{\boldsymbol{\tau}+\mathbf{R}Lj,n}$. The partial derivative of the electron density with respect to a nuclear position, e.g. $\boldsymbol{\tau}_{rl}$, can then be expressed as

$$\begin{aligned}\frac{\partial n_e(\mathbf{r})}{\partial \tau_{rl\alpha}} &= \sum_n \sum_{\mathbf{k}\in \mathrm{BZ}} \sum_{Lj} \frac{\partial n_e(\mathbf{r})}{\partial z^{\mathbf{k}}_{\boldsymbol{\tau}_r Lj,n}} \frac{\partial z^{\mathbf{k}}_{\boldsymbol{\tau}_r Lj,n}}{\partial \tau_{rl\alpha}} + \sum_{\mathbf{k}\in \mathrm{BZ}} \sum_{Lj} \int_\Omega d\mathbf{r}' \frac{\delta n_e(\mathbf{r})}{\delta \chi^{\mathbf{k}}_{\boldsymbol{\tau}_r Lj}(\mathbf{r}')} \frac{\partial \chi^{\mathbf{k}}_{\boldsymbol{\tau}_r Lj}(\mathbf{r}')}{\partial \tau_{rl\alpha}} \\ &= \left.\frac{\partial n_e(\mathbf{r})}{\partial \tau_{rl\alpha}}\right|_{\{\boldsymbol{\chi}^{\mathbf{k}}\}} + \left.\frac{\partial n_e(\mathbf{r})}{\partial \tau_{rl\alpha}}\right|_{\{\boldsymbol{z}^{\mathbf{k}}\}}\end{aligned} \tag{S.215}$$

where

$$\left.\frac{\partial n_e(\mathbf{r})}{\partial \tau_{rl\alpha}}\right|_{\{\boldsymbol{\chi}^{\mathbf{k}}\}} = \frac{2\delta_{l0}}{N_{\mathbf{k}}} \sum_{\mathbf{k}\in \mathrm{BZ}} \sum_{\substack{Lj \\ \boldsymbol{\tau}' L' j'}} \sum_n f_{n,\mathbf{k}} \mathrm{Re}\left[\frac{\partial z^{\mathbf{k}}_{\boldsymbol{\tau}_r Lj,n}}{\partial \tau_{r\alpha}} z^{\mathbf{k}*}_{\boldsymbol{\tau}' L' j',n} \chi^{\mathbf{k}}_{\boldsymbol{\tau}_r Lj}(\mathbf{r}) \chi^{\mathbf{k}*}_{\boldsymbol{\tau}' L' j'}(\mathbf{r})\right] \tag{S.216}$$

$$\left.\frac{\partial n_e(\mathbf{r})}{\partial \tau_{rl\alpha}}\right|_{\{\boldsymbol{z}^{\mathbf{k}}\}} = \frac{2\delta_{l0}}{N_{\mathbf{k}}} \sum_{\mathbf{k}\in \mathrm{BZ}} \sum_{\substack{Lj \\ \boldsymbol{\tau}' L' j'}} \sum_n f_{n,\mathbf{k}} \mathrm{Re}\left[z^{\mathbf{k}}_{\boldsymbol{\tau}_r Lj,n} z^{\mathbf{k}*}_{\boldsymbol{\tau}' L' j',n} \frac{\partial \chi^{\mathbf{k}}_{\boldsymbol{\tau}_r Lj}(\mathbf{r})}{\partial \tau_{r\alpha}} \chi^{\mathbf{k}*}_{\boldsymbol{\tau}' L' j'}(\mathbf{r})\right] . \tag{S.217}$$

Note that Eq. (S.217) is a kind of *Pulay-like incomplete-basis-set correction* (IBC), which arises from the parametric dependence of the LMTO basis functions on the nuclear positions. Consequently, we can rewrite the sum rule (S.211) as

$$\begin{aligned}\frac{\partial n_e(\mathbf{r})}{\partial r_\alpha} = &-2 \sum_{\mathbf{k}\in \mathrm{BZ}} \sum_{\substack{\boldsymbol{\tau}_r Lj \\ \boldsymbol{\tau}' L' j'}} \sum_n f_{n,\mathbf{k}} \mathrm{Re}\left[\frac{\partial z^{\mathbf{k}}_{\boldsymbol{\tau}_r Lj,n}}{\partial \tau_{r\alpha}} z^{\mathbf{k}*}_{\boldsymbol{\tau}' L' j',n} \chi^{\mathbf{k}}_{\boldsymbol{\tau}_r Lj}(\mathbf{r}) \chi^{\mathbf{k}*}_{\boldsymbol{\tau}' L' j'}(\mathbf{r})\right] - \\ &-2 \sum_{\mathbf{k}\in \mathrm{BZ}} \sum_{\substack{\boldsymbol{\tau}_r Lj \\ \boldsymbol{\tau}' L' j'}} \sum_n f_{n,\mathbf{k}} \mathrm{Re}\left[z^{\mathbf{k}}_{\boldsymbol{\tau}_r Lj,n} z^{\mathbf{k}*}_{\boldsymbol{\tau}' L' j',n} \frac{\partial \chi^{\mathbf{k}}_{\boldsymbol{\tau}_r Lj}(\mathbf{r})}{\partial \tau_{r\alpha}} \chi^{\mathbf{k}*}_{\boldsymbol{\tau}' L' j'}(\mathbf{r})\right] ,\end{aligned} \tag{S.218}$$

which is fully defined within the primitive unit cell. Equation (S.218) illustrates that the $\alpha$-th component of the gradient $\nabla n_e$ of the electron density, which is explicitly free from Pulay-like IBCs when computed using an alternative approach to the acoustic sum rule (S.211), is nevertheless defined in terms of a Pulay-like IBC on the right-hand side. This correction term is not necessarily zero and plays a crucial role in accurately capturing the derivative of the electron density with respect to nuclear displacements. In addition to the perturbation responsible for changes in the wave function, Eqs. (S.215) and (S.218) also account for the contributions arising from variations in the basis set. In contrast, Eq. (S.212) is no longer satisfied, as linear response theory now provides an equivalent result only when the basis set is assumed to remain constant with respect to nuclear displacements

$$\begin{aligned}\left.\frac{\partial n_e(\mathbf{r})}{\partial \tau_{rl\alpha}}\right|_{\{\boldsymbol{\chi}^{\mathbf{k}}\}} &= \int_\Omega d\mathbf{r}' \frac{\delta n_e(\mathbf{r})}{\delta V_n(\mathbf{r}')} \frac{\partial V_n(\mathbf{r}')}{\partial \tau_{rl\alpha}} \\ &= -\int_\Omega d\mathbf{r}' \chi_e(\mathbf{r},\mathbf{r}') \frac{\partial V^{(0)}_{rl}(\mathbf{r}')}{\partial r'_\alpha} \,.\end{aligned} \tag{S.219}$$

Expression (S.219) captures the response of the electron density to external perturbations and does not involve explicit nuclear displacements in the LMTO basis functions. Within linear response theory, $V_n = \sum_{rl} V^{(0)}_{rl}$ is understood as an external field coupling with the electrons, and the definition for the static reducible electronic polarizability, $\chi_e(\mathbf{r},\mathbf{r}') = \delta n_e(\mathbf{r})/\delta V_n(\mathbf{r}')$, has been applied. By combining Eqs. (S.215) and (S.219), we obtain

$$\frac{\partial n_e(\mathbf{r})}{\partial \tau_{rl\alpha}} = -\int_\Omega d\mathbf{r}' \chi_e(\mathbf{r},\mathbf{r}') \frac{\partial V^{(0)}_{rl}(\mathbf{r}')}{\partial r'_\alpha} + \left.\frac{\partial n_e(\mathbf{r})}{\partial \tau_{rl\alpha}}\right|_{\{\boldsymbol{z}^{\mathbf{k}}\}} , \tag{S.220}$$

and the sum rule (S.213) is transformed into

$$\frac{\partial n_e(\mathbf{r})}{\partial r_\alpha} = \sum_{rl}\int_\Omega d\mathbf{r}'\chi_e(\mathbf{r},\mathbf{r}')\frac{\partial V^{(0)}_{rl}(\mathbf{r}')}{\partial r'_\alpha} - \sum_{rl}\frac{\partial n_e(\mathbf{r})}{\partial \tau_{rl\alpha}}\bigg|_{\{\boldsymbol{z}^{\mathbf{k}}\}}, \tag{S.221}$$

which corresponds to Eq. (S.218), with the first term reformulated within the framework of linear response theory. It is worth noting that Gillis's proof of the acoustic sum rule in Ref. 21 also has potential limitations arising from the incompleteness of the basis functions due to their explicit dependence on nuclear coordinates. This stems from the fact that, in this approach, the electron density is translated while the nuclei remain fixed in the lattice reference frame. However, this perspective is equivalent to considering a translating lattice reference frame while keeping the electron density fixed. Consequently, Pulay-like IBCs may emerge if the electron density is described using localized basis functions.

As discussed in the main text, the primary consequence of the sum rule (S.221), when affected by Pulay-like IBCs, is that the adiabatic phonon self-energy $\widetilde{\Pi}^{\mathrm{A}}_{r\alpha l,s\beta l'}$, given by Eq. (79) in the main text, does not satisfy the acoustic sum rule, yielding

$$\sum_{sl'}\widetilde{\Pi}^{\mathrm{A}}_{r\alpha l,s\beta l'} = -\sum_{tn}\int_\Omega d\mathbf{r}\frac{\partial V^{(0)}_{rl}(\mathbf{r})}{\partial r_\beta}\,\frac{\partial n_e(\mathbf{r})}{\partial \tau_{tn\alpha}}\bigg|_{\{\boldsymbol{z}^{\mathbf{k}}\}}, \tag{S.222}$$

which, however, should ideally vanish. In this section, we demonstrate that the aforementioned acoustic sum rule is indeed satisfied when the basis functions form a *complete set*. First, we observe that Eq. (S.222) can be reformulated as

$$\begin{aligned}\sum_{sl'}\widetilde{\Pi}^{\mathrm{A}}_{r\alpha l,s\beta l'} &= \sum_{tn}\int_\Omega d\mathbf{r}\,\frac{\partial V^{(0)}_{rl}(\mathbf{r})}{\partial \tau_{rl\beta}}\bigg|_{\boldsymbol{\tau}^0_{rl}}\frac{\partial n_e(\mathbf{r})}{\partial \tau_{tn\alpha}}\bigg|_{\{\boldsymbol{z}^{\mathbf{k}}\}}\\ &= \sum_{tn}\int_\Omega d\mathbf{r}\,\frac{\partial V^{(0)}_{rl}(\mathbf{r})}{\partial \tau_{rl\beta}}\bigg|_{\boldsymbol{\tau}^0_{rl}}\left(\frac{\partial n_e(\mathbf{r})}{\partial \tau_{tn\alpha}} - \frac{\partial n_e(\mathbf{r})}{\partial \tau_{tn\alpha}}\bigg|_{\{\boldsymbol{\chi}^{\mathbf{k}}\}}\right),\end{aligned} \tag{S.223}$$

by employing the identity $\partial v(\mathbf{r}-\boldsymbol{\tau}_{rl})/\partial\tau_{rl\alpha} = -\nabla_\alpha v(\mathbf{r}-\boldsymbol{\tau}_{rl})$, along with Eq. (S.215). The integrals in this equation can then be associated with the differentiation of the *Hellmann-Feynman forces* $\boldsymbol{F}_{rl}$, which takes the form

$$F_{rl\beta} = -\frac{\partial E_0(\{\boldsymbol{\tau}_{sp}\})}{\partial \tau_{rl\beta}}\bigg|_{\boldsymbol{\tau}^0_{rl}} = -\langle\Psi_0(\{\boldsymbol{\tau}^0_{sp}\})|\,\partial_{\tau_{rl\beta}}\hat{H}(\{\boldsymbol{\tau}^0_{sp}\})\,|\Psi_0(\{\boldsymbol{\tau}^0_{sp}\})\rangle\,, \tag{S.224}$$

i.e. as expectation value of the variation of the Born-Oppenheimer (BO) Hamiltonian for a system of interacting electrons moving within the field of fixed nuclei, characterized by the ground-state energy $E_0$ and many-body wave function $\Psi_0$. The BO energy and Hamiltonian depend parametrically on the nuclear positions, with the latter depending on $\{\boldsymbol{\tau}^0_{sp}\}$ exclusively through the electron-nuclear and nuclear-nuclear potential operators. Here, $\partial_{\tau_{rl\beta}}$ is shorthand notation for the partial derivative with respect to the nuclear position $\boldsymbol{\tau}_{rl}$ in the $\beta$-th direction. The derivative of the Hellmann-Feynman forces can thus be expressed as

$$\begin{aligned}\frac{\partial F_{rl\beta}}{\partial \tau_{tn\alpha}} =& -\langle\Psi_0(\{\boldsymbol{\tau}^0_{sp}\})|\,\partial_{\tau_{rl\beta}}\partial_{\tau_{tn\alpha}}\hat{H}(\{\boldsymbol{\tau}^0_{sp}\})\,|\Psi_0(\{\boldsymbol{\tau}^0_{sp}\})\rangle -\\ &-2\sum_{m\neq 0}\frac{\langle\Psi_0(\{\boldsymbol{\tau}^0_{sp}\})|\,\partial_{\tau_{rl\beta}}\hat{H}(\{\boldsymbol{\tau}^0_{sp}\})\,|\Psi_m(\{\boldsymbol{\tau}^0_{sp}\})\rangle\langle\Psi_m(\{\boldsymbol{\tau}^0_{sp}\})|\,\partial_{\tau_{tn\alpha}}\hat{H}(\{\boldsymbol{\tau}^0_{sp}\})\,|\Psi_0(\{\boldsymbol{\tau}^0_{sp}\})\rangle}{E_0(\{\boldsymbol{\tau}^0_{sp}\}) - E_m(\{\boldsymbol{\tau}^0_{sp}\})}.\end{aligned} \tag{S.225}$$

It is important to note that Eqs. (S.224) and (S.225) have been derived under the assumption of a complete basis set. Alternatively, when assuming an incomplete basis set, the forces are defined as $F_{rl\beta} = F^{(0)}_{rl\beta} + P^{(1)}_{rl\beta}$, with $F^{(0)}_{rl\beta}$ given by Eq. (S.224) and $P^{(1)}_{rl\beta}$ representing the Pulay force correction [21]. By differentiating this force and recognizing that $n_e = \Psi_0^*\Psi_0$, the derivative of the Hellmann-Feynman forces becomes

$$-\frac{\partial F_{rl\beta}}{\partial \tau_{tn\alpha}} = \int_\Omega d\mathbf{r}\,\frac{\partial V^{(0)}_{rl}(\mathbf{r})}{\partial \tau_{rl\beta}}\bigg|_{\boldsymbol{\tau}^0_{rl}}\frac{\partial n_e(\mathbf{r})}{\partial \tau_{tn\alpha}} + \delta_{rt}\delta_{ln}\int_\Omega d\mathbf{r}\,n_e(\mathbf{r})\,\frac{\partial^2 V^{(0)}_{rl}(\mathbf{r})}{\partial \tau_{rl\beta}\partial \tau_{rl\alpha}}\bigg|_{\boldsymbol{\tau}^0_{rl}} + \frac{\partial^2\langle\hat{U}_{nn}(\{\boldsymbol{\tau}_{sp}\})\rangle}{\partial \tau_{rl\beta}\partial \tau_{tn\alpha}}\bigg|_{\{\boldsymbol{\tau}^0_{rl}\}} + \frac{\partial P^{(1)}_{rl\beta}}{\partial \tau_{tn\alpha}}\bigg|_{\boldsymbol{\tau}^0_{rl}} + P^{(2)}_{rl\beta,tn\alpha}, \tag{S.226}$$

where the first term on the right-hand side includes Pulay-like IBCs, which stem from the parametric dependence of the basis functions on the nuclear positions. $P^{(2)}_{rl\beta,tn\alpha}$ accounts for the Pulay corrections arising from the application of the completeness relation $\sum_m|\Psi_m\rangle\langle\Psi_m| = 1$ when reformulating the linear response term in Eq. (S.225). Equation (S.226) thus provides an alternative definition of the interatomic force constants (IFCs), wherein the third-to-last term on the right-hand side denotes the nuclear contribution to the IFCs, i.e., the second derivative of the expectation value of the nuclear-nuclear interaction operator $\langle\hat{U}_{nn}(\boldsymbol{\tau}_{sp})\rangle$, evaluated at equilibrium positions. In contrast, when

differentiating the Hellmann-Feynman forces while keeping the basis functions constant, we have

$$-\left.\frac{\partial F_{rl\beta}}{\partial \tau_{tn\alpha}}\right|_{\{\boldsymbol{\chi}^{\mathbf{k}}\}} = \int_\Omega d\mathbf{r}\left.\frac{\partial V^{(0)}_{rl}(\mathbf{r})}{\partial \tau_{rl\beta}}\right|_{\boldsymbol{\tau}^0_{rl}}\left.\frac{\partial n_e(\mathbf{r})}{\partial \tau_{tn\alpha}}\right|_{\{\boldsymbol{\chi}^{\mathbf{k}}\}} + \delta_{rt}\delta_{ln}\int_\Omega d\mathbf{r}\, n_e(\mathbf{r})\left.\frac{\partial^2 V^{(0)}_{rl}(\mathbf{r})}{\partial \tau_{rl\beta}\partial \tau_{rl\alpha}}\right|_{\boldsymbol{\tau}^0_{rl}} + \\ + \left.\frac{\partial^2\langle \hat{U}_{nn}(\{\boldsymbol{\tau}^0_{sp}\})\rangle}{\partial \tau_{rl\beta}\partial \tau_{tn\alpha}}\right|_{\{\boldsymbol{\tau}^0_{rl}\}} + \left.\frac{\partial P^{(1)}_{rl\beta}}{\partial \tau_{tn\alpha}}\right|_{\{\boldsymbol{\chi}^{\mathbf{k}}\}}. \tag{S.227}$$

By combining Eqs. (S.223), (S.226), and (S.227), we obtain

$$\sum_{sl'}\widetilde{\Pi}^{\mathrm{A}}_{r\alpha l,s\beta l'} = \\ = -\sum_{tn}\left(\left.\frac{\partial F_{rl\beta}}{\partial \tau_{tn\alpha}}\right|_{\{\boldsymbol{z}^{\mathbf{k}}\}} + \left.\frac{\partial P^{(1)}_{rl\beta}}{\partial \tau_{tn\alpha}}\right|_{\{\boldsymbol{z}^{\mathbf{k}}\}} + P^{(2)}_{rl\beta,tn\alpha}\right), \tag{S.228}$$

which is not necessarily guaranteed to sum to zero. However, recognizing that Pulay corrections $P^{(1)}_{rl\beta}$ and $P^{(2)}_{rl\beta,tn\alpha}$ vanish when the basis functions form a complete set, and that, under these conditions, $\partial F_{r\beta l}/\partial\tau_{t\alpha n}|_{\{\boldsymbol{z}^{\mathbf{k}}\}} = 0$ (as evident from Eq. (S.225)), the acoustic sum rule for the IFCs simplifies to

$$\sum_{sl'}\widetilde{\Pi}^{\mathrm{A}}_{r\alpha l,s\beta l'} = 0\,, \tag{S.229}$$

thus proving the intended result.

Finally, to conclude this section, we address the presence of Pulay-like IBCs in the computation of the screened bare nuclear potential. As detailed in Sec. V of the main text, the bare electron-nuclear potential is screneed by a spherically symmetric core density, leading to the screened potential $\widetilde{V}^{(0)}_{rl} = V^{(0)}_{rl} + V^c_{rl}$, where

$$V^c_{rl}(\mathbf{r}) = \int_{\Omega_r(\mathbf{R}_l)} d\mathbf{r}'\frac{n^c_{e,r}(\mathbf{r}')}{|\mathbf{r}-\mathbf{r}'-\boldsymbol{\tau}_r-\mathbf{R}_l|} \tag{S.230}$$

represents the potential generated by the spherically symmetric core density. Linear response theory provides a sum of two terms (see Sec. VI in the main text)

$$\left.\frac{\partial n^v_e(\mathbf{r})}{\partial \tau_{rl\alpha}}\right|_{\{\boldsymbol{\chi}^{\mathbf{k}}\}} = \int_\Omega d\mathbf{r}'\chi^v_e(\mathbf{r},\mathbf{r}')\left.\frac{\partial V^{(0)}_{rl}(\mathbf{r}')}{\partial \tau_{rl\alpha}}\right|_{\boldsymbol{\tau}^0_{rl}} + \\ + \int_\Omega d\mathbf{r}'\chi^v_e(\mathbf{r},\mathbf{r}')\left.\frac{\partial V^c_{rl}(\mathbf{r}')}{\partial \tau_{rl\alpha}}\right|_{\boldsymbol{\tau}^0_{rl}}, \tag{S.231}$$

where $n^v_e(\mathbf{r})$ denotes the density due to the valence electrons, defined through the decomposition $n_e(\mathbf{r}) = n^v_e(\mathbf{r}) + n^c_e(\mathbf{r})$, and where $\chi^v_e(\mathbf{r},\mathbf{r}')$ is the static reducible electronic polarizability with contributions from valence states only. Here, the second term depends on the spherically symmetric core density $n^c_{e,r}(\mathbf{r}) = n^c_{e,r}(r)Y_{00}(\widehat{\mathbf{r}})$, which is invariant under nuclear displacements, as its radial profile is assumed to remain unperturbed by such displacements. Consequently, the derivatives of the screened electron-nuclear potential can be recast as

$$\frac{\partial V^c_{rl}(\mathbf{r})}{\partial \tau_{rl\alpha}} = \int_{\Omega_r} d\mathbf{r}' n^c_{e,r}(\mathbf{r}')\frac{\partial}{\partial \tau_{rl\alpha}}\left(\frac{1}{|\mathbf{r}-\mathbf{r}'-\boldsymbol{\tau}_r-\mathbf{R}_l|}\right) \\ = -\frac{\partial V^c_{rl}(\mathbf{r})}{\partial r_\alpha}\,. \tag{S.232}$$

To evaluate the nuclear gradient of the core potential $V^c_{rl}(\mathbf{r})$, we use its form given in Eq. (156b) of the main text, rather than the equivalent expression in Eq. (156a), because the step function $\theta(s_r - |\mathbf{r}'-\boldsymbol{\tau}_r-\mathbf{R}_l|)$ introduces a discontinuity in its derivative. This violates the conditions required for the application of the *Leibniz integral rule* (or the *theorem of differentiation under the integral sign*), as the derivative of the integrand with respect to the nuclear position cannot be properly exchanged with the integral in Eq. (156a). Conversely, the form in Eq. (156b) ensures the validity of this operation, as no such discontinuity arises.

## S.6. *E-PH* MATRIX ELEMENTS FOR ACOUSTIC PHONON MODES IN THE LONG WAVELENGTH LIMIT

As highlighted in Sec. IIA of the main text, the *e-ph* matrix elements become ill-defined for acoustic phonon modes in the long-wavelength limit, since, under these conditions, the phonon frequency behaves as

$$\lim_{\mathbf{q}\to 0}\omega_{\mathbf{q}\nu} = v_\nu(\widehat{\mathbf{q}})|\mathbf{q}|\,, \tag{S.233}$$

where $v_\nu(\widehat{\mathbf{q}})$ denotes the velocity of acoustic waves associated with the $\nu$-th phonon mode in the direction $\widehat{\mathbf{q}} = \mathbf{q}/|\mathbf{q}|$. Consequently, the *e-ph* coupling function diverges as $g_{\mathbf{q}\nu}(\mathbf{r}) \sim 1/\sqrt{q}$ in this limit, potentially posing challenges in modeling *e-ph* coupling.

In this section we analyze the behavior of the *e-ph* coupling matrix element for acoustic phonon modes in the long-wavelength limit $\mathbf{q}\to 0$, with the aim of identifying the conditions under which the *e-ph* problem becomes ill-defined. A general definition for the *e-ph* matrix elements within the field-theoretic formalism is provided in Eqs. (75)-(77) of the main text. Here, however, we

adopt the KS-DFT framework, where the *e-ph* coupling function is defined as

$$g_{\mathbf{q}\nu}(\mathbf{r}) = \sum_{r\alpha}\sum_{l}\sqrt{\frac{\Omega_0}{2m_r\omega_{\mathbf{q}\nu}}}e^{i\mathbf{q}\cdot\mathbf{R}_l}e_{r\alpha,\nu}(\mathbf{q})\times \\ \times \left.\frac{\partial v^{\mathrm{KS}}(\mathbf{r}-\mathbf{R}_l)}{\partial\tau_{rl\alpha}}\right|_{\boldsymbol{\tau}^0_{rl}} . \quad \text{(S.234)}$$

In this expression, $m_r$ represents the mass of the $r$-th atom in the primitive unit cell, $\mathbf{R}_l$ is the lattice vector pointing to the $l$-th unit cell in the BvK macrocrystal, $e_{r\alpha,\nu}(\mathbf{q})$ denotes the components of the polarization vector $\boldsymbol{e}_\nu(\mathbf{q})$ associated with the $\nu$-th phonon mode with frequency $\omega_{\mathbf{q}\nu}$, and $v^{\mathrm{KS}}(\mathbf{r}) = v^{\mathrm{KS}}(\mathbf{r};\{\boldsymbol{\tau}_{rl}\})$ is the Kohn-Sham potential perturbed by a vibration of the nucleus located at equilibrium position $\boldsymbol{\tau}^0_r$ in the $l$-th unit cell. Notably, this expression is affected by Pulay-like IBCs due to the parametric dependence of the LMTO basis functions on the nuclear positions. Indeed, since the KS-DFT potential is a functional of the electron density, the following chain rule can be applied

$$\left.\frac{\partial v^{\mathrm{KS}}(\mathbf{r}-\mathbf{R}_l)}{\partial\tau_{rl\alpha}}\right|_{\boldsymbol{\tau}^0_{rl}} = \int_\Omega d\mathbf{r}'\,\frac{\delta v^{\mathrm{KS}}(\mathbf{r}-\mathbf{R}_l)}{\delta n_e(\mathbf{r}')}\left.\frac{\partial n_e(\mathbf{r}')}{\partial\tau_{rl\alpha}}\right|_{\boldsymbol{\tau}^0_{rl}} , \quad \text{(S.235)}$$

where the variation of the electron density resulting from nuclear displacements is given by Eq. (S.215), thereby revealing the dependence on the fictitious Pulay-like IBC term. However, in this section, we aim to derive an expression for investigating the short-range *e-ph* coupling matrix elements for acoustic phonon modes in the long wavelength limit $\mathbf{q}\to 0$, which can be readily accessed within the KS-DFT framework. Instead of relying on the KS-DFT formalism, we employ our Pulay-like IBCs-free field-theoretic approach to evaluate the *e-ph* matrix elements.

We now focus on the link between *e-ph* matrix elements and reduced *e-ph* matrix elements $\xi^{r\alpha}_{in}(\mathbf{q},\mathbf{k})$, given by

$$g_{in,\nu}(\mathbf{k},\mathbf{q}) = \sum_{r\alpha}\sqrt{\frac{\hbar}{2m_r\omega_{\mathbf{q}\nu}}}e_{r\alpha,\nu}(\mathbf{q})\,\xi^{r\alpha}_{in}(\mathbf{q},\mathbf{k}) . \quad \text{(S.236)}$$

The reduced *e-ph* matrix elements are defined within the KS-DFT level of theory as

$$\xi^{r\alpha}_{in}(\mathbf{q},\mathbf{k}) = \sum_l e^{i\mathbf{q}\cdot\mathbf{R}_l}\left\langle\psi_{i,\mathbf{k}+\mathbf{q}}\right|\partial_{\tau_{rl\alpha}}v^{\mathrm{KS}}\left|\psi_{n,\mathbf{k}}\right\rangle_{\Omega_0} , \quad \text{(S.237)}$$

where $\partial_{\tau_{rl\alpha}}$ denotes a shorthand notation for the partial derivative with respect to the nuclear position $\boldsymbol{\tau}^0_{rl}$ in the $\alpha$-th direction. For simplicity, we will focus on homonuclear crystals, i.e., crystals composed of a single element, and investigate the behavior of the following quantity:

$$\sqrt{\omega_{\mathbf{q}\nu}}g_{in,\nu}(\mathbf{k},\mathbf{q}) = \sqrt{\frac{\hbar}{2m}}\sum_{r\alpha}e_{r\alpha,\nu}(\mathbf{q})\,\xi^{r\alpha}_{in}(\mathbf{q},\mathbf{k}) . \quad \text{(S.238)}$$

This quantity remains finite for acoustic phonon modes in the $\mathbf{q}\to 0$ limit. The term $\sum_l e^{i\mathbf{q}\cdot\mathbf{R}_l}\partial_{\tau_{r\alpha l}}v^{\mathrm{KS}}$ exhibits Bloch function properties, following the periodicity of the crystal. Consequently, the integral over the primitive unit cell, as defined in Eq. (S.237), can be reformulated as an integral over the entire volume of the BvK supercell, $\Omega = N_{\mathbf{k}}\Omega_0$, yielding

$$\xi^{r\alpha}_{in}(\mathbf{q},\mathbf{k}) = \frac{1}{N_{\mathbf{k}}}\sum_l e^{i\mathbf{q}\cdot\mathbf{R}_l}\left\langle\psi_{i,\mathbf{k}+\mathbf{q}}\right|\partial_{\tau_{rl\alpha}}v^{\mathrm{KS}}\left|\psi_{n,\mathbf{k}}\right\rangle_{\Omega} , \quad \text{(S.239)}$$

where $N_{\mathbf{k}}$ represents the number of unit cells in the BvK macrocrystal, corresponding to the number of phonon wave vectors in the BZ. Focusing on the matrix element in Eq. (S.239), we perform a change of variables, $\mathbf{y} = \mathbf{r}-\mathbf{R}_l$

$$\int_\Omega d\mathbf{r}\,\psi^*_{i,\mathbf{k}+\mathbf{q}}(\mathbf{r})\partial_{\tau_{rl\alpha}}v^{\mathrm{KS}}(\mathbf{r}-\mathbf{R}_l)\psi_{n,\mathbf{k}}(\mathbf{r}) = \\ = \int_\Omega d\mathbf{y}\,\psi^*_{i,\mathbf{k}+\mathbf{q}}(\mathbf{y}+\mathbf{R}_l)\partial_{\tau_{rl\alpha}}v^{\mathrm{KS}}(\mathbf{y})\psi_{n,\mathbf{k}}(\mathbf{y}+\mathbf{R}_l) . \quad \text{(S.240)}$$

The wave functions, being Bloch functions, satisfy the condition

$$\begin{aligned}\psi_{n,\mathbf{k}}(\mathbf{r}+\mathbf{R}) &= u_{n,\mathbf{k}}(\mathbf{r}+\mathbf{R})e^{i\mathbf{k}\cdot(\mathbf{r}+\mathbf{R})}/\sqrt{N_{\mathbf{q}}} \\ &= \left[u_{n,\mathbf{k}}(\mathbf{r})e^{i\mathbf{k}\cdot\mathbf{r}}\right]e^{i\mathbf{k}\cdot\mathbf{R}}/\sqrt{N_{\mathbf{q}}} \\ &= \psi_{n,\mathbf{k}}(\mathbf{r})e^{i\mathbf{k}\cdot\mathbf{R}} ,\end{aligned} \quad \text{(S.241)}$$

where $u_{n,\mathbf{k}}(\mathbf{r}+\mathbf{R}) = u_{n,\mathbf{k}}(\mathbf{r})$ represents the periodic part of the wave function. Thus, the integral in Eq. (S.240) simplifies to

$$e^{-i\mathbf{q}\cdot\mathbf{R}}\int_\Omega d\mathbf{r}\,\psi^*_{i,\mathbf{k}+\mathbf{q}}(\mathbf{r})\partial_{\tau_{rl\alpha}}v^{\mathrm{KS}}(\mathbf{r})\psi_{n,\mathbf{k}}(\mathbf{r}) . \quad \text{(S.242)}$$

This allows the reduced *e-ph* matrix elements in Eq. (S.239) to be simplified as

$$\xi^{r\alpha}_{in}(\mathbf{q},\mathbf{k}) = \frac{1}{N_{\mathbf{k}}}\sum_l\left\langle\psi_{i,\mathbf{k}+\mathbf{q}}\right|\partial_{\tau_{rl\alpha}}v^{\mathrm{KS}}_0\left|\psi_{n,\mathbf{k}}\right\rangle_{\Omega} , \quad \text{(S.243)}$$

where $v^{\mathrm{KS}}_0$ denotes the KS potential evaluated for $\mathbf{R} = 0$, and the dependence on the lattice vector index $l$ is reduced to the nuclear position oscillation $\delta\tau_{rl\alpha}$.

In the long-wavelength limit $\mathbf{q} \to 0$, Eq. (S.238) becomes

$$\lim_{\mathbf{q}\to 0} \sqrt{\omega_{\mathbf{q}\nu}} g_{in,\nu}(\mathbf{k},\mathbf{q}) = \lim_{\mathbf{q}\to 0} \sqrt{\frac{\hbar}{2m}} \frac{1}{N_\mathbf{k}} \sum_{r\alpha} e_{r\alpha,\nu}(\mathbf{q}) \sum_{l} \langle \psi_{i,\mathbf{k}} | \, \partial_{\tau_{rl\alpha}} v_0^{\mathrm{KS}} \, | \psi_{n,\mathbf{k}} \rangle_\Omega \, , \tag{S.244}$$

where Eqs. (S.243) and (S.238) have been combined. We can further employ the Epstein generalization of the Hellmann-Feynman theorem[22]

$$\langle \psi_{i,\mathbf{k}} | \, \partial_{\tau_{rl\alpha}} v_0^{\mathrm{KS}} \, | \psi_{n,\mathbf{k}} \rangle_\Omega = \frac{\partial \varepsilon_{n\mathbf{k}}}{\partial \tau_{rl\alpha}} \delta_{in} - (\varepsilon_{i\mathbf{k}} - \varepsilon_{n\mathbf{k}}) \langle \psi_{i,\mathbf{k}} | \, \partial_{\tau_{rl\alpha}} \psi_{n,\mathbf{k}} \rangle_\Omega \tag{S.245}$$

to rewrite Eq. (S.244) as

$$\lim_{\mathbf{q}\to 0} \sqrt{\omega_{\mathbf{q}\nu}} g_{in,\nu}(\mathbf{k},\mathbf{q}) = \lim_{\mathbf{q}\to 0} \sqrt{\frac{\hbar}{2m}} \frac{1}{N_\mathbf{k}} \sum_{r\alpha} e_{r\alpha,\nu}(\mathbf{q}) \sum_{l} \left[ \frac{\partial \varepsilon_{n\mathbf{k}}}{\partial \tau_{rl\alpha}} \delta_{in} - (\varepsilon_{i\mathbf{k}} - \varepsilon_{n\mathbf{k}}) \langle \psi_{i,\mathbf{k}} | \, \partial_{\tau_{rl\alpha}} \psi_{n,\mathbf{k}} \rangle_\Omega \right] . \tag{S.246}$$

Focusing exclusively on acoustic phonon modes, we consider a specific $\bar{\nu}$-th acoustic phonon mode corresponding to a translation of the crystal along the direction of the polarization vector $\boldsymbol{e}_{r,\bar{\nu}} = \{e_{\bar{\nu}}, \, e_{\bar{\nu}}, \, e_{\bar{\nu}}\}$. This choice of acoustic polarization vector in the long-wavelength limit is arbitrary, as it depends on the diagonalization details of the dynamical matrix. Moreover, an acoustic phonon mode in this limit is purely translational, implying that all atoms in the crystal translate by the same amount and direction. Under this assumptions, we can then simplify Eq. (S.246) as

$$\lim_{\mathbf{q}\to 0} \sqrt{\omega_{\mathbf{q}\bar{\nu}}} g_{in,\bar{\nu}}(\mathbf{k},\mathbf{q}) = \sqrt{\frac{\hbar}{2m}} \frac{e_{\bar{\nu}}}{N_\mathbf{k}} \sum_{rl\alpha} \left[ \frac{\partial \varepsilon_{n\mathbf{k}}}{\partial \tau_{rl\alpha}} \delta_{in} - (\varepsilon_{i\mathbf{k}} - \varepsilon_{n\mathbf{k}}) \langle \psi_{i,\mathbf{k}} | \, \partial_{\tau_{rl\alpha}} \psi_{n,\mathbf{k}} \rangle_\Omega \right] . \tag{S.247}$$

### A. Diagonal components of the *e-ph* matrix

In the case of the diagonal components of the *e-ph* matrix $\boldsymbol{g}_{\bar{\nu}}(\mathbf{k},\mathbf{q})$ in the $\mathbf{q} \to 0$ limit, i.e., for $i = n$, Eq. (S.247) simplifies to

$$\lim_{\mathbf{q}\to 0} \sqrt{\omega_{\mathbf{q}\bar{\nu}}} g_{nn,\bar{\nu}}(\mathbf{k},\mathbf{q}) = \sqrt{\frac{\hbar}{2m}} \frac{e_{\bar{\nu}}}{N_\mathbf{k}} \sum_{rl\alpha} \frac{\partial \varepsilon_{n\mathbf{k}}}{\partial \tau_{rl\alpha}} \, . \tag{S.248}$$

Understanding the term $\sum_{r\alpha l} \partial_{\tau_{rl\alpha}} \varepsilon_{n\mathbf{k}}$ is essential to gaining insight into the behavior of $\lim_{\mathbf{q}\to 0} \sqrt{\omega_{\mathbf{q}\bar{\nu}}} g_{nn,\bar{\nu}}(\mathbf{k},\mathbf{q})$. The energy state $\varepsilon_{n\mathbf{k}}(\{\boldsymbol{\tau}_{tp}\})$ depends on the equilibrium positions and vibrations of all nuclei in the crystal. For small nuclear oscillations along specific phonon modes, it can be expanded in a Taylor series as

$$\varepsilon_{n\mathbf{k}}(\{\delta\boldsymbol{\tau}_{tp}\}) = \varepsilon^0_{n\mathbf{k}} + \sum_{rl\alpha} \delta\tau_{rl\alpha} \left( \frac{\partial \varepsilon_{n\mathbf{k}}}{\partial \tau_{rl\alpha}} \right)_{\{\boldsymbol{\tau}^0_{tp}\}} + \tfrac{1}{2} \sum_{rl\alpha} \sum_{sl'\beta} \delta\tau_{rl\alpha} \delta\tau_{sl'\beta} \left( \frac{\partial^2 \varepsilon_{n\mathbf{k}}}{\partial \tau_{rl\alpha} \partial \tau_{sl'\beta}} \right)_{\{\boldsymbol{\tau}^0_{tp}\}} + \dots \, , \tag{S.249}$$

where $\varepsilon^0_{n\mathbf{k}}$ is the energy state corresponding to the fixed nuclear frame in the crystal (i.e. without contributions from *zero-point motion*). For acoustic phonon modes in the long-wavelength limit $\mathbf{q} \to 0$, all nuclear displacements $\delta\tau_{rl\alpha}$ can be assumed to equal an arbitrary constant $\delta\tau$, transforming the Taylor expansion into

$$\varepsilon_{n\mathbf{k}}(\delta\boldsymbol{\tau}) = \varepsilon^0_{n\mathbf{k}} + \delta\tau \sum_{rl\alpha} \left( \frac{\partial \varepsilon_{n\mathbf{k}}}{\partial \tau_{rl\alpha}} \right)_{\{\boldsymbol{\tau}^0_{tp}\}} + \frac{\delta\tau^2}{2} \sum_{rl\alpha} \sum_{sl'\beta} \left( \frac{\partial^2 \varepsilon_{n\mathbf{k}}}{\partial \tau_{rl\alpha} \partial \tau_{sl'\beta}} \right)_{\{\boldsymbol{\tau}^0_{tp}\}} + \dots \, . \tag{S.250}$$

However, due to the translational symmetry of the crystal, the energy states remain unchanged, i.e., $\varepsilon_{n\mathbf{k}}(\delta\boldsymbol{\tau}) = \varepsilon^0_{n\mathbf{k}}$. From this expansion, we obtain

$$\delta\tau \sum_{rl\alpha} \left( \frac{\partial \varepsilon_{n\mathbf{k}}}{\partial \tau_{rl\alpha}} \right)_{\{\boldsymbol{\tau}^0_{tp}\}} + \frac{\delta\tau^2}{2} \sum_{rl\alpha} \sum_{sl'\beta} \left( \frac{\partial^2 \varepsilon_{n\mathbf{k}}}{\partial \tau_{rl\alpha} \partial \tau_{sl'\beta}} \right)_{\{\boldsymbol{\tau}^0_{tp}\}} + \dots = 0 \, . \tag{S.251}$$

Since the nuclear displacements $\delta\boldsymbol{\tau}$ are arbitrary, the above equality holds if and only if the following sum rules are valid

$$\sum_{rl\alpha} \left( \frac{\partial \varepsilon_{n\mathbf{k}}}{\partial \tau_{rl\alpha}} \right)_{\{\boldsymbol{\tau}^0_{tp}\}} = 0 \, ; \qquad \sum_{rl\alpha} \sum_{sl'\beta} \left( \frac{\partial^2 \varepsilon_{n\mathbf{k}}}{\partial \tau_{rl\alpha} \partial \tau_{sl'\beta}} \right)_{\{\boldsymbol{\tau}^0_{tp}\}} = 0 \, ; \qquad \dots \tag{S.252}$$

By combining the sum rule (S.252) with Eq. (S.248), one can readily show that the diagonal components of the *e-ph* matrix for a $\bar{\nu}$-th acoustic phonon mode in the long-wavelength limit obey the condition

$$\boxed{\lim_{\mathbf{q}\to 0} \sqrt{\omega_{\mathbf{q}\bar{\nu}}}\, g_{nn,\bar{\nu}}(\mathbf{k},\mathbf{q}) = 0 \quad \forall n, \mathbf{k}}\,, \tag{S.253}$$

which holds for all energy states that solve the KS-DFT eigenvalue problem and for all the electronic wave vectors $\mathbf{k}$. This implies that the diagonal components of the *e-ph* matrix corresponding to acoustic phonon modes do not diverge in the long-wavelength limit, but are exactly zero.

### B. Off-diagonal components of the *e-ph* matrix

In the case of off-diagonal components of the *e-ph* matrix, i.e., for $i \neq n$, Eq. (S.247) becomes

$$\lim_{\mathbf{q}\to 0} \sqrt{\omega_{\mathbf{q}\bar{\nu}}}\, g_{in,\bar{\nu}}(\mathbf{k},\mathbf{q}) = \sqrt{\frac{\hbar}{2m}\frac{e_{\bar{\nu}}}{N_{\mathbf{k}}}} (\varepsilon_{n\mathbf{k}} - \varepsilon_{i\mathbf{k}}) \sum_{rl\alpha} \langle \psi_{i,\mathbf{k}} | \, \partial_{\tau_{rl\alpha}} \psi_{n,\mathbf{k}} \rangle_\Omega \,. \tag{S.254}$$

First, it is important to note that the condition

$$\boxed{\lim_{\mathbf{q}\to 0} \sqrt{\omega_{\mathbf{q}\bar{\nu}}}\, g_{in,\bar{\nu}}(\mathbf{k},\mathbf{q}) = 0 \quad \text{for degenerate states only}}\,, \tag{S.255}$$

holds only in the case of degenerate states, i.e., when $\varepsilon_{n\mathbf{k}} = \varepsilon_{i\mathbf{k}}$. *In case of non-degenerate states it can be demonstrated that Eq. (S.254) is not guaranteed to be zero.* While it may vanish due to symmetry, depending on the symmetry properties of the electronic states $|i,\mathbf{k}\rangle$ and $|n,\mathbf{k}\rangle$, it generally will not be zero. As a result, the matrix elements $g_{in,\bar{\nu}}(\mathbf{k},\mathbf{q}\to 0)$, where $\varepsilon_{n\mathbf{k}} \neq \varepsilon_{i\mathbf{k}}$, may diverge for a given $\bar{\nu}$-th acoustic phonon mode. To demonstrate this, we need to show that the quantity $\sum_{rl\alpha} \partial_{\tau_{rl\alpha}} \psi_{n,\mathbf{k}}$ does not satisfy a sum rule analogous to the one for the energy state, i.e., Eq. (S.252). With this in mind, let us consider the wave function corresponding to the state $|n,\mathbf{k}\rangle$ as a function of all the nuclear positions and their displacements from equilibrium in the BvK macrocrystal. For small nuclear vibrations along specific phonon modes, the wave function can be expanded in a Taylor series as

$$\psi_{n\mathbf{k}}(\mathbf{r};\{\delta\boldsymbol{\tau}_{tp}\}) = \psi^0_{n\mathbf{k}}(\mathbf{r}) + \sum_{rl\alpha} \delta\tau_{rl\alpha} \left(\frac{\partial \psi_{n\mathbf{k}}(\mathbf{r})}{\partial \tau_{rl\alpha}}\right)_{\{\boldsymbol{\tau}^0_{tp}\}} + \tfrac{1}{2} \sum_{rl\alpha}\sum_{sl'\beta} \delta\tau_{rl\alpha}\delta\tau_{sl'\beta} \left(\frac{\partial^2 \psi_{n\mathbf{k}}(\mathbf{r})}{\partial \tau_{rl\alpha}\partial\tau_{sl'\beta}}\right)_{\{\boldsymbol{\tau}^0_{tp}\}} + \dots\,, \tag{S.256}$$

where $\psi^0_{n\mathbf{k}}$ is the wave function associated with the fixed nuclear frame in the crystal. As in Sec. S.6 A, we focus on acoustic phonon modes in the long-wavelength limit, where all nuclear displacements components $\delta\tau_{rl\alpha}$ are set equal to an arbitrary constant displacement $\delta\tau$, leading to

$$\psi_{n\mathbf{k}}(\mathbf{r}+\delta\boldsymbol{\tau}) = \psi^0_{n\mathbf{k}}(\mathbf{r}) + \delta\tau \sum_{rl\alpha} \left(\frac{\partial \psi_{n\mathbf{k}}(\mathbf{r})}{\partial \tau_{rl\alpha}}\right)_{\{\boldsymbol{\tau}^0_{tp}\}} + \frac{\delta\tau^2}{2} \sum_{rl\alpha}\sum_{sl'\beta} \left(\frac{\partial^2 \psi_{n\mathbf{k}}(\mathbf{r})}{\partial \tau_{rl\alpha}\partial\tau_{sl'\beta}}\right)_{\{\boldsymbol{\tau}^0_{tp}\}} + \dots\,, \tag{S.257}$$

Using the Bloch representation of the wave function—see first line in Eq. (S.241)—this expansion can be rewritten as

$$u_{n\mathbf{k}}(\mathbf{r}+\delta\boldsymbol{\tau}) - u^0_{n\mathbf{k}}(\mathbf{r})e^{-i\mathbf{k}\cdot\delta\boldsymbol{\tau}} = \delta\tau e^{-i\mathbf{k}\cdot\delta\boldsymbol{\tau}} \sum_{rl\alpha} \left(\frac{\partial u_{n\mathbf{k}}(\mathbf{r})}{\partial \tau_{rl\alpha}}\right)_{\boldsymbol{\tau}^0_{tp}\}} + \frac{\delta\tau^2}{2} e^{-i\mathbf{k}\cdot\delta\boldsymbol{\tau}} \sum_{rl\alpha}\sum_{sl'\beta} \left(\frac{\partial^2 u_{n\mathbf{k}}(\mathbf{r})}{\partial \tau_{rl\alpha}\partial\tau_{sl'\beta}}\right)_{\{\boldsymbol{\tau}^0_{tp}\}} + \dots\,, \tag{S.258}$$

where the difference on the left hand side equals zero if and only if $\delta\boldsymbol{\tau}$ coincides with a particular family of lattice vectors $\{\mathbf{R}\}$, i.e., under the following conditions: (i) $u_{n\mathbf{k}}(\mathbf{r}+\mathbf{R}) = u_{n\mathbf{k}}(\mathbf{r}) = u^0_{n\mathbf{k}}(\mathbf{r})$, and (ii) $\mathbf{k}\cdot\mathbf{R} = 0$, implying $\exp(-i\mathbf{k}\cdot\mathbf{R}) = 1$. In this specific case, Eq. (S.258) reduces to

$$R \sum_{rl\alpha} \left(\frac{\partial u_{n\mathbf{k}}(\mathbf{r})}{\partial \tau_{rl\alpha}}\right)_{\{\boldsymbol{\tau}^0_{tp}\}} + \frac{R^2}{2} \sum_{rl\alpha}\sum_{sl'\beta} \left(\frac{\partial^2 u_{n\mathbf{k}}(\mathbf{r})}{\partial \tau_{rl\alpha}\partial\tau_{sl'\beta}}\right)_{\{\boldsymbol{\tau}^0_{tp}\}} + \dots = 0\,, \tag{S.259}$$

where $R = \|\mathbf{R}\|$ is the module of the lattice vector $\mathbf{R}$. Note that this expression is zero, although all the coefficients may not vanish, as $R$ is not an arbitrary displacement. Therefore, it is not possible to define sum rules for the wave functions analogous to those found for the energy state. Consequently, Eq. (S.254) is not guaranteed to be zero in the case of non-degenerate states.

### C. Results within the field-theoretic approach: application to diamond

In this section, we present some results to validate the discussions from Sections S.6 A and S.6 B. To address potential issues arising from the gauge arbitrariness of degenerate electronic states and phonon modes, we compute the following quantity

$$G^2_{\{\bar{i}\},\{\bar{n}\}}(\mathbf{k}) = \lim_{\mathbf{q}\to 0} \omega_{\mathbf{q}\bar{\nu}} \sum_{\mu\in\{\bar{\nu}\}} \sum_{i\in\{\bar{i}\}} \sum_{n\in\{\bar{n}\}} |g^{\mathcal{S}}_{in,\mu}(\mathbf{k},\mathbf{q})|^2 \,. \tag{S.260}$$

This equation represents a summation over all degenerate acoustic phonon modes $\{\bar{\nu}\}$ and all degenerate electronic states within the manifolds $\{\bar{i}\}$ and $\{\bar{n}\}$. The short-range *e-ph* matrix elements $g^{\mathcal{S}}_{in,\mu}(\mathbf{k},\mathbf{q})$ are evaluated using the field-theoretic approach implemented in the `Questaal` electronic structure suite. The formalism for these calculations is detailed in Eqs. (75)-(77), (123), and (160).

In order to illustrate the cases discussed in Sec. S.6 A and S.6 B with a practical calculation, we apply this methodology to a diamond crystal model. The electronic structure calculations were performed within QS$GW$, using the RPA. Additionally, ladder diagrams were incorporated via a QS$G\widehat{W}$ scheme, as detailed in Sec. IIIC of the main text. In the QS$G\widehat{W}$ case, 11 unoccupied bands were included in the two-particle Hamiltonian within the BSE scheme, showing convergence of the electronic band structure. A $11^3$ **k**-point mesh and a kinetic energy cutoff of 6.2 Ry for the Coulomb interaction in the interstitial region yielded an optical gap accuracy of approximately 2 meV.

Lattice dynamical properties were computed using Density Functional Perturbation Theory (DFPT) within the *local-density approximation* (LDA) [23, 24], utilizing the `QUANTUM-ESPRESSO` code[25–27], as described in Sec. VI of the main text. A $12^3$ **k**-point mesh was used to sample the BZ along with a 150 Ry kinetic energy cutoff. Although we tested the convergence of the vibrational frequencies for the highest optical modes at $\mathbf{q} = \Gamma$, the phonon frequencies themselves are not required for the results presented here. Instead, the polarization vectors, which are predominantly determined by the crystal symmetry, are used to compute Eq. (S.260) within a field-theoretic framework.

Table I reports several cases and shows that the *diagonal components* $G^2_{\{\bar{n}\},\{\bar{n}\}}(\Gamma)$ are consistently zero, which includes both diagonal $\sum_{\mu\in\{\bar{\nu}\}} g^{\mathcal{S}}_{nn,\mu}(\mathbf{k},\Gamma)$ as well as off-diagonal $\sum_{\mu\in\{\bar{\nu}\}} g^{\mathcal{S}}_{in,\mu}(\mathbf{k},\Gamma)$ components for degenerate states, as for the top of the valence band ($\Gamma'_{25v}$) and the bottom of the conduction band ($\Gamma_{15c}$) at $\mathbf{k} = 0$. In contrast, as discussed in Sec. S.6 B, off-diagonal components can be non-zero in case of non-degenerate electronic states. This behavior is observed for both QS$GW$ and QS$G\widehat{W}$ calculations, showing comparable results, which indicates that the inclusion of ladder diagrams does not significantly impact the *e-ph* matrix elements. On the contrary, the electronic band structure is notably affected, with the optical gap renormalized from 8.18 eV to 7.73 eV when ladder diagrams are included in the inverse dielectric function via the QS$G\widehat{W}$ scheme. To match the experimental value of ∼7.1 eV [28], zero-point renormalizations [29, 30] will then need to be included.

TABLE I. The values of the quantity in Eq. (S.260) are presented for various initial and final electronic states involved in the *e-ph* scattering process. Results are shown for both QS$GW$ and QS$G\widehat{W}$ calculations, with the latter incorporating 11 unoccupied bands in constructing the two-particle Hamiltonian within the BSE framework.

| $\lvert i,\mathbf{k}\rangle$ | $\lvert n,\mathbf{k}\rangle$ | $G^2_{\{\bar{i}\},\{\bar{n}\}}(\Gamma)$ | |
|---|---|---|---|
| | | QS$GW$ | QS$G\widehat{W}$ |
| $\Gamma_1$ | $\Gamma_1$ | 0.000000000 | 0.000000000 |
| $\Gamma_1$ | $\Gamma'_{25v}$ | 0.000000000 | 0.000000000 |
| $\Gamma_1$ | $\Gamma_{15c}$ | 0.000072793 | 0.001537034 |
| $\Gamma'_{25v}$ | $\Gamma'_{25v}$ | 0.000000000 | 0.000000000 |
| $\Gamma'_{25v}$ | $\Gamma_{15c}$ | 0.021225925 | 0.021064804 |
| $\Gamma'_{25v}$ | $\Gamma^{+1}_{15c}$ | 0.051082865 | 0.066033834 |
| $\Gamma'_{25v}$ | $\Gamma^{+2}_{15c}$ | 0.000000000 | 0.000000000 |
| $\Gamma'_{25v}$ | $\Gamma^{+3}_{15c}$ | 0.772927365 | 0.774648402 |
| $\Gamma_{15c}$ | $\Gamma_{15c}$ | 0.000000000 | 0.000000000 |
| $\Gamma_{15c}$ | $\Gamma^{+1}_{15c}$ | 0.000000000 | 0.000000000 |
| $\Gamma_{15c}$ | $\Gamma^{+2}_{15c}$ | 0.075636882 | 0.080205652 |
| $\Gamma_{15c}$ | $\Gamma^{+3}_{15c}$ | 0.000000000 | 0.000000000 |
| $\Gamma_{15c}$ | $\Gamma^{+4}_{15c}$ | 0.406001929 | 0.390335995 |
| $\Gamma^{+1}_{15c}$ | $\Gamma^{+1}_{15c}$ | 0.000000000 | 0.000000000 |
| $\Gamma^{+2}_{15c}$ | $\Gamma^{+2}_{15c}$ | 0.000000000 | 0.000000000 |
| $\Gamma^{+3}_{15c}$ | $\Gamma^{+3}_{15c}$ | 0.000000000 | 0.000000000 |
| $\Gamma^{+4}_{15c}$ | $\Gamma^{+4}_{15c}$ | 0.000000000 | 0.000000000 |
| $\Gamma^{+5}_{15c}$ | $\Gamma^{+5}_{15c}$ | 0.000000000 | 0.000000000 |
| $\Gamma^{+6}_{15c}$ | $\Gamma^{+6}_{15c}$ | 0.000000000 | 0.000000000 |

## S.7. ON THE DERIVATION OF THE NUCLEAR CONTRIBUTION TO THE ADIABATIC PHONON SELF-ENERGY $\Pi^{\mathbf{A},i}_{r\alpha l,s\beta l'}$

In Sec. VI of the main text, we introduce the nuclear contribution to the adiabatic phonon self-energy as follows

$$\Pi^{\mathrm{A},i}_{r\alpha l,s\beta l'} = \left.\frac{\partial^2 \langle \hat{U}_{nn}(\{\boldsymbol{\tau}_{rl}\})\rangle}{\partial\tau_{rl\alpha}\partial\tau_{sl'\beta}}\right|_{\{\boldsymbol{\tau}^0_{rl}\}} . \tag{S.261}$$

In this section, we demonstrate Eq. (S.261) by employing the Fourier transform of the Coulomb kernel within a plane wave framework. Using the definition of the nuclear-nuclear interaction energy provided by Eq. (24)

of the main text, the second derivative on the right-hand side of Eq. (S.261) can be expressed as

$$\left.\frac{\partial^2 \langle \hat{U}_{nn}(\{\boldsymbol{\tau}_{rl}\})\rangle}{\partial \tau_{rl\alpha}\partial \tau_{sl'\beta}}\right|_{\{\boldsymbol{\tau}^0_{rl}\}} = \tfrac{e^2}{2}\sum_{t\neq p}\sum_{n\neq m} Z_t Z_p \left.\frac{\partial^2}{\partial \tau_{rl\alpha}\partial \tau_{sl'\beta}}\frac{1}{|\boldsymbol{\tau}_{tn}-\boldsymbol{\tau}_{pm}|}\right|_{\{\boldsymbol{\tau}^0_{rl}\}}, \tag{S.262}$$

where $\boldsymbol{\tau}_{tn} = \boldsymbol{\tau}^0_t + \mathbf{R}_n + \Delta\boldsymbol{\tau}_{tn}$. By employing the Fourier transform of the nuclear Coulomb kernel

$$\frac{1}{|\boldsymbol{\tau}_{tn}-\boldsymbol{\tau}_{pm}|} = \frac{1}{N_{\mathbf{k}}\Omega_0}\sum_{\mathbf{q}\in\mathrm{BZ}}\sum_{\mathbf{G}}\frac{4\pi}{|\mathbf{q}+\mathbf{G}|^2}e^{i(\mathbf{q}+\mathbf{G})\cdot(\boldsymbol{\tau}_{tn}-\boldsymbol{\tau}_{pm})}, \tag{S.263}$$

we can rewrite Eq. (S.262) as

$$\left.\frac{\partial^2 \langle \hat{U}_{nn}(\{\boldsymbol{\tau}_{rl}\})\rangle}{\partial \tau_{rl\alpha}\partial \tau_{sl'\beta}}\right|_{\{\boldsymbol{\tau}^0_{rl}\}} = \frac{2\pi e^2}{N_{\mathbf{k}}\Omega_0}\sum_{\mathbf{q}\in\mathrm{BZ}}\sum_{\mathbf{G}}\sum_{t\neq p}\sum_{n\neq m}\frac{Z_t Z_p}{|\mathbf{q}+\mathbf{G}|^2}\left\{\frac{\partial^2}{\partial \tau_{rl\alpha}\partial \tau_{sl'\beta}}e^{i(\mathbf{q}+\mathbf{G})\cdot(\boldsymbol{\tau}_{tn}-\boldsymbol{\tau}_{pm})}\right\}_{\{\boldsymbol{\tau}^0_{rl}\}} \tag{S.264}$$

where

$$\begin{aligned}
&\left\{\frac{\partial^2}{\partial \tau_{rl\alpha}\partial \tau_{sl'\beta}}e^{i(\mathbf{q}+\mathbf{G})\cdot(\boldsymbol{\tau}_{tn}-\boldsymbol{\tau}_{pm})}\right\}_{\{\boldsymbol{\tau}^0_{rl}\}} = i(\mathbf{q}+\mathbf{G})_\beta\left[\delta_{st}\delta_{l'n}-\delta_{sp}\delta_{l'm}\right]\left\{\frac{\partial}{\partial \tau_{rl\alpha}}e^{i(\mathbf{q}+\mathbf{G})\cdot(\boldsymbol{\tau}_{tn}-\boldsymbol{\tau}_{pm})}\right\}_{\{\boldsymbol{\tau}^0_{rl}\}}\\
&= -(\mathbf{q}+\mathbf{G})_\alpha(\mathbf{q}+\mathbf{G})_\beta\left[\delta_{st}\delta_{l'n}-\delta_{sp}\delta_{l'm}\right]\left[\delta_{rt}\delta_{ln}-\delta_{rp}\delta_{lm}\right]e^{i(\mathbf{q}+\mathbf{G})\cdot(\boldsymbol{\tau}^0_{tn}-\boldsymbol{\tau}^0_{pm})}\\
&= -(\mathbf{q}+\mathbf{G})_\alpha(\mathbf{q}+\mathbf{G})_\beta\left[\delta_{st}\delta_{l'n}\delta_{rt}\delta_{ln}-\delta_{st}\delta_{l'n}\delta_{rp}\delta_{lm}-\delta_{sp}\delta_{l'm}\delta_{rt}\delta_{ln}+\delta_{sp}\delta_{l'm}\delta_{rp}\delta_{lm}\right]e^{i(\mathbf{q}+\mathbf{G})\cdot(\boldsymbol{\tau}^0_{tn}-\boldsymbol{\tau}^0_{pm})}\,.
\end{aligned} \tag{S.265}$$

We can then restate Eq. (S.264) as follows

$$\left.\frac{\partial^2 \langle \hat{U}_{nn}(\{\boldsymbol{\tau}_{rl}\})\rangle}{\partial \tau_{rl\alpha}\partial \tau_{sl'\beta}}\right|_{\{\boldsymbol{\tau}^0_{rl}\}} = -\frac{2\pi e^2}{N_{\mathbf{k}}\Omega_0}\sum_{\mathbf{q}\in\mathrm{BZ}}\sum_{\mathbf{G}}\sum_{\eta=1}^{4}\frac{(\mathbf{q}+\mathbf{G})_\alpha(\mathbf{q}+\mathbf{G})_\beta}{|\mathbf{q}+\mathbf{G}|^2}\varrho^{sl'}_{rl,\eta}(\mathbf{q},\mathbf{G})\,, \tag{S.266}$$

with the coefficients $\varrho^{sl'}_{rl,\eta}(\mathbf{q},\mathbf{G})$ defined as

$$\begin{aligned}
\varrho^{sl'}_{rl,1}(\mathbf{q},\mathbf{G}) &= \sum_{t\neq p}\sum_{n\neq m} Z_t Z_p\,\delta_{rt}\delta_{nl}\delta_{st}\delta_{nl'}\,e^{i(\mathbf{q}+\mathbf{G})\cdot(\boldsymbol{\tau}^0_{tn}-\boldsymbol{\tau}^0_{pm})}\\
&= \delta_{rs}\delta_{ll'}\,Z_r\sum_{pm}Z_p\,e^{i(\mathbf{q}+\mathbf{G})\cdot(\boldsymbol{\tau}^0_{rl}-\boldsymbol{\tau}^0_{pm})}\,,
\end{aligned} \tag{S.267}$$

$$\begin{aligned}
\varrho^{sl'}_{rl,2}(\mathbf{q},\mathbf{G}) &= -\sum_{t\neq p}\sum_{n\neq m} Z_t Z_p\,\delta_{rp}\delta_{lm}\delta_{st}\delta_{nl'}\,e^{i(\mathbf{q}+\mathbf{G})\cdot(\boldsymbol{\tau}^0_{tn}-\boldsymbol{\tau}^0_{pm})}\\
&= -Z_r Z_s\,e^{i(\mathbf{q}+\mathbf{G})\cdot(\boldsymbol{\tau}^0_{rl}-\boldsymbol{\tau}^0_{sl'})}\,,
\end{aligned} \tag{S.268}$$

$$\begin{aligned}
\varrho^{sl'}_{rl,3}(\mathbf{q},\mathbf{G}) &= -\sum_{t\neq p}\sum_{n\neq m} Z_t Z_p\,\delta_{rt}\delta_{ln}\delta_{sp}\delta_{l'm}\,e^{i(\mathbf{q}+\mathbf{G})\cdot(\boldsymbol{\tau}^0_{tn}-\boldsymbol{\tau}^0_{pm})}\\
&= \left[\varrho^{sl'}_{rl,2}(\mathbf{q},\mathbf{G})\right]^* = \varrho^{sl'}_{rl,2}(-\mathbf{q},-\mathbf{G})
\end{aligned} \tag{S.269}$$

$$\begin{aligned}
\varrho^{sl'}_{rl,4}(\mathbf{q},\mathbf{G}) &= \sum_{t\neq p}\sum_{n\neq m} Z_t Z_p\,\delta_{rp}\delta_{lm}\delta_{sp}\delta_{l'm}\,e^{i(\mathbf{q}+\mathbf{G})\cdot(\boldsymbol{\tau}^0_{tn}-\boldsymbol{\tau}^0_{pm})}\\
&= \left[\varrho^{sl'}_{rl,1}(\mathbf{q},\mathbf{G})\right]^* = \varrho^{sl'}_{rl,1}(-\mathbf{q},-\mathbf{G})\,.
\end{aligned} \tag{S.270}$$

Combining Eqs. (S.266)-(S.270) and performing the substitution $\mathbf{q}+\mathbf{G} \to -(\mathbf{q}+\mathbf{G})$ for terms with $\eta = 3, 4$, which keeps the summation over wave vectors $\mathbf{q}$ and reciprocal lattice vectors $\mathbf{G}$ invariant, we obtain

$$\left.\frac{\partial^2 \langle \hat{U}_{nn}(\{\boldsymbol{\tau}_{rl}\})\rangle}{\partial \tau_{rl\alpha}\partial \tau_{sl'\beta}}\right|_{\{\boldsymbol{\tau}^0_{rl}\}} = -\frac{4\pi e^2}{N_{\mathbf{k}}\Omega_0}\sum_{\mathbf{q}\in\mathrm{BZ}}\sum_{\mathbf{G}}\frac{(\mathbf{q}+\mathbf{G})_\alpha(\mathbf{q}+\mathbf{G})_\beta}{|\mathbf{q}+\mathbf{G}|^2}\left\{\varrho^{sl'}_{rl,1}(\mathbf{q},\mathbf{G})+\varrho^{sl'}_{rl,2}(\mathbf{q},\mathbf{G})\right\}$$
$$= \frac{4\pi e^2}{N_{\mathbf{k}}\Omega_0}\sum_{pm}\Big(\delta_{ps}\delta_{ml'}-\delta_{rs}\delta_{ll'}\Big)Z_r Z_p \sum_{\mathbf{q}\in\mathrm{BZ}}\sum_{\mathbf{G}}\frac{(\mathbf{q}+\mathbf{G})_\alpha(\mathbf{q}+\mathbf{G})_\beta}{|\mathbf{q}+\mathbf{G}|^2}e^{i(\mathbf{q}+\mathbf{G})\cdot(\boldsymbol{\tau}^0_{rl}-\boldsymbol{\tau}^0_{pm})}, \quad \text{(S.271)}$$

which corresponds to the result presented in Ref. 31.

Now, we focus on the purely electrostatic contribution to the phonon self-energy given by Eq. (181) of the main text

$$\Pi^{\mathrm{A},i}_{r\alpha l,s\beta l'} = \sum_{pm}\Big(\delta_{ps}\delta_{ml'}-\delta_{rs}\delta_{ll'}\Big)\int_\Omega\int_\Omega \frac{\partial V^{(0)}_{rl}(\mathbf{r})}{\partial r_\beta}v^{-1}(\mathbf{r}-\mathbf{r}')\frac{\partial V^{(0)}_{pm}(\mathbf{r}')}{\partial r'_\alpha}\,d\mathbf{r}\,d\mathbf{r}'\,. \quad \text{(S.272)}$$

Here, we use the bare nuclear potential at equilibrium, $V^{(0)}_{rl}$, rather than the nuclear potential screened by core electrons, $\widetilde{V}^{(0)}_{rl}$, since the nuclear-nuclear interaction energy in Eq. (S.261) accounts for the repulsive interaction between nuclei in the absence of screening. Using the Fourier transform of the bare nuclear potential

$$V^{(0)}_{rl}(\mathbf{r}) = -\frac{eZ_r}{N_{\mathbf{k}}\Omega_0}\sum_{\mathbf{q}\in\mathrm{BZ}}\sum_{\mathbf{G}}\frac{4\pi}{|\mathbf{q}+\mathbf{G}|^2}e^{i(\mathbf{q}+\mathbf{G})\cdot(\mathbf{r}-\boldsymbol{\tau}_{rl})}\,, \quad \text{(S.273)}$$

we can rewrite Eq. (S.272) as

$$\Pi^{\mathrm{A},i}_{r\alpha l,s\beta l'} = \sum_{pm}\Big(\delta_{ps}\delta_{ml'}-\delta_{rs}\delta_{ll'}\Big)Z_p Z_r\left[\frac{e4\pi}{N_{\mathbf{k}}\Omega_0}\right]^2\sum_{\mathbf{q},\mathbf{q}'\in\mathrm{BZ}}\sum_{\mathbf{G},\mathbf{G}'}\frac{(\mathbf{q}+\mathbf{G})_\beta(\mathbf{q}'+\mathbf{G}')_\alpha}{|\mathbf{q}+\mathbf{G}|^2|\mathbf{q}'+\mathbf{G}'|^2}e^{-i(\mathbf{q}+\mathbf{G})\cdot\boldsymbol{\tau}^0_{rl}}e^{-i(\mathbf{q}'+\mathbf{G}')\cdot\boldsymbol{\tau}^0_{pm}}\times$$
$$\times\int_\Omega\int_\Omega e^{i(\mathbf{q}+\mathbf{G})\cdot\mathbf{r}}v^{-1}(\mathbf{r}-\mathbf{r}')e^{i(\mathbf{q}'+\mathbf{G}')\cdot\mathbf{r}'}\,d\mathbf{r}\,d\mathbf{r}'\,. \quad \text{(S.274)}$$

Using the Fourier transform result

$$\int_\Omega\int_\Omega e^{i(\mathbf{q}+\mathbf{G})\cdot\mathbf{r}}v^{-1}(\mathbf{r}-\mathbf{r}')e^{i(\mathbf{q}'+\mathbf{G}')\cdot\mathbf{r}'}\,d\mathbf{r}\,d\mathbf{r}' = \frac{N_{\mathbf{k}}\Omega_0}{4\pi}|\mathbf{q}+\mathbf{G}||\mathbf{q}'+\mathbf{G}'|\delta_{\mathbf{q},-\mathbf{q}'}\delta_{\mathbf{G},-\mathbf{G}'}\,, \quad \text{(S.275)}$$

we find that the nuclear phonon self-energy simplifies to

$$\Pi^{\mathrm{A},i}_{r\alpha l,s\beta l'} = \frac{e^2 4\pi}{N_{\mathbf{k}}\Omega_0}\sum_{pm}\Big(\delta_{ps}\delta_{ml'}-\delta_{rs}\delta_{ll'}\Big)Z_r Z_p\sum_{\mathbf{q}\in\mathrm{BZ}}\sum_{\mathbf{G}}\frac{(\mathbf{q}+\mathbf{G})_\beta(\mathbf{q}+\mathbf{G})_\alpha}{|\mathbf{q}+\mathbf{G}|^2}e^{i(\mathbf{q}+\mathbf{G})\cdot(\boldsymbol{\tau}^0_{rl}-\boldsymbol{\tau}^0_{pm})}\,, \quad \text{(S.276)}$$

which coincides with Eq. (S.271), thereby proving the equality (S.261).


[1] E. Bott, M. Methfessel, W. Krabs, and P. C. Schmidt, Journal of Mathematical Physics **39**, 3393 (1998).

[2] D. A. Varshalovich, A. N. Moskalev, and V. K. Khersonskii, *Quantum Theory of Angular Momentum* (WORLD SCIENTIFIC, 1988).

[3] D. Pashov, S. Acharya, W. R. Lambrecht, J. Jackson, K. D. Belashchenko, A. Chantis, F. Jamet, and M. van Schilfgaarde, Computer Physics Communications **249**, 107065 (2020).

[4] The condition $\boldsymbol{\tau}_i - \boldsymbol{\tau}_r = \mathbf{R}_p \neq 0$ cannot occur when $\boldsymbol{\tau}_i \neq \boldsymbol{\tau}_r$ since only the primitive unit cell is generally considered in electronic structure codes.

[5] D. B. Litvin and V. Kopský, Acta Crystallographica Section A **67**, 415 (2011).

[6] To derive identity (S.62), we first establish a related expression for the fractional translation vector $\boldsymbol{v}(\mathcal{S})$. This expression can be obtained by applying the space group symmetry operator and its inverse to a given nuclear position vector $\boldsymbol{\tau}_r$, as follow: $\{\mathbf{S}|\boldsymbol{v}\}\{\mathbf{S}|\boldsymbol{v}\}^{-1}\boldsymbol{\tau}_r = \{\mathbf{S}|\boldsymbol{v}\}\big[\mathbf{S}^{-1}\boldsymbol{\tau}_r + \boldsymbol{v}(\mathcal{S}^{-1})\big] = \boldsymbol{\tau}_r + \mathbf{S}\boldsymbol{v}(\mathcal{S}^{-1}) + \boldsymbol{v}(\mathcal{S})$, which

must reduce to $\boldsymbol{\tau}_r$. Enforcing this condition leads to the identity

$$\boldsymbol{v}(\mathcal{S}^{-1}) = -\mathbf{S}^{-1}\boldsymbol{v}(\mathcal{S})\,. \qquad \text{(S.277)}$$

To derive identity (S.62), we consider the rotation defined in Eq. (S.49) and the corresponding inverse rotation rule

$$\boldsymbol{\tau}_s = \{\mathbf{S}|\boldsymbol{v}\}^{-1}\boldsymbol{\tau}_r + \bar{\boldsymbol{v}}_{\boldsymbol{\tau}_r}(\mathcal{S}^{-1})\,. \qquad \text{(S.278)}$$

Substituting Eq. (S.278) into Eq. (S.49), we obtain

$$\boldsymbol{\tau}_r = \mathbf{S}\big[\mathbf{S}^{-1}\boldsymbol{\tau}_r + \boldsymbol{v}(\mathcal{S}^{-1}) + \bar{\boldsymbol{v}}_{\boldsymbol{\tau}_r}(\mathcal{S}^{-1})\big] + \boldsymbol{v}(\mathcal{S}) + \bar{\boldsymbol{v}}_{\boldsymbol{\tau}_s}(\mathcal{S}), \qquad \text{(S.279)}$$

which, using the identity (S.277), simplifies to

$$\boldsymbol{\tau}_r = \boldsymbol{\tau}_r + \mathbf{S}\bar{\boldsymbol{v}}_{\boldsymbol{\tau}_r}(\mathcal{S}^{-1}) + \bar{\boldsymbol{v}}_{\boldsymbol{\tau}_s}(\mathcal{S})\,. \qquad \text{(S.280)}$$

For Eq. (S.280) to hold, the following condition must be satisfied

$$\bar{\boldsymbol{v}}_{\boldsymbol{\tau}_r}(\mathcal{S}^{-1}) = -\mathbf{S}^{-1}\bar{\boldsymbol{v}}_{\mathcal{S}^{-1}\boldsymbol{\tau}_r}(\mathcal{S})\,, \qquad \text{(S.281)}$$

where we have used the relation $\boldsymbol{\tau}_s = \mathcal{S}^{-1}\boldsymbol{\tau}_r$. This expression corresponds to Eq. (S.62), completing the proof.

[7] Demonstrating the transformation (S.85) is straightforward. The function $\sqrt{\Omega_0}P^{\mathbf{Sq}}_{\mathbf{G}}(\mathbf{r}) = \exp[i(\mathbf{Sq}+\mathbf{G})\cdot\mathbf{r}]$ can be rewritten as

$$\sqrt{\Omega_0}P^{\mathbf{Sq}}_{\mathbf{G}}(\mathbf{r}) = e^{i(\mathbf{q}+\mathbf{S}^{-1}\mathbf{G})\cdot\mathbf{S}^{-1}\mathbf{r}} \qquad \text{(S.282)}$$

using the identity $\mathbf{Sq}\cdot\mathbf{r} = \mathbf{q}\cdot\mathbf{S}^{-1}\mathbf{r}$. Adding and subtracting the fractional translation $\boldsymbol{v}(\mathcal{S}^{-1})$ to $\mathbf{S}^{-1}\mathbf{r}$, we obtain

$$\sqrt{\Omega_0}P^{\mathbf{Sq}}_{\mathbf{G}}(\mathbf{r}) = e^{-i(\mathbf{q}+\mathbf{S}^{-1}\mathbf{G})\cdot\boldsymbol{v}(\mathcal{S}^{-1})}e^{i(\mathbf{q}+\mathbf{S}^{-1}\mathbf{G})\cdot\{\mathbf{S}|\boldsymbol{v}\}^{-1}\mathbf{r}}\,. \qquad \text{(S.283)}$$

Finally, using the identity (S.277), this expression can be reformulated as

$$P^{\mathbf{Sq}}_{\mathbf{G}}(\mathbf{r}) = e^{i(\mathbf{Sq}+\mathbf{G})\cdot\boldsymbol{v}(\mathcal{S})}P^{\mathbf{q}}_{\mathbf{S}^{-1}\mathbf{G}}(\{\mathbf{S}|\boldsymbol{v}\}^{-1}\mathbf{r})\,, \qquad \text{(S.284)}$$

where $\sqrt{\Omega_0}P^{\mathbf{q}}_{\mathbf{S}^{-1}\mathbf{G}}(\{\mathbf{S}|\boldsymbol{v}\}^{-1}\mathbf{r}) = \exp[i(\mathbf{q}+\mathbf{S}^{-1}\mathbf{G})\cdot\{\mathbf{S}|\boldsymbol{v}\}^{-1}\mathbf{r}]$.

In contrast, demonstrating the transformation (S.86) is more involved. We start from the Bloch-summed radial product basis function, defined in Eq. (91) in the main text, evaluated for a rotated momentum transfer $\mathbf{Sq}$

$$B^{\mathbf{Sq}}_{\boldsymbol{\tau}_r\mu L}(\mathbf{r}) = \sum_l \frac{e^{i\mathbf{Sq}\cdot\mathbf{R}_l}}{\sqrt{\Omega_0}}\times B_{\boldsymbol{\tau}_r\mu L}(\mathbf{r}-\boldsymbol{\tau}_r-\mathbf{R}_l)\theta(s_r - |\mathbf{r}-\boldsymbol{\tau}_r-\mathbf{R}_l|). \qquad \text{(S.285)}$$

Using the identity $\mathbf{Sq}\cdot\mathbf{R}_l = \mathbf{q}\cdot\mathbf{S}^{-1}\mathbf{R}_l$ and defining the new lattice reference frame $\mathbf{R}_n = \mathbf{S}^{-1}\mathbf{R}_l$, we obtain

$$B^{\mathbf{Sq}}_{\boldsymbol{\tau}_r\mu L}(\mathbf{r}) = \sum_n \frac{e^{i\mathbf{q}\cdot\mathbf{R}_n}}{\sqrt{\Omega_0}}\times B_{\boldsymbol{\tau}_r\mu L}(\mathbf{r}-\boldsymbol{\tau}_r-\mathbf{SR}_n)\theta(s_r - |\mathbf{r}-\boldsymbol{\tau}_r-\mathbf{SR}_n|). \qquad \text{(S.286)}$$

The argument of the function can then be rewritten as

$$\mathbf{r}-\boldsymbol{\tau}_r-\mathbf{SR}_n = \mathbf{S}[\mathbf{S}^{-1}\mathbf{r}-\mathbf{S}^{-1}\boldsymbol{\tau}_r-\mathbf{R}_n]\,, \qquad \text{(S.287)}$$

and adding and subtracting the fractional translation $\boldsymbol{v}(\mathcal{S}^{-1})$, we finds

$$\mathbf{r}-\boldsymbol{\tau}_r-\mathbf{SR}_n = \mathbf{S}[\{\mathbf{S}|\boldsymbol{v}\}^{-1}\mathbf{r}-\{\mathbf{S}|\boldsymbol{v}\}^{-1}\boldsymbol{\tau}_r-\mathbf{R}_n]\,. \qquad \text{(S.288)}$$

Additionally, using Eq. (S.60), we can reformulate the argument as

$$\mathbf{r}-\boldsymbol{\tau}_r-\mathbf{SR}_n = \mathbf{S}[\{\mathbf{S}|\boldsymbol{v}\}^{-1}\mathbf{r}-\mathcal{S}^{-1}\boldsymbol{\tau}_r-\mathbf{R}_p]\,, \qquad \text{(S.289)}$$

where we set $\mathbf{R}_p = \mathbf{R}_n - \bar{\boldsymbol{v}}_{\boldsymbol{\tau}_r}(\mathcal{S}^{-1}) = \mathbf{R}_n + \mathbf{S}^{-1}\bar{\boldsymbol{v}}_{\mathcal{S}^{-1}\boldsymbol{\tau}_r}(\mathcal{S})$, with $\bar{\boldsymbol{v}}_{\boldsymbol{\tau}_r}$ indicating a lattice translation vector, and where identity (S.62) has been used. The Heaviside step function can then be rewritten as

$$\theta(s_{\mathcal{S}^{-1}\boldsymbol{\tau}_r} - |\{\mathbf{S}|\boldsymbol{v}\}^{-1}\mathbf{r}-\mathcal{S}^{-1}\boldsymbol{\tau}_r-\mathbf{R}_p|)\,, \qquad \text{(S.290)}$$

since the module of the vector in Eq. (S.289) is rotationally invariant. The radial function $B_{\boldsymbol{\tau}_r\mu L}$, on the other hand, can be rewritten, by setting $\mathbf{y} = \{\mathbf{S}|\boldsymbol{v}\}\mathbf{r}-\mathcal{S}^{-1}\boldsymbol{\tau}_r-\mathbf{R}_p$, as

$$B_{\mathcal{S}^{-1}\boldsymbol{\tau}_r\mu L}(\mathbf{Sy}) = B_{\mathcal{S}^{-1}\boldsymbol{\tau}_r\mu l}(y)Y_{lm}(\mathbf{Sy}/y)\,. \qquad \text{(S.291)}$$

Finally, expressing the rotated real spherical harmonics in terms of unrotated ones via Eq. (S.87), and combining Eqs. (S.286) and (S.289)-(S.291), we arrive at Eq. (S.86), after replacing the phase factor $\exp[i\mathbf{q}\cdot\mathbf{R}_n]$ with

$$e^{-i\mathbf{Sq}\cdot\bar{\boldsymbol{v}}_{\mathcal{S}^{-1}\boldsymbol{\tau}_r}(\mathcal{S})}e^{i\mathbf{q}\cdot\mathbf{R}_p}\,, \qquad \text{(S.292)}$$

then completing the proof.

[8] Here we present the proof of Eq. (S.122). Starting from Eq. (S.103) evaluated for $l-1$, and using the identity $(2l+2n-1)!! = (2l+2n+1)!!/(2l+2n+1)$, we obtain

$$j^m_{l-1}(ar) = r^{l-1}\sum_{n=0}^{\infty}\frac{(-)^n a^{2n}r^{2n}(2l+2n+1)}{2^n n!(2l+2n+1)!!}\,. \qquad \text{(S.293)}$$

This expression can be conveniently decomposed into two terms

$$j^m_{l-1}(ar) = \frac{2l+1}{r}j^m_l(ar) + \sum_{n=1}^{\infty}\frac{(-)^n a^{2n}r^{2n}r^{l-1}}{2^{n-1}(n-1)!(2l+2n+1)!!} \qquad \text{(S.294)}$$

By setting $m = n-1$, the second term of this expression can be easily reformulated, leading to

$$j^m_{l-1}(ar) = \frac{2l+1}{r}j^m_l(ar) - a^2 j^m_{l+1}(ar)\,, \qquad \text{(S.295)}$$

from which Eq. (S.122) follow.


[9] E. T. Whittaker and G. N. Watson, *A Course Of Modern Analysis*, 5th ed. (Cambridge University Press, 2021).

[10] F. Bowman, *Inrtroduction to Bessel functions* (Dover Publications, New York, 1958).

[11] J. M. Blatt and V. Weisskopf, *Theoretical nuclear physics* (J. Wiley and Sons, NY, 1952).

[12] E. L. Hill, American Journal of Physics **22**, 211 (1954).

[13] P. M. Morse and H. Feshbach, *Methods of Theoretical Physics, Part II* (McGraw-Hill, NY, 1953).

[14] R. G. Barrera, G. A. Estevez, and J. Giraldo, European Journal of Physics **6**, 287 (1985).

[15] B. Carrascal, G. A. Estevez, P. Lee, and V. Lorenzo, European Journal of Physics **12**, 184 (1991).

[16] D. Belkić, Physica Scripta **45**, 9 (1992).
[17] N. Sanna, Computer Physics Communications **132**, 66 (2000).
[18] H. H. Homeier and E. Steinborn, Journal of Molecular Structure: THEOCHEM **368**, 31 (1996), proceedings of the Second Electronic Computational Chemistry Conference.
[19] J. J. Sakurai, *Modern Quantum Mechanics* (Addison-Wesley Publishing Company, Reading, MA, 1994).
[20] N. S. Gillis, Phys. Rev. B **1**, 1872 (1970).
[21] P. Pulay, Molecular Physics **17**, 197 (1969).
[22] S. T. Epstein, The Journal of Chemical Physics **60**, 3328 (1974).
[23] D. M. Ceperley and B. J. Alder, Phys. Rev. Lett. **45**, 566 (1980).
[24] J. P. Perdew and A. Zunger, Phys. Rev. B **23**, 5048 (1981).
[25] P. Giannozzi, S. Baroni, N. Bonini, M. Calandra, R. Car, C. Cavazzoni, D. Ceresoli, G. L. Chiarotti, M. Cococcioni, I. Dabo, A. D. Corso, S. de Gironcoli, S. Fabris, G. Fratesi, R. Gebauer, U. Gerstmann, C. Gougoussis, A. Kokalj, M. Lazzeri, L. Martin-Samos, N. Marzari, F. Mauri, R. Mazzarello, S. Paolini, A. Pasquarello, L. Paulatto, C. Sbraccia, S. Scandolo, G. Sclauzero, A. P. Seitsonen, A. Smogunov, P. Umari, and R. M. Wentzcovitch, Journal of Physics: Condensed Matter **21**, 395502 (2009).
[26] P. Giannozzi, O. Andreussi, T. Brumme, O. Bunau, M. B. Nardelli, M. Calandra, R. Car, C. Cavazzoni, D. Ceresoli, M. Cococcioni, N. Colonna, I. Carnimeo, A. D. Corso, S. de Gironcoli, P. Delugas, R. A. DiStasio, A. Ferretti, A. Floris, G. Fratesi, G. Fugallo, R. Gebauer, U. Gerstmann, F. Giustino, T. Gorni, J. Jia, M. Kawamura, H.-Y. Ko, A. Kokalj, E. Küçükbenli, M. Lazzeri, M. Marsili, N. Marzari, F. Mauri, N. L. Nguyen, H.-V. Nguyen, A. O. de-la Roza, L. Paulatto, S. Poncé, D. Rocca, R. Sabatini, B. Santra, M. Schlipf, A. P. Seitsonen, A. Smogunov, I. Timrov, T. Thonhauser, P. Umari, N. Vast, X. Wu, and S. Baroni, Journal of Physics: Condensed Matter **29**, 465901 (2017).
[27] P. Giannozzi, O. Baseggio, P. Bonfà, D. Brunato, R. Car, I. Carnimeo, C. Cavazzoni, S. de Gironcoli, P. Delugas, F. Ferrari Ruffino, A. Ferretti, N. Marzari, I. Timrov, A. Urru, and S. Baroni, The Journal of Chemical Physics **152**, 154105 (2020).
[28] S. Logothetidis, J. Petalas, H. M. Polatoglou, and D. Fuchs, Phys. Rev. B **46**, 4483 (1992).
[29] G. Antonius, S. Poncé, P. Boulanger, M. Côté, and X. Gonze, Phys. Rev. Lett. **112**, 215501 (2014).
[30] F. Karsai, M. Engel, E. Flage-Larsen, and G. Kresse, New Journal of Physics **20**, 123008 (2018).
[31] G. Venkataraman, L. A. Feldkamp, and V. C. Sahni, *Dynamics of Perfect Crystals* (The MIT Press, 1975).
